# Supplementary material for: OpenMaterial: A Large-scale Dataset of Complex Materials for 3D Reconstruction
Source: arXiv:2406.08894 source file (2025-11-02)
Supplement: Supplementary file 1 [file 7-appendix.tex]

\vspace{-7em}
\appendix

\section{Additional Qualitative Result}
Let us now present additional qualitative results, complementing those in Sec.~4.

\subsection{Ablation Dataset}
\noindent\textbf{Visual Preview.}
To illustrate the shape variety of the ablation dataset, which includes five uniquely shaped objects, we provide visualizations in \cref{fig:shape_appendix}. To give an intuition of the type of images in the ablation dataset, we showcase the `Vase' object rendered with seven material types and three lighting conditions in~\cref{fig:ablation_preview-1}.
\newcommand{\imghei}{.135\textwidth}
\begin{figure*}[htb]
    \setlength{\belowcaptionskip}{-.5cm}
    \centering
    
    \setlength{\tabcolsep}{2pt}
    \begin{minipage}{\textwidth}
    \begin{tabular}{cccccc}
        & Vase & Snail  & Boat & Motor Bike & Statue \\ % \hline
        \vspace{-5pt} \\
        \rotatebox{90}{\parbox{\imghei}{\centering RGB Image}} &
        \includegraphics[width=.18\textwidth]{img/ablation-preview/b14a251fe8ad4a10bbc75f7dd3f6cebb/gt_conductor_leadenhall_market_4k_12.png} &
        \includegraphics[width=.18\textwidth]{img/ablation-preview/fc4f34dae22c4dae95c19b1654c3cb7e/leadenhall_market_4k-conductor.png} &
        \includegraphics[width=.18\textwidth]{img/ablation-preview/01098ad7973647a9b558f41d2ebc5193/leadenhall_market_4k-conductor.png} &
        \includegraphics[width=.18\textwidth]{img/ablation-preview/df894b66e2e54b558a43497becb94ff0/leadenhall_market_4k-conductor.png} &
        \includegraphics[width=.18\textwidth]{img/ablation-preview/5c230ea126b943b8bc1da3f5865d5cd2/leadenhall_market_4k-conductor.png} \\
        
        \rotatebox{90}{\parbox{\imghei}{\centering Shape}} &
        \includegraphics[width=.18\textwidth]{img/shape-ablation/gt_b14a251fe8ad4a10bbc75f7dd3f6cebb_12.png} &
        \includegraphics[width=.18\textwidth]{img/shape-ablation/gt_fc4f34dae22c4dae95c19b1654c3cb7e_31.png} &
        \includegraphics[width=.18\textwidth]{img/shape-ablation/gt_01098ad7973647a9b558f41d2ebc5193_0.png} &
        \includegraphics[width=.18\textwidth]{img/shape-ablation/gt_df894b66e2e54b558a43497becb94ff0_1.png} &
        \includegraphics[width=.18\textwidth]{img/shape-ablation/gt_5c230ea126b943b8bc1da3f5865d5cd2_10.png} \\

    \end{tabular}
    \caption{\label{fig:shape_appendix} \textbf{Selection of objects in the ablation dataset.}}
    \end{minipage}
\end{figure*}

\noindent\textbf{3D Reconstruction.}
To enable a thorough analysis of the SOTA 3D reconstruction methods listed in Tab.~3 of the main paper, we summarize the results in~\cref{fig:neus_appendix-ablation}. We observe that the algorithms perform well on materials such as Diffuse and Plastic. However, Conductor and Dielectric materials pose greater challenges due to their complex interactions with light and matter. Notably, the specialized method NeRO substantially outperforms the general methods in the Conductor category. These visualizations validate the findings presented in Tab.~3 of the main paper, further underscoring the critical need for developing specialized algorithms capable of handling complex materials.

\vspace{.3cm}

\noindent\textbf{Novel View Synthesis.}
To enable an in-depth analysis of the SOTA novel view synthesis methods listed in the Tab.~3 of the main paper, we summarize the results in~\cref{fig:nerf_appendix-ablation-1}. All algorithms perform well on Diffuse and Plastic materials. It is important to note that, despite the lighting and shape of the object remaining the same, the appearance of the object in the image changes significantly due to variations in material type. This introduces greater challenges for Conductor and Dielectric materials compared to Plastic and Diffuse.
As illustrated in \cref{fig:nerf_appendix-ablation-1}, the blurred reflection patterns observed on Conductor materials are noticeable. These patterns arise as the methods interpret the intricate interactions between light and matter, leaving room for further refinement in their interpretation.
In the Dielectric category, methods such as 3DGS, PGSR, 2DGS, GES, and GaussianShader generate distorted patterns and illusory black spots on the body of the 'Vase'. This occurs because these methods struggle to accurately capture the complex refraction and reflection properties inherent in these materials.
These results confirm the findings in Tab.~3 of the main paper, underscoring the need to develop specialized algorithms for complex material interactions.

\begin{figure*}[htp]
    \setlength{\belowcaptionskip}{-5pt}
    
    \setlength{\tabcolsep}{10pt}
    \vspace{-0.5cm}
    \hspace{1.cm}
    
    \begin{minipage}{\textwidth}
    \begin{tabular}{cccc}
    \centering
        & Indoor Scene & Daytime Garden  & Nighttime Street  \\ % \hline
    % \vspace{-5pt} \\
    \rotatebox{90}{\parbox{\imghe}{\centering Conductor}} &
    \includegraphics[width=.24\textwidth]{img/ablation-preview/b14a251fe8ad4a10bbc75f7dd3f6cebb/gt_conductor_leadenhall_market_4k_12.png} &
    \includegraphics[width=.24\textwidth]{img/ablation-preview/b14a251fe8ad4a10bbc75f7dd3f6cebb/gt_conductor_symmetrical_garden_4k_12.png} &
    \includegraphics[width=.24\textwidth]{img/ablation-preview/b14a251fe8ad4a10bbc75f7dd3f6cebb/gt_conductor_cobblestone_street_night_4k_12.png} \\
    
    \rotatebox{90}{\parbox{\imghe}{\centering RoughConductor}} &
    \includegraphics[width=.24\textwidth]{img/ablation-preview/b14a251fe8ad4a10bbc75f7dd3f6cebb/gt_roughconductor_leadenhall_market_4k_12.png} &
    \includegraphics[width=.24\textwidth]{img/ablation-preview/b14a251fe8ad4a10bbc75f7dd3f6cebb/gt_roughconductor_symmetrical_garden_4k_12.png} &
    \includegraphics[width=.24\textwidth]{img/ablation-preview/b14a251fe8ad4a10bbc75f7dd3f6cebb/gt_roughconductor_cobblestone_street_night_4k_12.png} \\
    
    \rotatebox{90}{\parbox{\imghe}{\centering Dielectric}} &
    \includegraphics[width=.24\textwidth]{img/ablation-preview/b14a251fe8ad4a10bbc75f7dd3f6cebb/gt_dielectric_leadenhall_market_4k_12.png} &
    \includegraphics[width=.24\textwidth]{img/ablation-preview/b14a251fe8ad4a10bbc75f7dd3f6cebb/gt_dielectric_symmetrical_garden_4k_12.png} &
    \includegraphics[width=.24\textwidth]{img/ablation-preview/b14a251fe8ad4a10bbc75f7dd3f6cebb/gt_dielectric_cobblestone_street_night_4k_12.png} \\
    
    \rotatebox{90}{\parbox{\imghe}{\centering RoughDielectric}} &
    \includegraphics[width=.24\textwidth]{img/ablation-preview/b14a251fe8ad4a10bbc75f7dd3f6cebb/gt_roughdielectric_leadenhall_market_4k_12.png} &
    \includegraphics[width=.24\textwidth]{img/ablation-preview/b14a251fe8ad4a10bbc75f7dd3f6cebb/gt_roughdielectric_symmetrical_garden_4k_12.png} &
    \includegraphics[width=.24\textwidth]{img/ablation-preview/b14a251fe8ad4a10bbc75f7dd3f6cebb/gt_roughdielectric_cobblestone_street_night_4k_12.png} \\
    
    \rotatebox{90}{\parbox{\imghe}{\centering Plastic}} &
    \includegraphics[width=.24\textwidth]{img/ablation-preview/b14a251fe8ad4a10bbc75f7dd3f6cebb/gt_plastic_leadenhall_market_4k_12.png} &
    \includegraphics[width=.24\textwidth]{img/ablation-preview/b14a251fe8ad4a10bbc75f7dd3f6cebb/gt_plastic_symmetrical_garden_4k_12.png} &
    \includegraphics[width=.24\textwidth]{img/ablation-preview/b14a251fe8ad4a10bbc75f7dd3f6cebb/gt_plastic_cobblestone_street_night_4k_12.png} \\
    
    \rotatebox{90}{\parbox{\imghe}{\centering RoughPlastic}} &
    \includegraphics[width=.24\textwidth]{img/ablation-preview/b14a251fe8ad4a10bbc75f7dd3f6cebb/gt_roughplastic_leadenhall_market_4k_12.png} &
    \includegraphics[width=.24\textwidth]{img/ablation-preview/b14a251fe8ad4a10bbc75f7dd3f6cebb/gt_roughplastic_symmetrical_garden_4k_12.png} &
    \includegraphics[width=.24\textwidth]{img/ablation-preview/b14a251fe8ad4a10bbc75f7dd3f6cebb/gt_roughplastic_cobblestone_street_night_4k_12.png} \\
    
    \rotatebox{90}{\parbox{\imghe}{\centering Diffuse}} &
    \includegraphics[width=.24\textwidth]{img/ablation-preview/b14a251fe8ad4a10bbc75f7dd3f6cebb/gt_diffuse_leadenhall_market_4k_12.png} &
    \includegraphics[width=.24\textwidth]{img/ablation-preview/b14a251fe8ad4a10bbc75f7dd3f6cebb/gt_diffuse_symmetrical_garden_4k_12.png} &
    \includegraphics[width=.24\textwidth]{img/ablation-preview/b14a251fe8ad4a10bbc75f7dd3f6cebb/gt_diffuse_cobblestone_street_night_4k_12.png} \\
    
    \end{tabular}
    \end{minipage}
    \caption{\textbf{Previews of the 'Vase' in the ablation dataset.}}
    \label{fig:ablation_preview-1}
\end{figure*}

\begin{figure*}[htp]
    \setlength{\belowcaptionskip}{-.5cm}
    \centering
    
    \setlength{\tabcolsep}{2pt}
    \begin{minipage}{\textwidth}
    \begin{tabular}{ccccc}
        & Conductor & Dielectric  & Plastic & Diffuse  \\ % \hline
        \vspace{-5pt} \\
        \rotatebox{90}{\parbox{\imghe}{\centering RGB Image}} &
        \includegraphics[width=.24\textwidth]{img/ablation_neus_2/gt_conductor_symmetrical_garden_4k_10.png} &
        \includegraphics[width=.24\textwidth]{img/ablation_neus_2/gt_dielectric_symmetrical_garden_4k_10.png} &
        \includegraphics[width=.24\textwidth]{img/ablation_neus_2/gt_plastic_symmetrical_garden_4k_10.png} &
        \includegraphics[width=.24\textwidth]{img/ablation_neus_2/gt_diffuse_symmetrical_garden_4k_10.png} \\
        % PGSR_5c230ea126b943b8bc1da3f5865d5cd2_symmetrical_garden_4k_roughplastic_10.png
        \rotatebox{90}{\parbox{\imghe}{\centering PGSR}} &
        \includegraphics[width=.24\textwidth]{img/ablation_neus_2/PGSR_5c230ea126b943b8bc1da3f5865d5cd2_symmetrical_garden_4k_conductor_10.png} &
        \includegraphics[width=.24\textwidth]{img/ablation_neus_2/PGSR_5c230ea126b943b8bc1da3f5865d5cd2_symmetrical_garden_4k_dielectric_10.png} &
        \includegraphics[width=.24\textwidth]{img/ablation_neus_2/PGSR_5c230ea126b943b8bc1da3f5865d5cd2_symmetrical_garden_4k_plastic_10.png} &
        \includegraphics[width=.24\textwidth]{img/ablation_neus_2/PGSR_5c230ea126b943b8bc1da3f5865d5cd2_symmetrical_garden_4k_diffuse_10.png} \\

        \rotatebox{90}{\parbox{\imghe}{\centering NeRO}} &
        \includegraphics[width=.24\textwidth]{img/ablation_neus_2/NeRO_5c230ea126b943b8bc1da3f5865d5cd2_symmetrical_garden_4k_conductor_10.png} &
        \includegraphics[width=.24\textwidth]{img/ablation_neus_2/NeRO_5c230ea126b943b8bc1da3f5865d5cd2_symmetrical_garden_4k_dielectric_10.png} &
        \includegraphics[width=.24\textwidth]{img/ablation_neus_2/NeRO_5c230ea126b943b8bc1da3f5865d5cd2_symmetrical_garden_4k_plastic_10.png} &
        \includegraphics[width=.24\textwidth]{img/ablation_neus_2/NeRO_5c230ea126b943b8bc1da3f5865d5cd2_symmetrical_garden_4k_diffuse_10.png} \\
        
        \rotatebox{90}{\parbox{\imghe}{\centering 2DGS}} &
        \includegraphics[width=.24\textwidth]{img/ablation_neus_2/2dgs_5c230ea126b943b8bc1da3f5865d5cd2_symmetrical_garden_4k_conductor_10.png} &
        \includegraphics[width=.24\textwidth]{img/ablation_neus_2/2dgs_5c230ea126b943b8bc1da3f5865d5cd2_symmetrical_garden_4k_dielectric_10.png} &
        \includegraphics[width=.24\textwidth]{img/ablation_neus_2/2dgs_5c230ea126b943b8bc1da3f5865d5cd2_symmetrical_garden_4k_plastic_10.png} &
        \includegraphics[width=.24\textwidth]{img/ablation_neus_2/2dgs_5c230ea126b943b8bc1da3f5865d5cd2_symmetrical_garden_4k_diffuse_10.png} \\
        
        \rotatebox{90}{\parbox{\imghe}{\centering Instant-NeuS}} &
        \includegraphics[width=.24\textwidth]{img/ablation_neus_2/instant-nsr-pl-wmask_5c230ea126b943b8bc1da3f5865d5cd2_symmetrical_garden_4k_conductor_10.png} &
        \includegraphics[width=.24\textwidth]{img/ablation_neus_2/instant-nsr-pl-wmask_5c230ea126b943b8bc1da3f5865d5cd2_symmetrical_garden_4k_dielectric_10.png} &
        \includegraphics[width=.24\textwidth]{img/ablation_neus_2/instant-nsr-pl-wmask_5c230ea126b943b8bc1da3f5865d5cd2_symmetrical_garden_4k_plastic_10.png} &
        \includegraphics[width=.24\textwidth]{img/ablation_neus_2/instant-nsr-pl-wmask_5c230ea126b943b8bc1da3f5865d5cd2_symmetrical_garden_4k_diffuse_10.png} \\
        
        \rotatebox{90}{\parbox{\imghe}{\centering NeuS2}} &
        \includegraphics[width=.24\textwidth]{img/ablation_neus_2/neus2_5c230ea126b943b8bc1da3f5865d5cd2_symmetrical_garden_4k_conductor_10.png} &
        \includegraphics[width=.24\textwidth]{img/ablation_neus_2/neus2_5c230ea126b943b8bc1da3f5865d5cd2_symmetrical_garden_4k_dielectric_10.png} &
        \includegraphics[width=.24\textwidth]{img/ablation_neus_2/neus2_5c230ea126b943b8bc1da3f5865d5cd2_symmetrical_garden_4k_plastic_10.png} &
        \includegraphics[width=.24\textwidth]{img/ablation_neus_2/neus2_5c230ea126b943b8bc1da3f5865d5cd2_symmetrical_garden_4k_diffuse_10.png} \\
        
    \end{tabular}
    \caption{\label{fig:neus_appendix-ablation} \textbf{Additional qualitative 3D reconstruction results on the ablation dataset.}}
    \end{minipage}
\end{figure*}
\begin{figure*}[htp]
    \setlength{\belowcaptionskip}{-.5cm}
    \centering
    
    \setlength{\tabcolsep}{2pt}
    \begin{minipage}{\textwidth}
    \begin{tabular}{ccccc}
        & Conductor & Dielectric  & Plastic & Diffuse  \\ % \hline
        \vspace{-5pt} \\
        \rotatebox{90}{\parbox{\imghe}{\centering Ground Truth}} &
        \includegraphics[width=.24\textwidth]{img/ablation_nerf/b14a251fe8ad4a10bbc75f7dd3f6cebb/gt_conductor_leadenhall_market_4k_12.png} &
        \includegraphics[width=.24\textwidth]{img/ablation_nerf/b14a251fe8ad4a10bbc75f7dd3f6cebb/gt_dielectric_leadenhall_market_4k_12.png} &
        \includegraphics[width=.24\textwidth]{img/ablation_nerf/b14a251fe8ad4a10bbc75f7dd3f6cebb/gt_plastic_leadenhall_market_4k_12.png} &
        \includegraphics[width=.24\textwidth]{img/ablation_nerf/b14a251fe8ad4a10bbc75f7dd3f6cebb/gt_diffuse_leadenhall_market_4k_12.png} \\
        
        \rotatebox{90}{\parbox{\imghe}{\centering 3DGS}} &
        \includegraphics[width=.24\textwidth]{img/ablation_nerf/b14a251fe8ad4a10bbc75f7dd3f6cebb/gaussian_model_conductor_leadenhall_market_4k_12.png} &
        \includegraphics[width=.24\textwidth]{img/ablation_nerf/b14a251fe8ad4a10bbc75f7dd3f6cebb/gaussian_model_dielectric_leadenhall_market_4k_12.png} &
        \includegraphics[width=.24\textwidth]{img/ablation_nerf/b14a251fe8ad4a10bbc75f7dd3f6cebb/gaussian_model_plastic_leadenhall_market_4k_12.png} &
        \includegraphics[width=.24\textwidth]{img/ablation_nerf/b14a251fe8ad4a10bbc75f7dd3f6cebb/gaussian_model_diffuse_leadenhall_market_4k_12.png} \\

        \rotatebox{90}{\parbox{\imghe}{\centering Instant-NGP}} &
        \includegraphics[width=.24\textwidth]{img/ablation_nerf/b14a251fe8ad4a10bbc75f7dd3f6cebb/insr_conductor_leadenhall_market_4k_12.png} &
        \includegraphics[width=.24\textwidth]{img/ablation_nerf/b14a251fe8ad4a10bbc75f7dd3f6cebb/insr_dielectric_leadenhall_market_4k_12.png} &
        \includegraphics[width=.24\textwidth]{img/ablation_nerf/b14a251fe8ad4a10bbc75f7dd3f6cebb/insr_plastic_leadenhall_market_4k_12.png} &
        \includegraphics[width=.24\textwidth]{img/ablation_nerf/b14a251fe8ad4a10bbc75f7dd3f6cebb/insr_diffuse_leadenhall_market_4k_12.png} \\
        
        \rotatebox{90}{\parbox{\imghe}{\centering PGSR}} &
        \includegraphics[width=.24\textwidth]{img/ablation_nerf/b14a251fe8ad4a10bbc75f7dd3f6cebb/PGSR_conductor_leadenhall_market_4k_12.png} &
        \includegraphics[width=.24\textwidth]{img/ablation_nerf/b14a251fe8ad4a10bbc75f7dd3f6cebb/PGSR_dielectric_leadenhall_market_4k_12.png} &
        \includegraphics[width=.24\textwidth]{img/ablation_nerf/b14a251fe8ad4a10bbc75f7dd3f6cebb/PGSR_plastic_leadenhall_market_4k_12.png} &
        \includegraphics[width=.24\textwidth]{img/ablation_nerf/b14a251fe8ad4a10bbc75f7dd3f6cebb/PGSR_diffuse_leadenhall_market_4k_12.png} \\

        \rotatebox{90}{\parbox{\imghe}{\centering 2DGS}} &
        \includegraphics[width=.24\textwidth]{img/ablation_nerf/b14a251fe8ad4a10bbc75f7dd3f6cebb/2dgs_conductor_leadenhall_market_4k_12.png} &
        \includegraphics[width=.24\textwidth]{img/ablation_nerf/b14a251fe8ad4a10bbc75f7dd3f6cebb/2dgs_dielectric_leadenhall_market_4k_12.png} &
        \includegraphics[width=.24\textwidth]{img/ablation_nerf/b14a251fe8ad4a10bbc75f7dd3f6cebb/2dgs_plastic_leadenhall_market_4k_12.png} &
        \includegraphics[width=.24\textwidth]{img/ablation_nerf/b14a251fe8ad4a10bbc75f7dd3f6cebb/2dgs_diffuse_leadenhall_market_4k_12.png} \\

        \rotatebox{90}{\parbox{\imghe}{\centering GaussianShader}} &
        \includegraphics[width=.24\textwidth]{img/ablation_nerf/b14a251fe8ad4a10bbc75f7dd3f6cebb/GaussianShader_conductor_leadenhall_market_4k_12.png} &
        \includegraphics[width=.24\textwidth]{img/ablation_nerf/b14a251fe8ad4a10bbc75f7dd3f6cebb/GaussianShader_dielectric_leadenhall_market_4k_12.png} &
        \includegraphics[width=.24\textwidth]{img/ablation_nerf/b14a251fe8ad4a10bbc75f7dd3f6cebb/GaussianShader_plastic_leadenhall_market_4k_12.png} &
        \includegraphics[width=.24\textwidth]{img/ablation_nerf/b14a251fe8ad4a10bbc75f7dd3f6cebb/GaussianShader_diffuse_leadenhall_market_4k_12.png} \\

        \rotatebox{90}{\parbox{\imghe}{\centering GES}} &
        \includegraphics[width=.24\textwidth]{img/ablation_nerf/b14a251fe8ad4a10bbc75f7dd3f6cebb/ges_conductor_leadenhall_market_4k_12.png} &
        \includegraphics[width=.24\textwidth]{img/ablation_nerf/b14a251fe8ad4a10bbc75f7dd3f6cebb/ges_dielectric_leadenhall_market_4k_12.png} &
        \includegraphics[width=.24\textwidth]{img/ablation_nerf/b14a251fe8ad4a10bbc75f7dd3f6cebb/ges_plastic_leadenhall_market_4k_12.png} &
        \includegraphics[width=.24\textwidth]{img/ablation_nerf/b14a251fe8ad4a10bbc75f7dd3f6cebb/ges_diffuse_leadenhall_market_4k_12.png} \\
        
        \rotatebox{90}{\parbox{\imghe}{\centering GSDR}} &
        \includegraphics[width=.24\textwidth]{img/ablation_nerf/b14a251fe8ad4a10bbc75f7dd3f6cebb/gsdr_conductor_leadenhall_market_4k_12.png} &
        \includegraphics[width=.24\textwidth]{img/ablation_nerf/b14a251fe8ad4a10bbc75f7dd3f6cebb/gsdr_dielectric_leadenhall_market_4k_12.png} &
        \includegraphics[width=.24\textwidth]{img/ablation_nerf/b14a251fe8ad4a10bbc75f7dd3f6cebb/gsdr_plastic_leadenhall_market_4k_12.png} &
        \includegraphics[width=.24\textwidth]{img/ablation_nerf/b14a251fe8ad4a10bbc75f7dd3f6cebb/gsdr_diffuse_leadenhall_market_4k_12.png} \\
        
    \end{tabular}
    \caption{\label{fig:nerf_appendix-ablation-1} \textbf{Additional qualitative 3D reconstruction results on the ablation dataset.}}
    \end{minipage}
\end{figure*}
\FloatBarrier

\subsection{Additional Ablation Study}

\noindent\textbf{Ablation study of the lighting condition.}
In this experiment, we keep the shape and material types constant, and only adjust the lighting conditions.
In both 3D reconstruction and novel view synthesis, material properties have a more substantial impact on performance than lighting conditions. Regarding lighting, the difference in camera exposure between multi-view images appears to have a greater impact on the 3D reconstruction task. As evidence, the PGSR algorithm performs best in 3D reconstruction across all lighting conditions, suggesting that its camera exposure compensation strategy is effective.

\begin{table}[htb]  
\centering  
\scriptsize  
\caption{\label{tab:ablation_light}\textbf{Ablation of Lighting Condition.}}  
\setlength{\tabcolsep}{20pt}  
\begin{tabular}{p{1.2cm}|c|ccc}  
\toprule  
\multirow{2}{*}{Metric} & \multirow{2}{*}{Method} & \multicolumn{3}{c}{\textbf{Lighting Type}} \\  
                       &                         & street night & market hall & garden \\  
\midrule

\multirow{5}{*}{\parbox{1.2cm}{\centering Chamfer Distance$\downarrow$}}
                        & 2DGS~\cite{Huang24}             & \num{1.4259}                          & \num{1.3740}                         & \num{1.3371} \\
                        & Instant-NeuS~\cite{Guo22}              & \cellcolor{top3}\num{1.03488}          & \num{1.099435}                         & \num{1.106376}\\
                        & NeuS2~\cite{Wang23a}                     & \cellcolor{top2}\num{0.9680}          & \cellcolor{top3}\num{1.0118}         & \cellcolor{top3}\num{1.0299}\\
                        & PGSR~\cite{Chen24}                      & \cellcolor{top1}\num{0.8455}          & \cellcolor{top1}\num{0.9160}         & \cellcolor{top1}\num{0.8487}\\
                        & NeRO$\star$~\cite{Liu23b}                      & \num{1.0614}                          & \cellcolor{top2}\num{0.9669}         & \cellcolor{top2}\num{1.0003}\\
                        % & NeRRF$\star$ & 0.9062            & 0.9020            & 0.8916 \\
\midrule  
\multirow{7}{*}{\parbox{1.2cm}{\centering PSNR$\uparrow$}}         
                       & Gaussian Splatting~\cite{Kerbl23}          & \num{29.353405}        & \num{29.170987}           & \num{29.077644} \\
                       & InstantNGP~\cite{Muller22}  & \cellcolor{top2}\num{29.810709} & \num{28.92153} & \cellcolor{top3}\num{29.598134} \\
                       & 2DGS~\cite{Huang24}                    & \num{29.465541}        &    \num{28.803827}         &    \num{28.718458} \\
                       & PGSR~\cite{Chen24}                    & \cellcolor{top1}\num{29.841052}            &\cellcolor{top2}\num{29.491238}             &\cellcolor{top2}\num{29.660042}\\
                       & GES~\cite{Hamdi24}                     & \num{29.460795} & \cellcolor{top3}\num{29.292089} & \num{29.186757} \\
                       & GSDR$\star$~\cite{Ye24}        & \cellcolor{top3}\num{29.751078}        &    \cellcolor{top1}\num{29.749379}         &    \cellcolor{top1}\num{30.460075} \\  
                       & GaussianShader$\star$~\cite{Jiang23} & \num{21.306568} & \num{21.947638} & \num{22.570275} \\
                       
\bottomrule
\end{tabular}
\end{table}
%%%%%%%%%%%%%%%%%%%%%%%%%%%%%%%%%%%%%%%%%%%%%%%%%%%%%%%%%%%%%%%%%%%%%%%%%%%%%%%%%

\section{OpenMaterial Dataset}

\noindent\textbf{3D Reconstruction.}
To facilitate a deeper analysis of all the algorithms presented in the task of 3D reconstruction, we provide additional visualizations beyond the two methods, PGSR and NeRO, presented in the main paper. These visualizations, summarized in~\cref{fig:neus_appendix-1}, include all the methods listed in Tab.~1 in the main paper. 
All methods demonstrate effective performance on Diffuse and Plastic materials. However, for the more challenging Conductor material, the specially designed methods NeRO and NeRRF yield better results than the general-purpose methods. Specifically, these methods tend to produce objects with fewer holes, as observed in the car's body section. 
Building on this improvement, the outcomes demonstrate a smoother appearance, but there is potential to further enhance the preservation of finer details.
This highlights the critical need for the development of algorithms that are tailored to manage complex materials more effectively.

\vspace{.3cm}

\noindent\textbf{Novel View Synthesis.}
To facilitate a more thorough inspection of algorithm performance across various material types, we provide additional visualizations beyond the Conductor material type presented in the main paper. These additional visualizations, which include Dielectric, Plastic, and Diffuse materials, are detailed in~\cref{fig:nerf_appendix}.
Specifically for the Dielectric material, as demonstrated with a chess piece, the background texture should appear by transparency, but both methods PGSR and InstantNGP yield textures that are jumbled due to the color viewpoint dependency caused by transmission. Moreover, the sharp highlights due to reflections at the base are to some degree captured by PGSR, whereas Instant-NGP fails to reconstruct these features.

\begin{figure*}[htb]
    \setlength{\belowcaptionskip}{-.5cm}
    \centering
    
    \setlength{\tabcolsep}{2pt}
    \begin{minipage}{\textwidth}
    \begin{tabular}{ccccc}
        & Conductor & Dielectric  & Plastic & Diffuse  \\ % \hline
        \vspace{-5pt} \\
        \rotatebox{90}{\parbox{\imghe}{\centering RGB Image}} &
        \includegraphics[width=.24\textwidth]{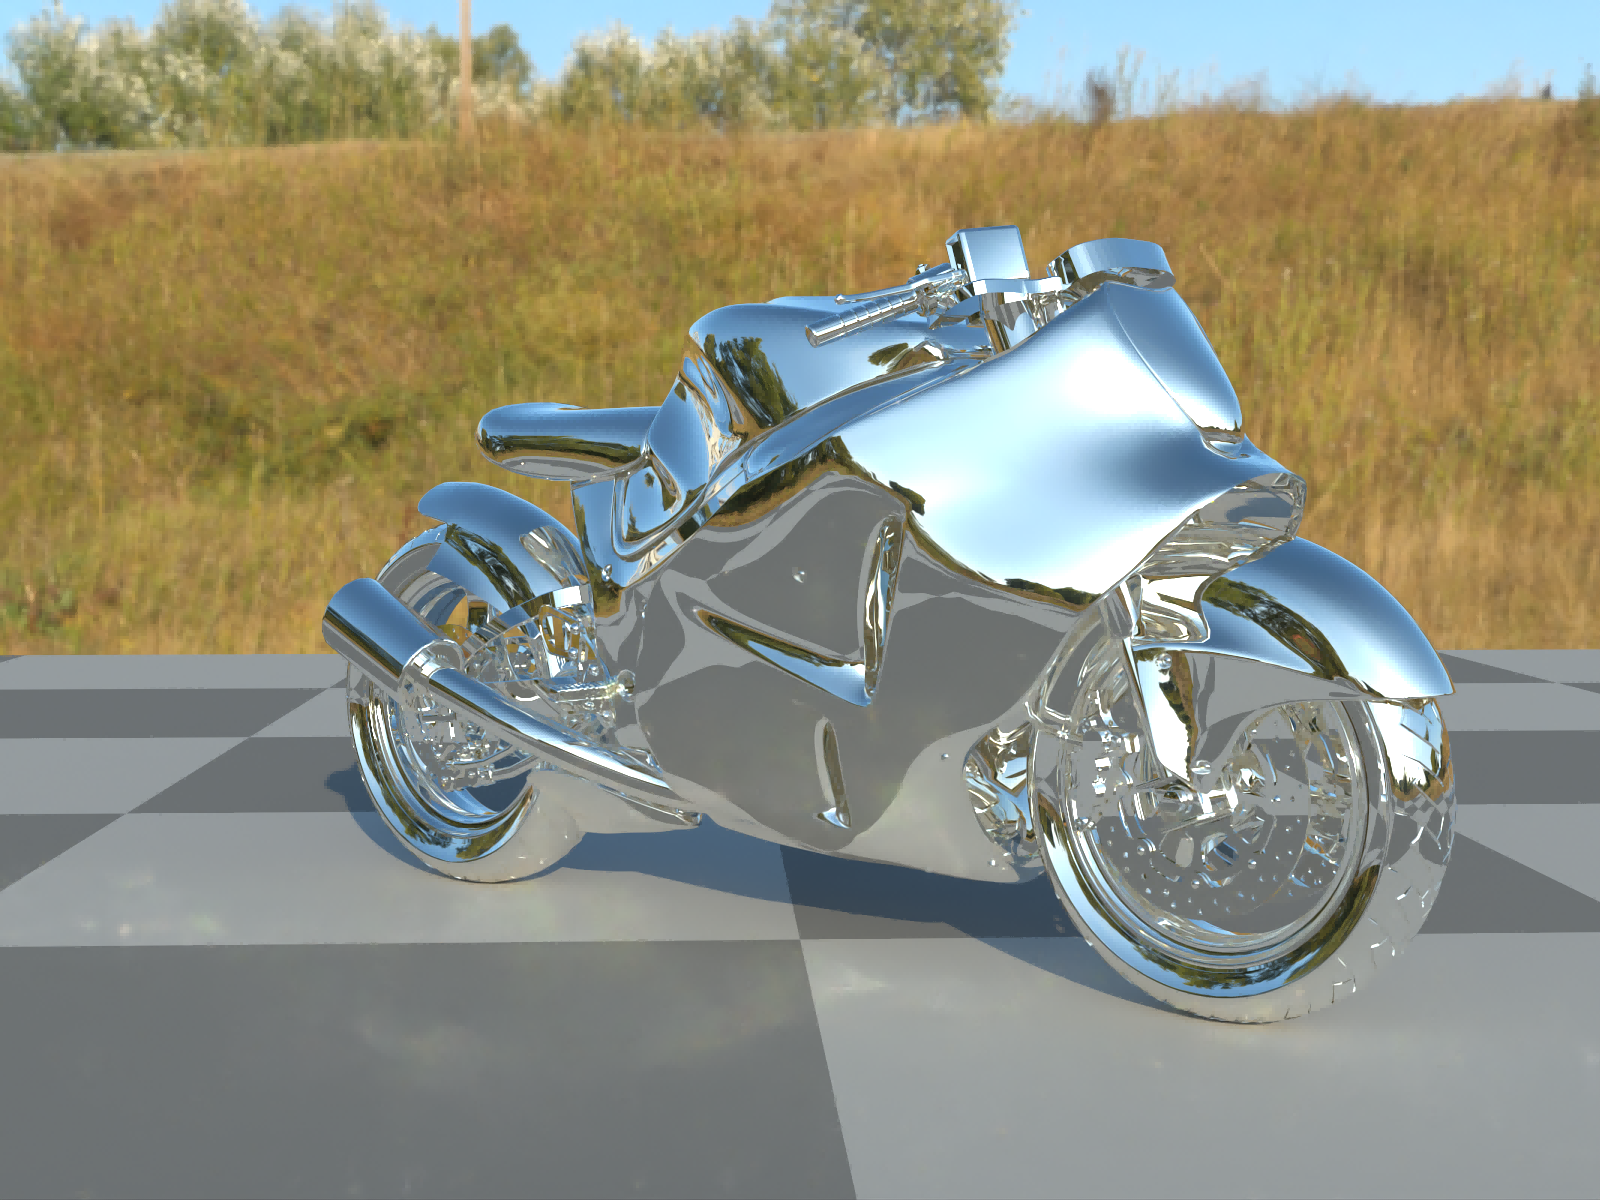} &
        \includegraphics[width=.24\textwidth]{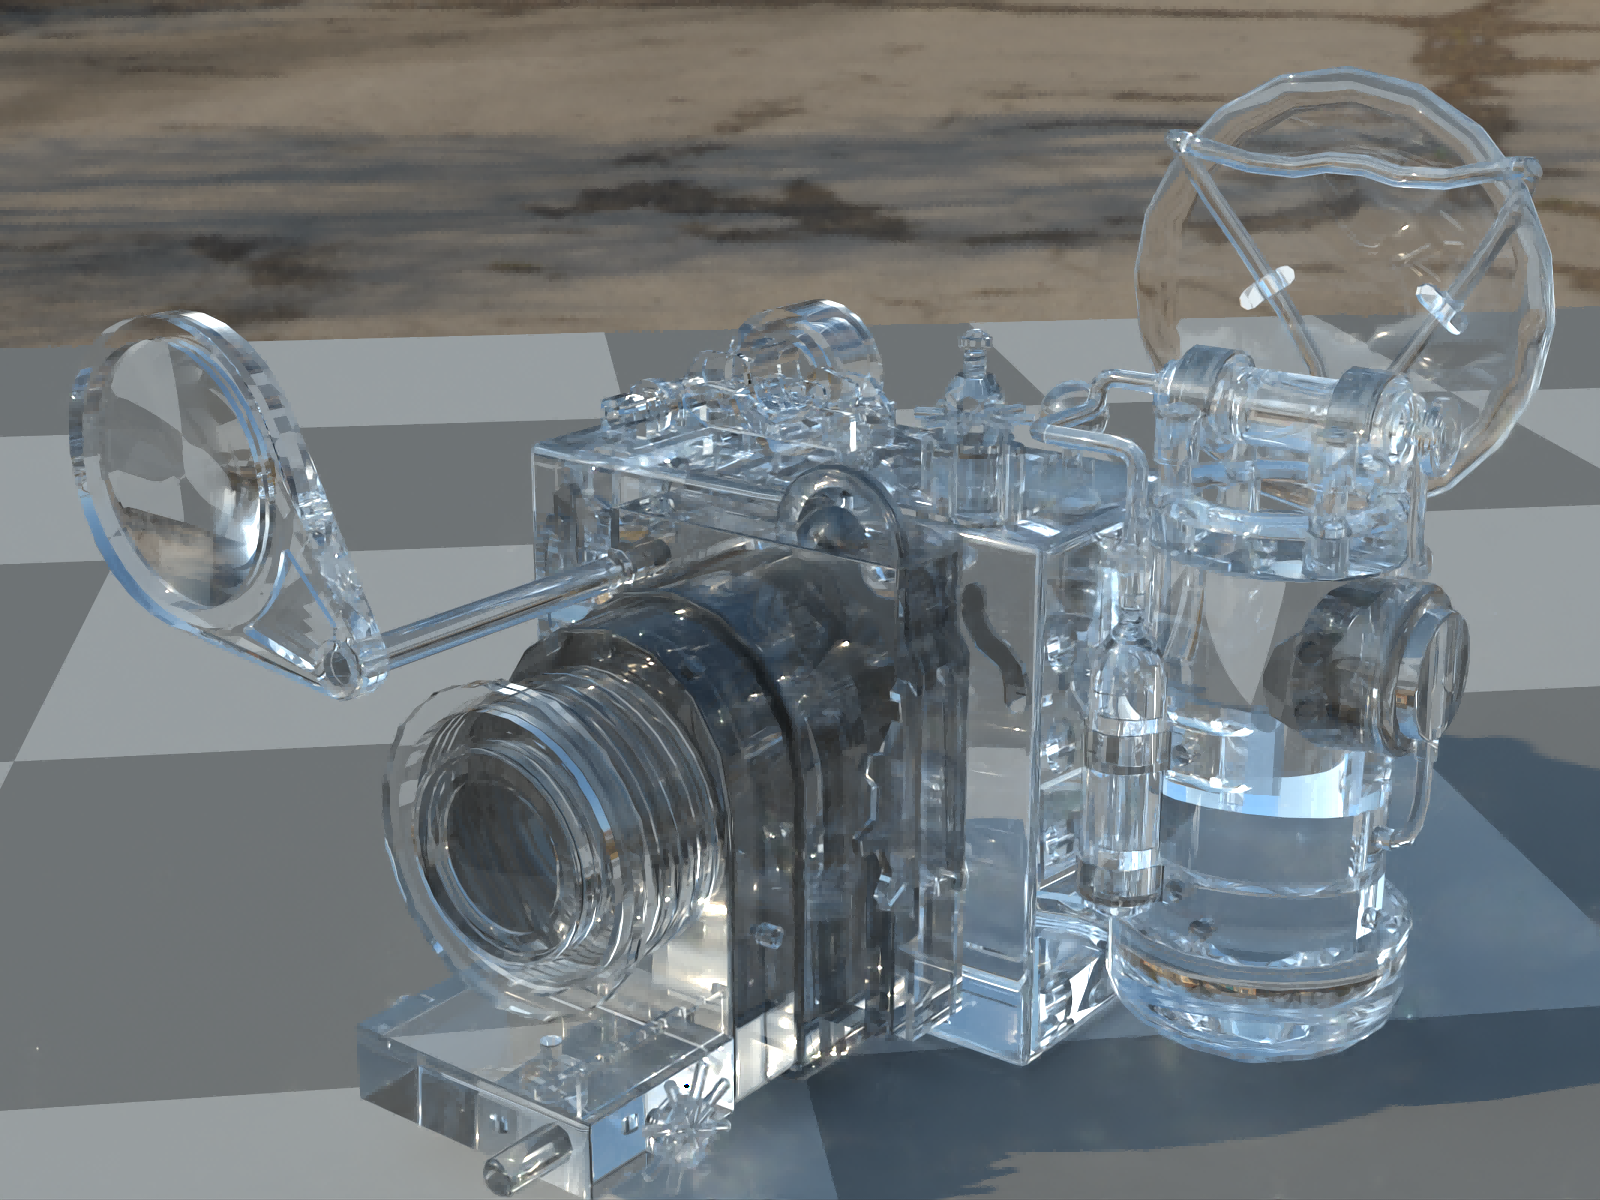} &
        \includegraphics[width=.24\textwidth]{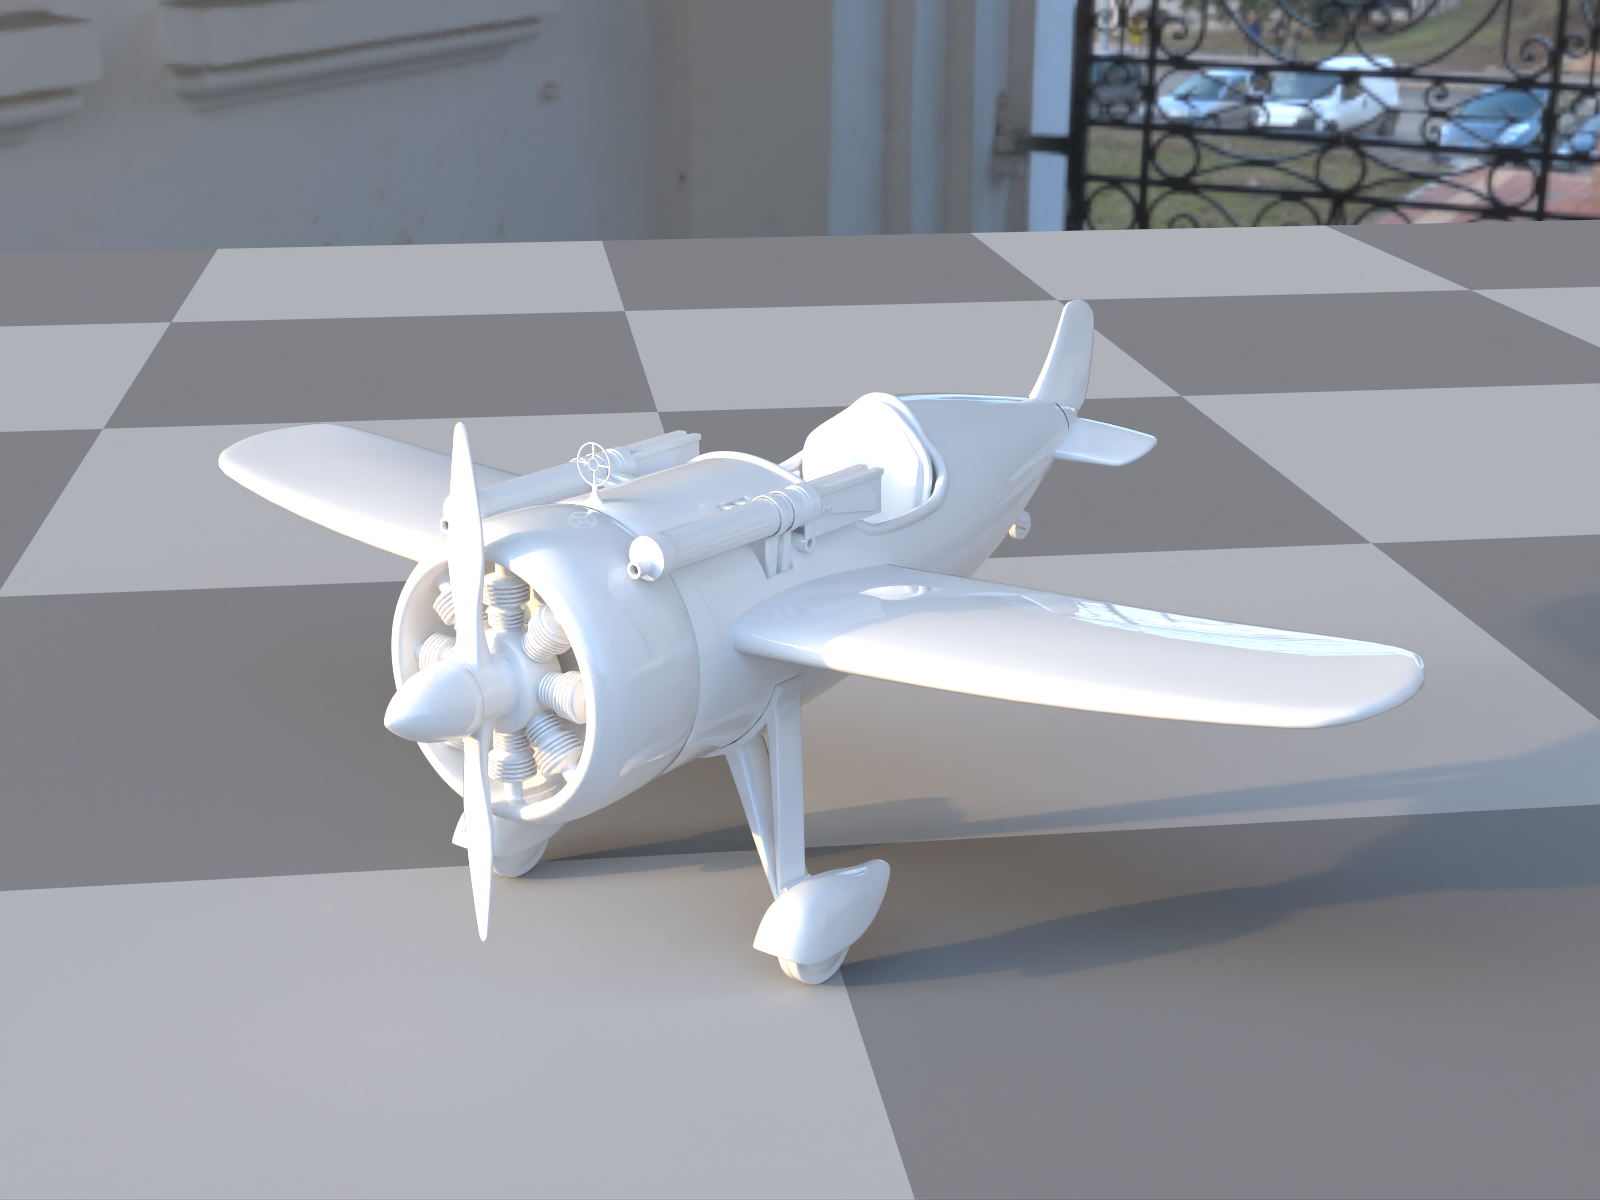} &
        \includegraphics[width=.24\textwidth]{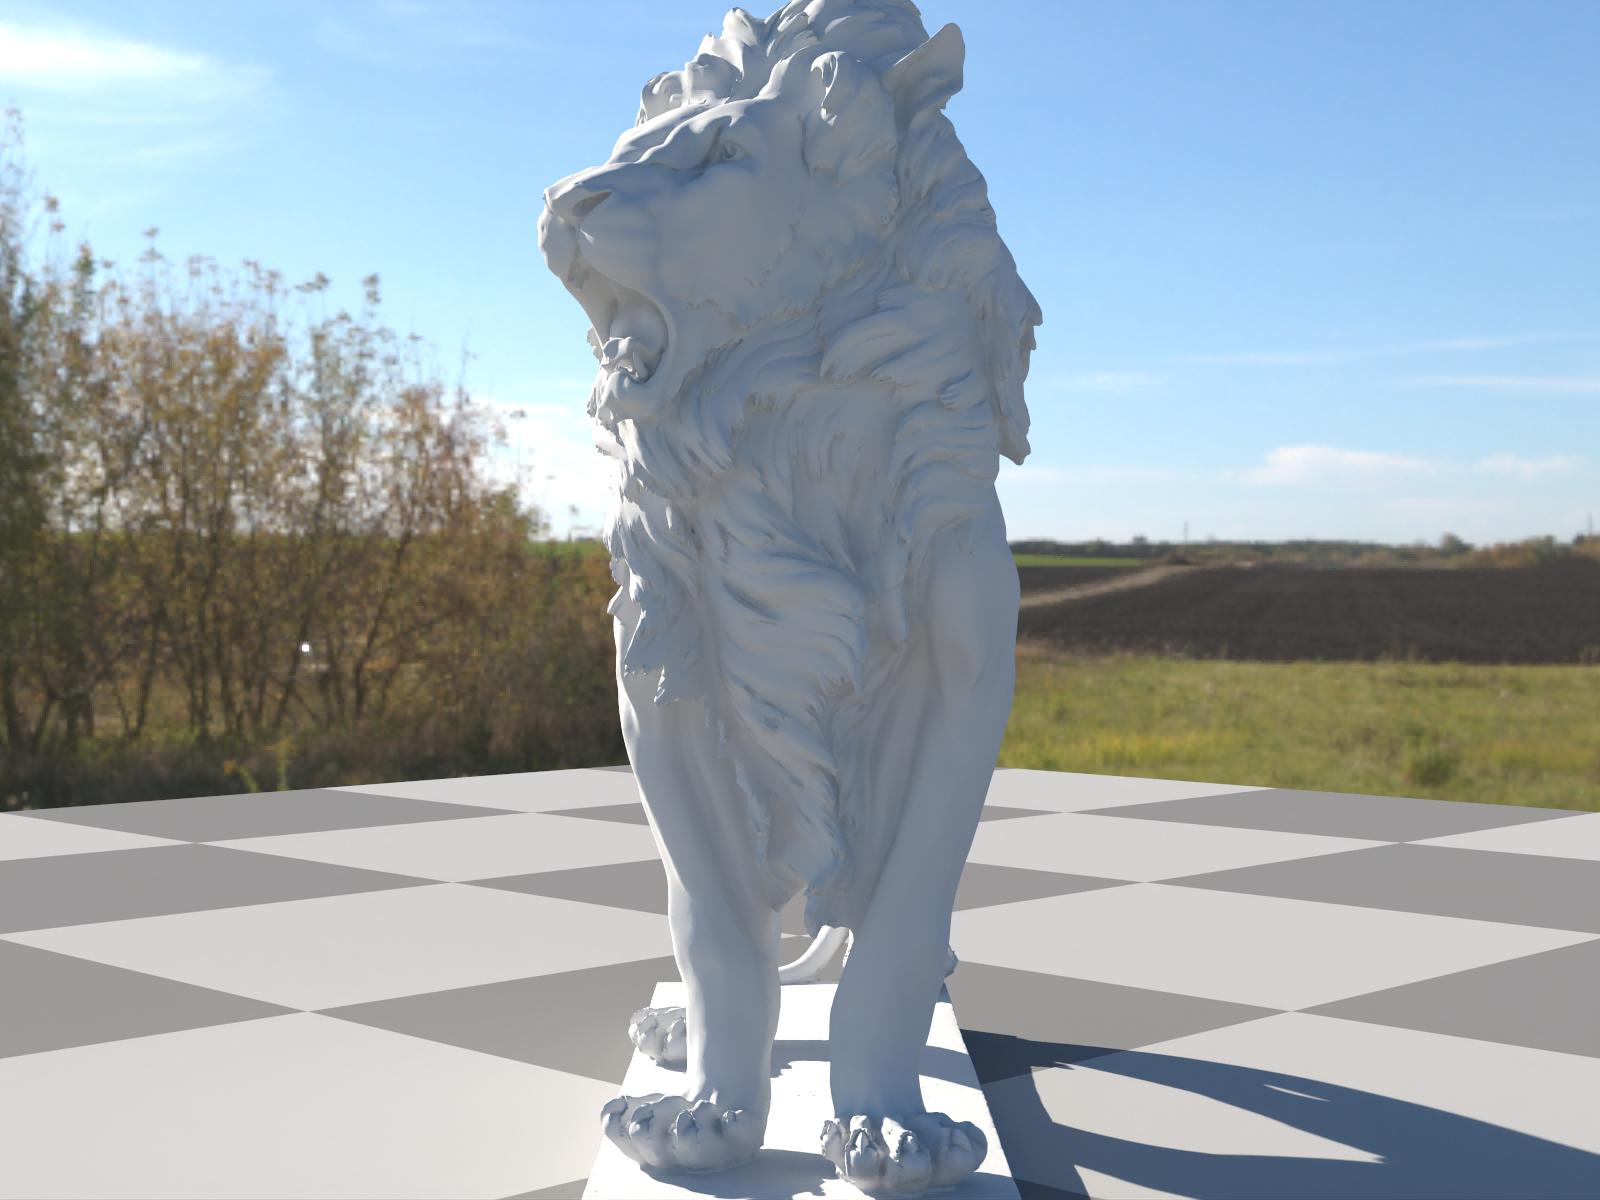} \\
        
        \rotatebox{90}{\parbox{\imghe}{\centering Ground Truth}} &
        \includegraphics[width=.24\textwidth]{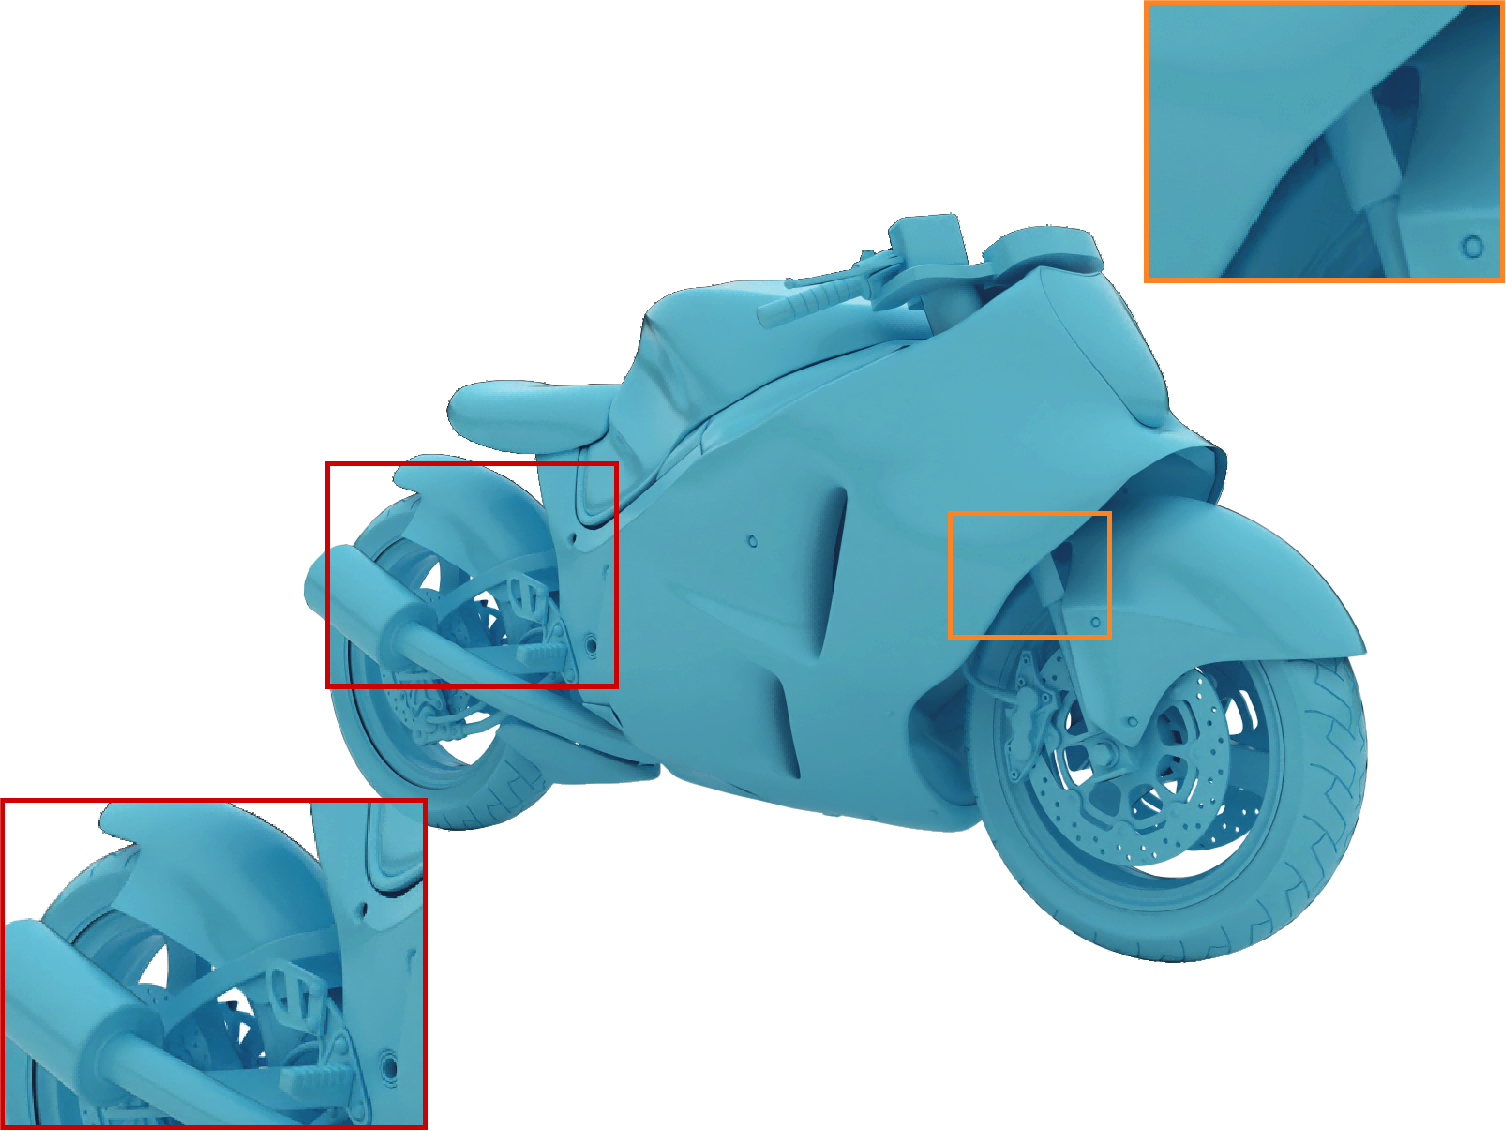} &
        \includegraphics[width=.24\textwidth]{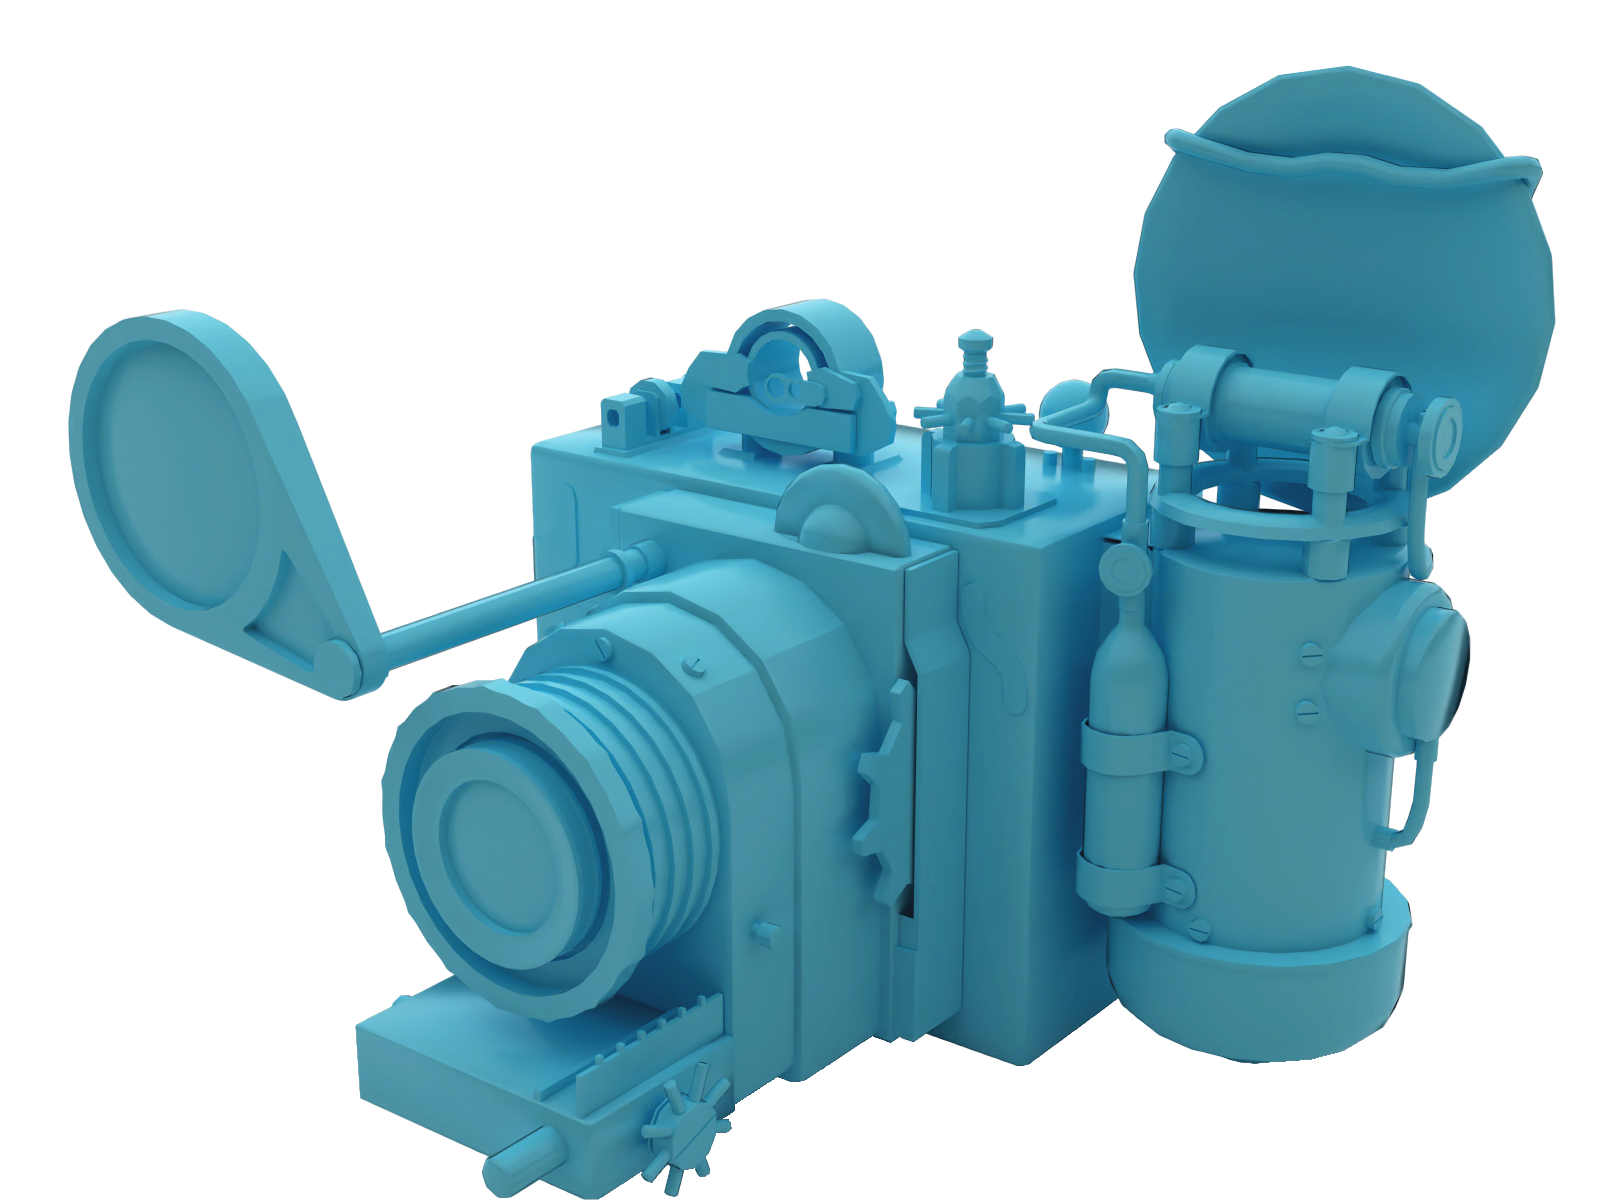} &
        \includegraphics[width=.24\textwidth]{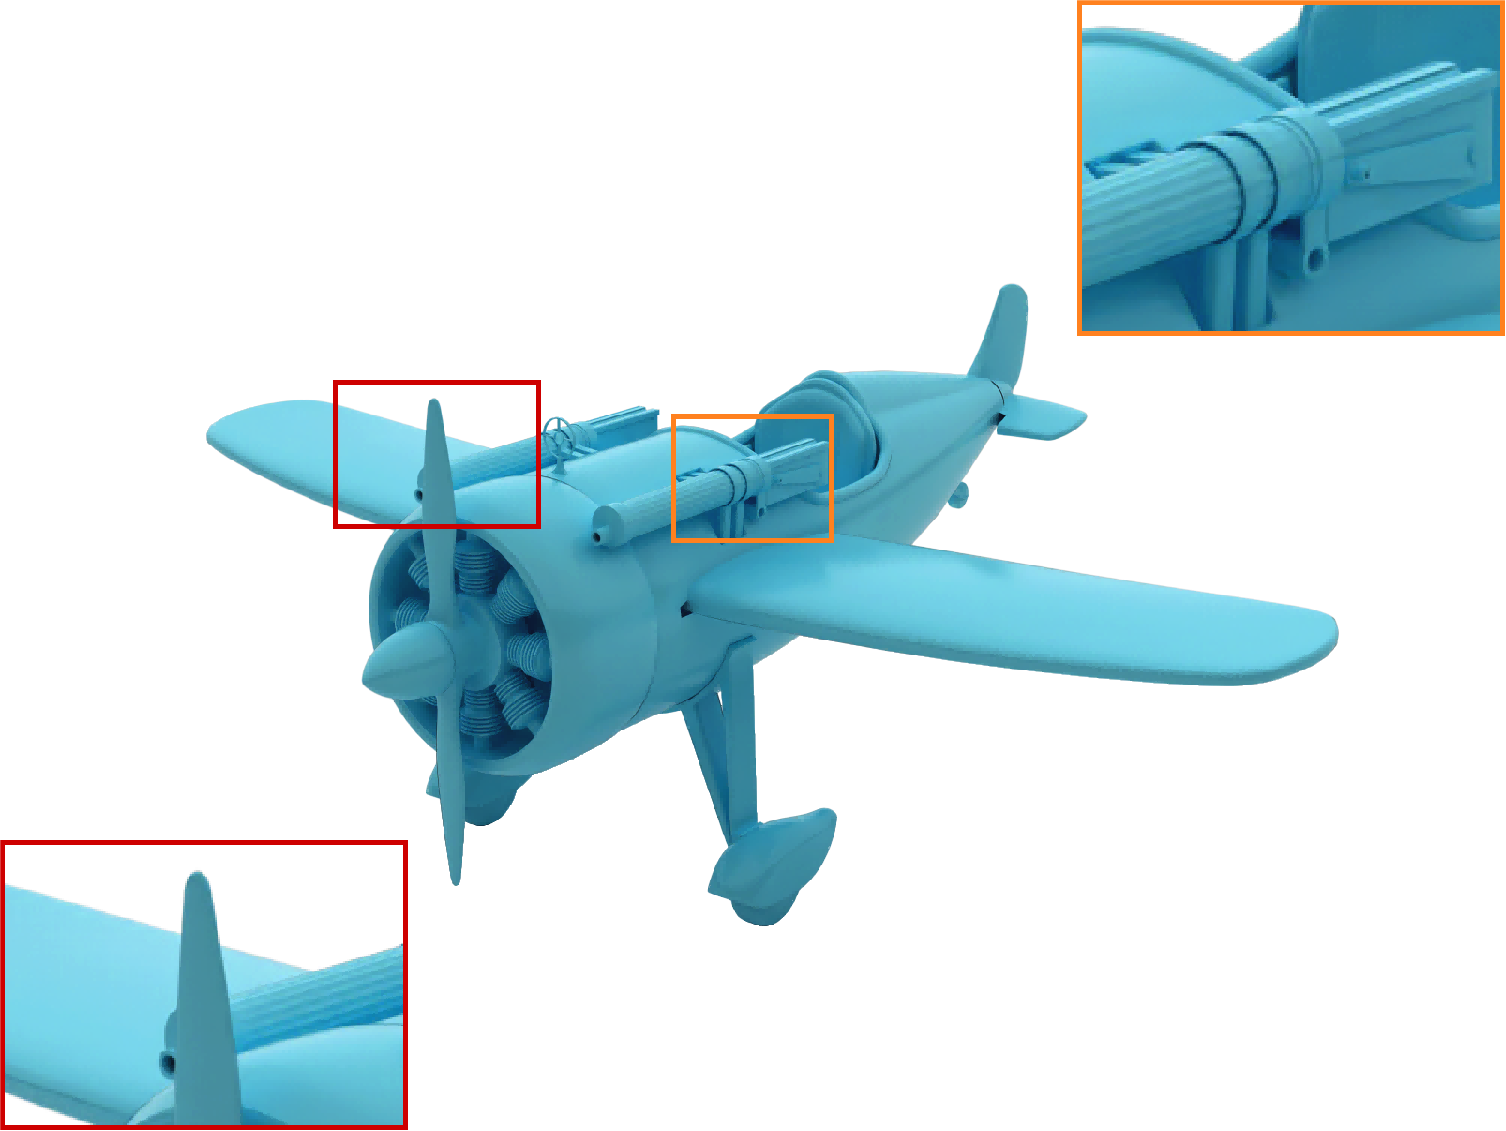} &
        \includegraphics[width=.24\textwidth]{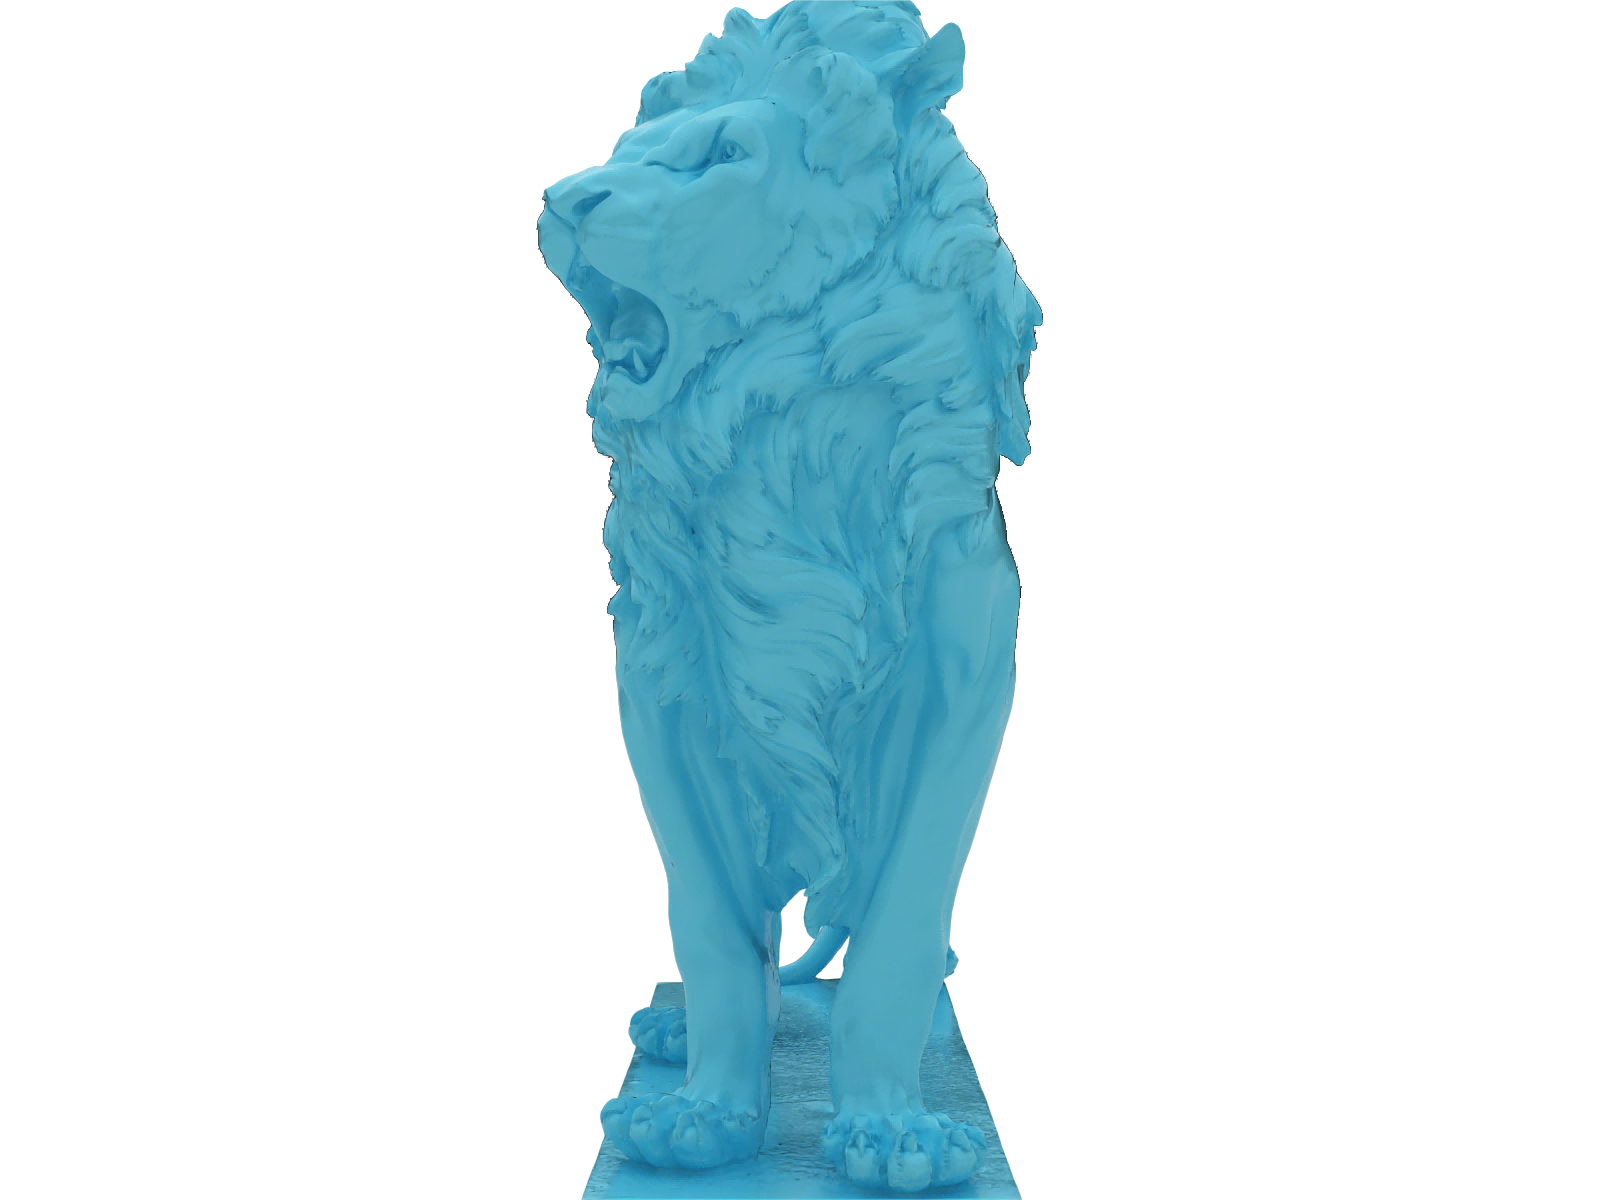} \\
        
        \rotatebox{90}{\parbox{\imghe}{\centering PGSR}} &
        \includegraphics[width=.24\textwidth]{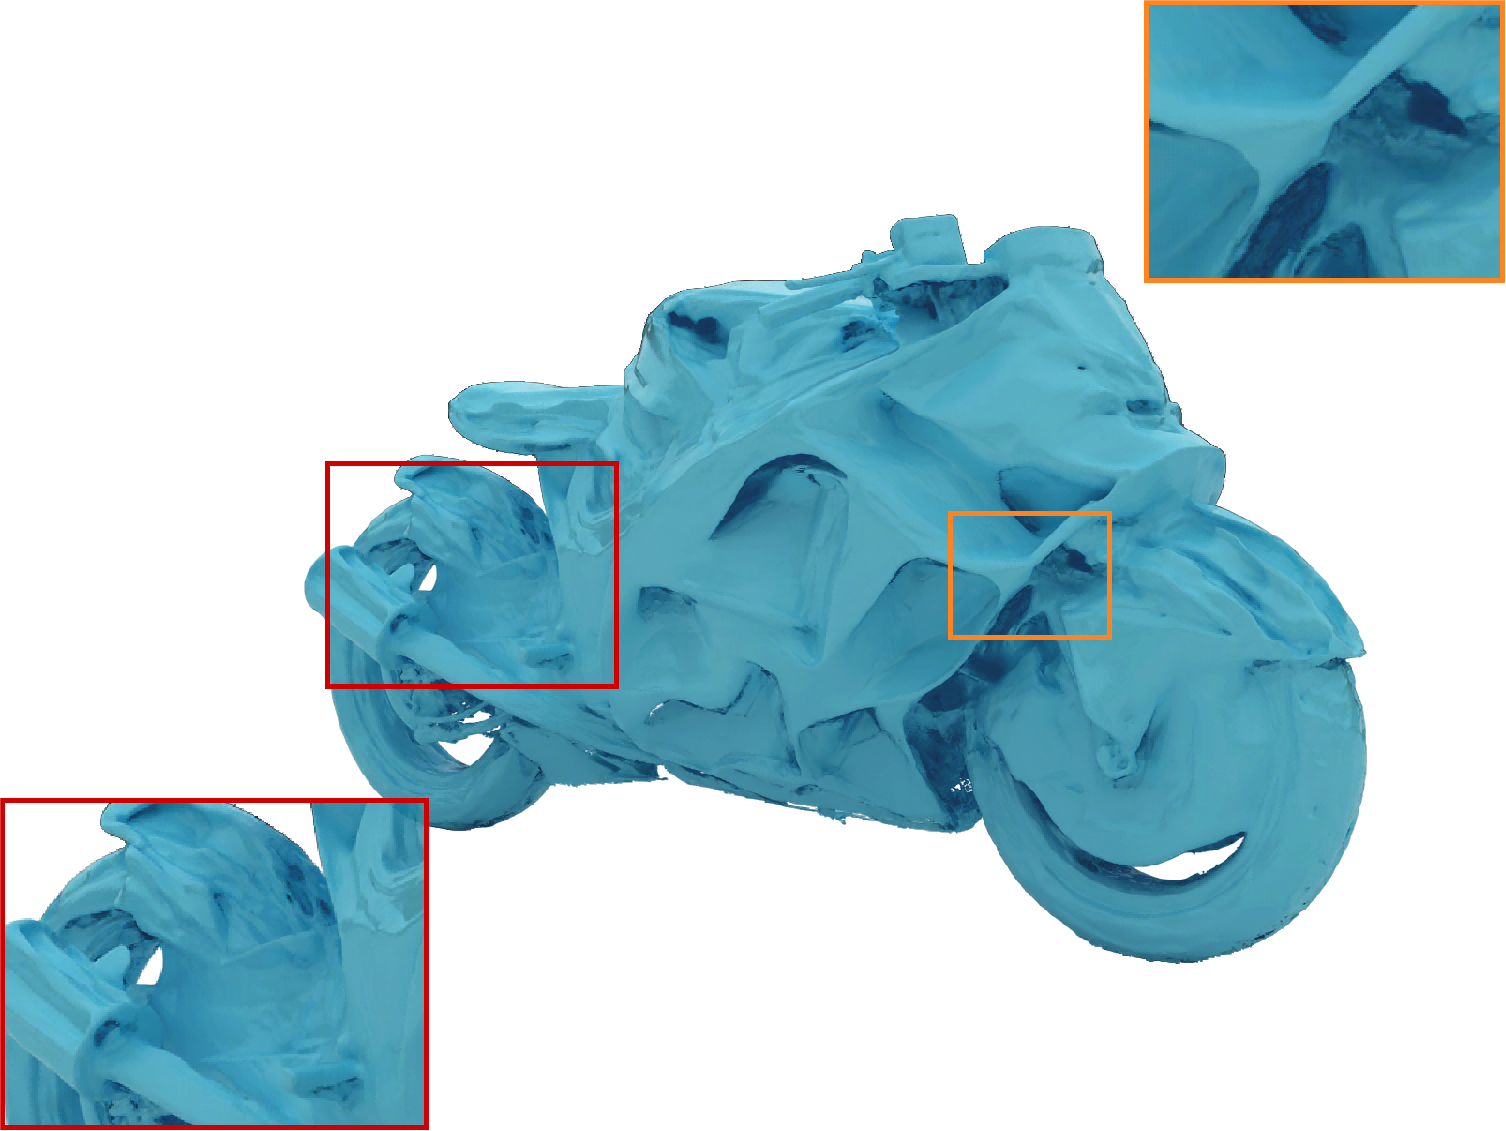} &
        \includegraphics[width=.24\textwidth]{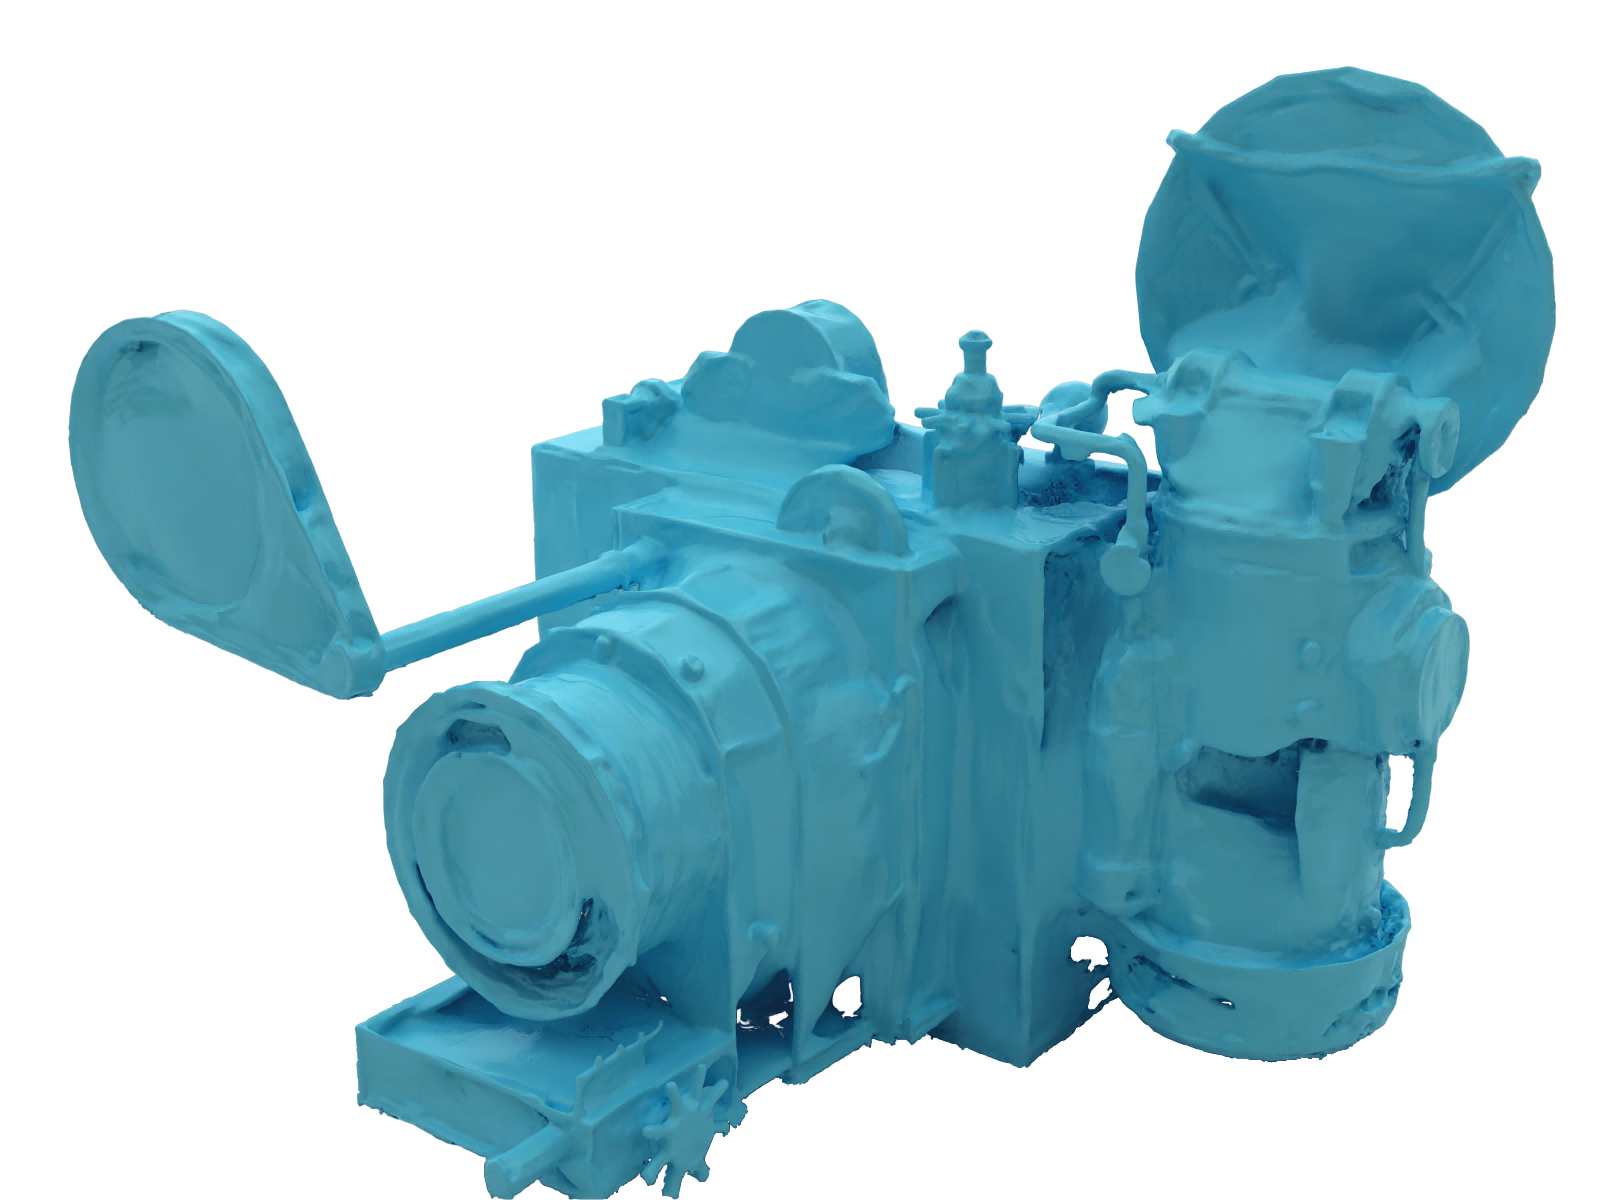} &
        \includegraphics[width=.24\textwidth]{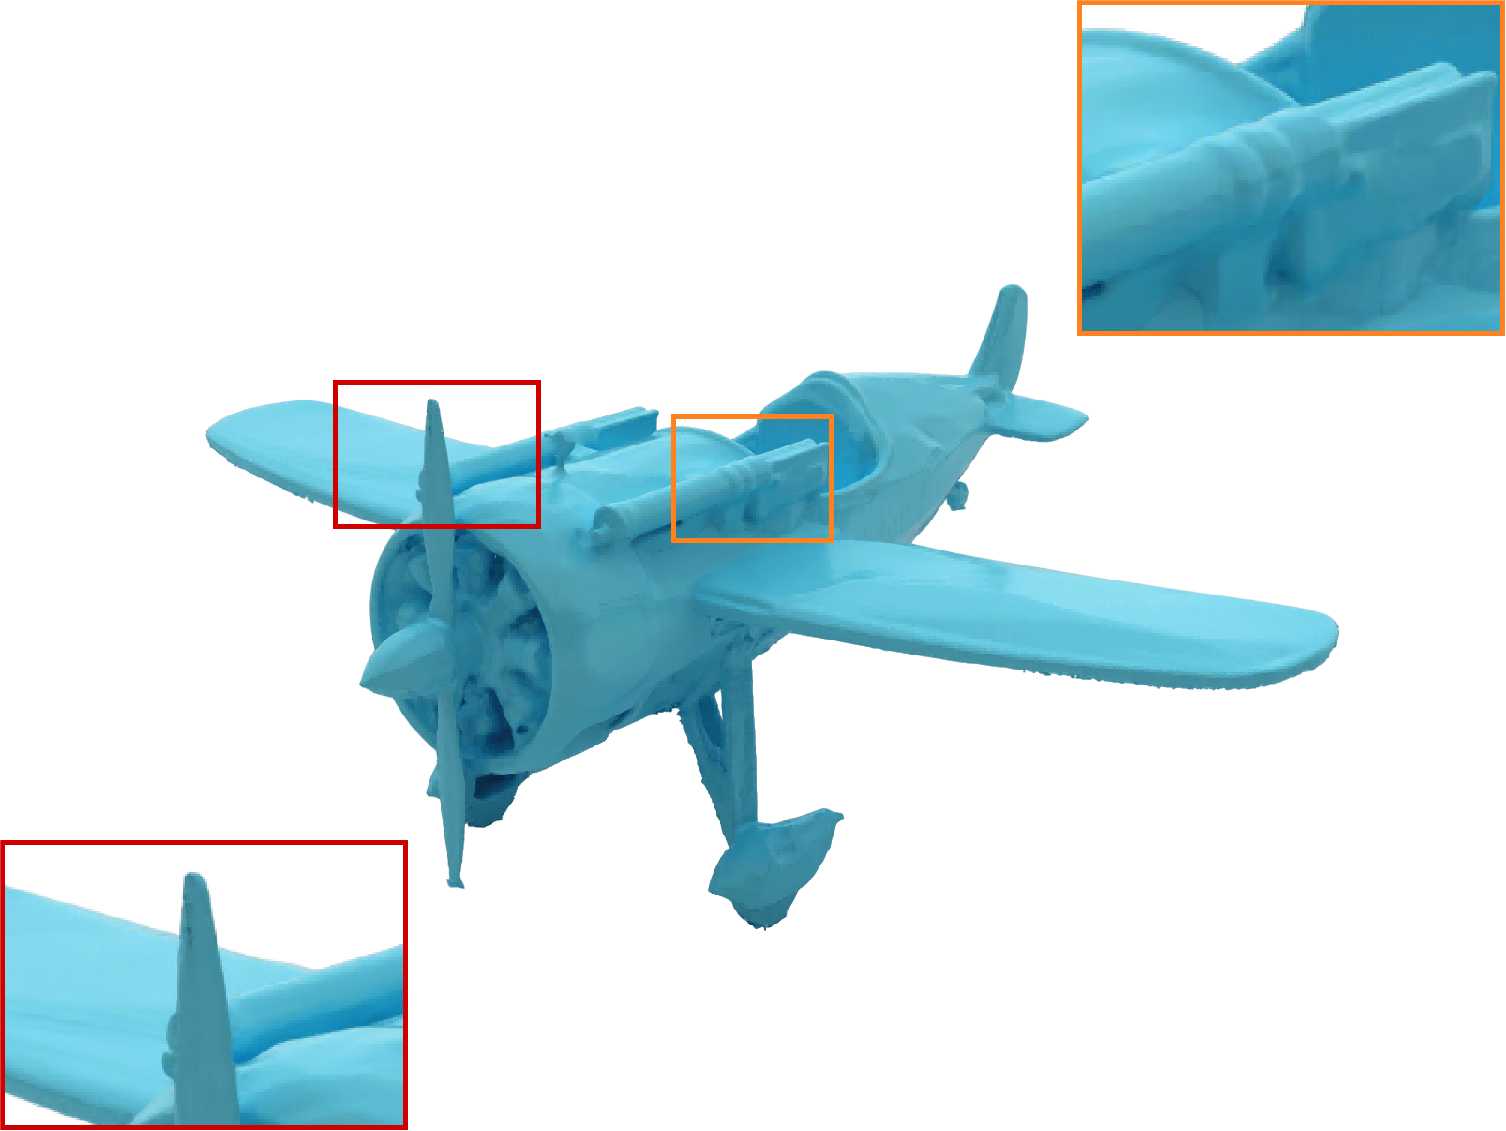} &
        \includegraphics[width=.24\textwidth]{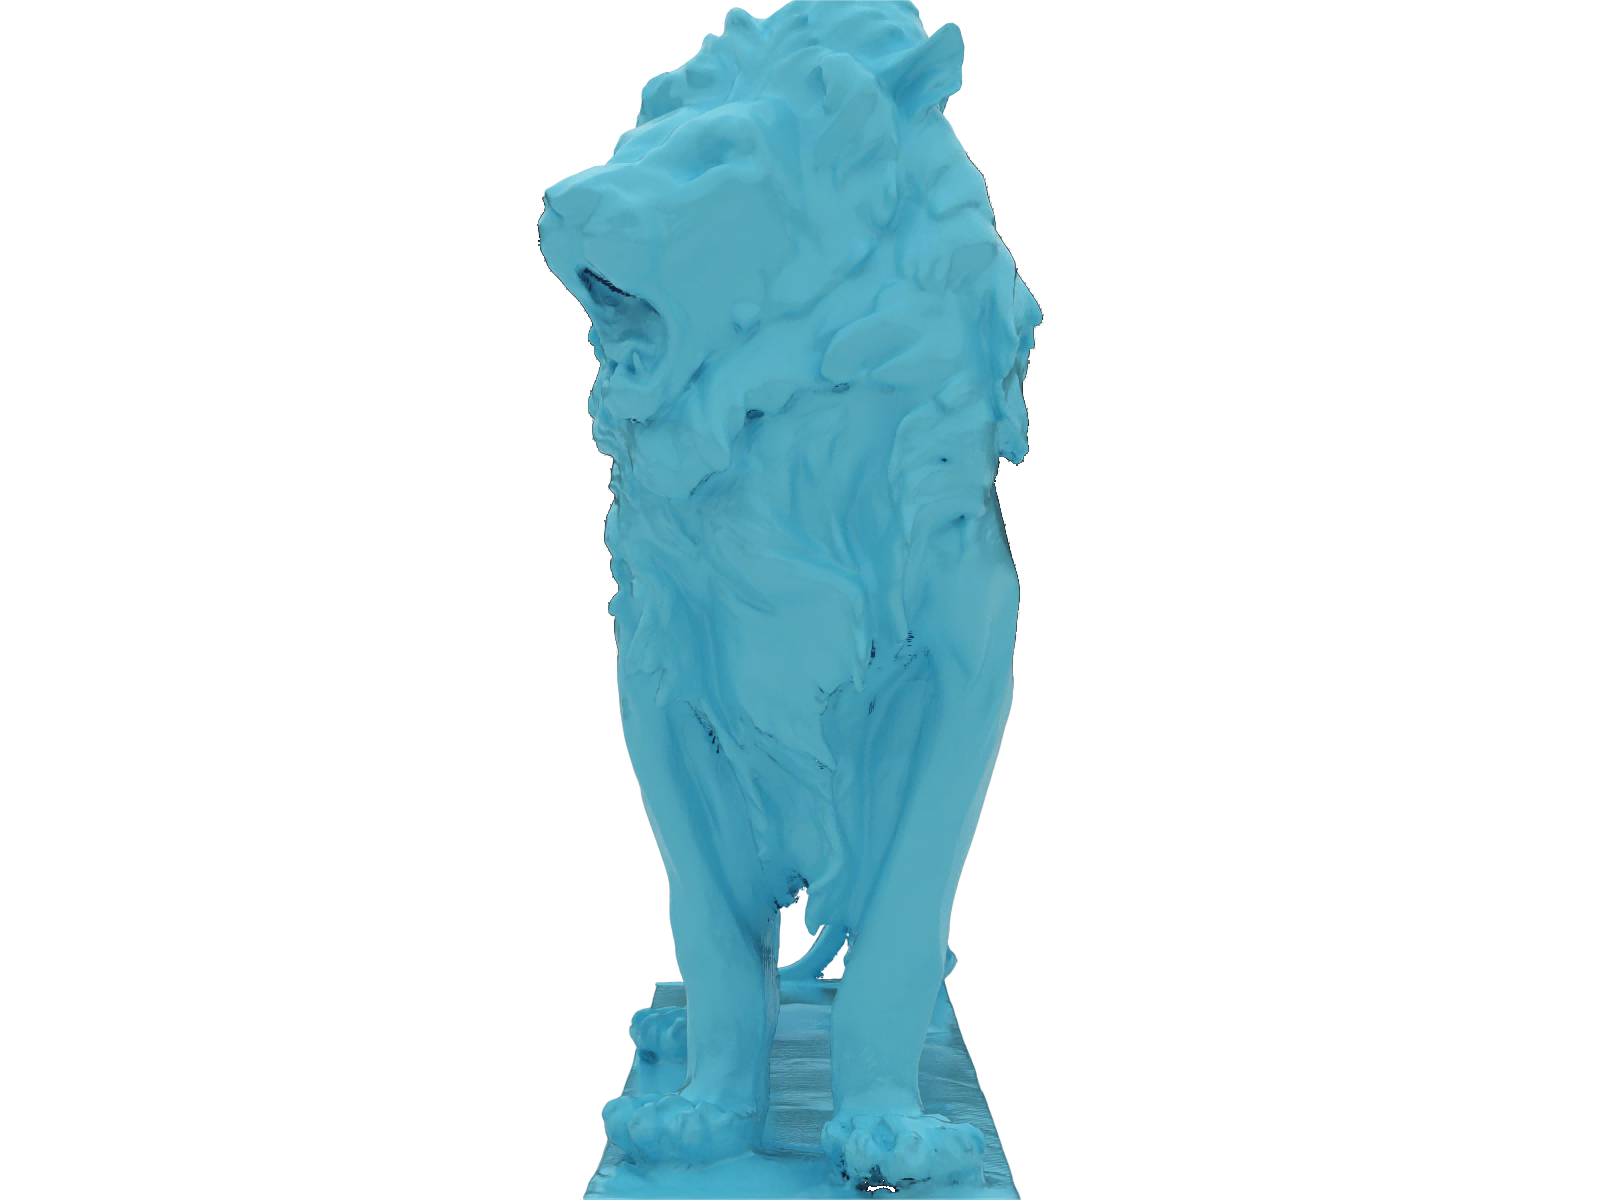} \\
        
        \rotatebox{90}{\parbox{\imghe}{\centering 2DGS}} &
        \includegraphics[width=.24\textwidth]{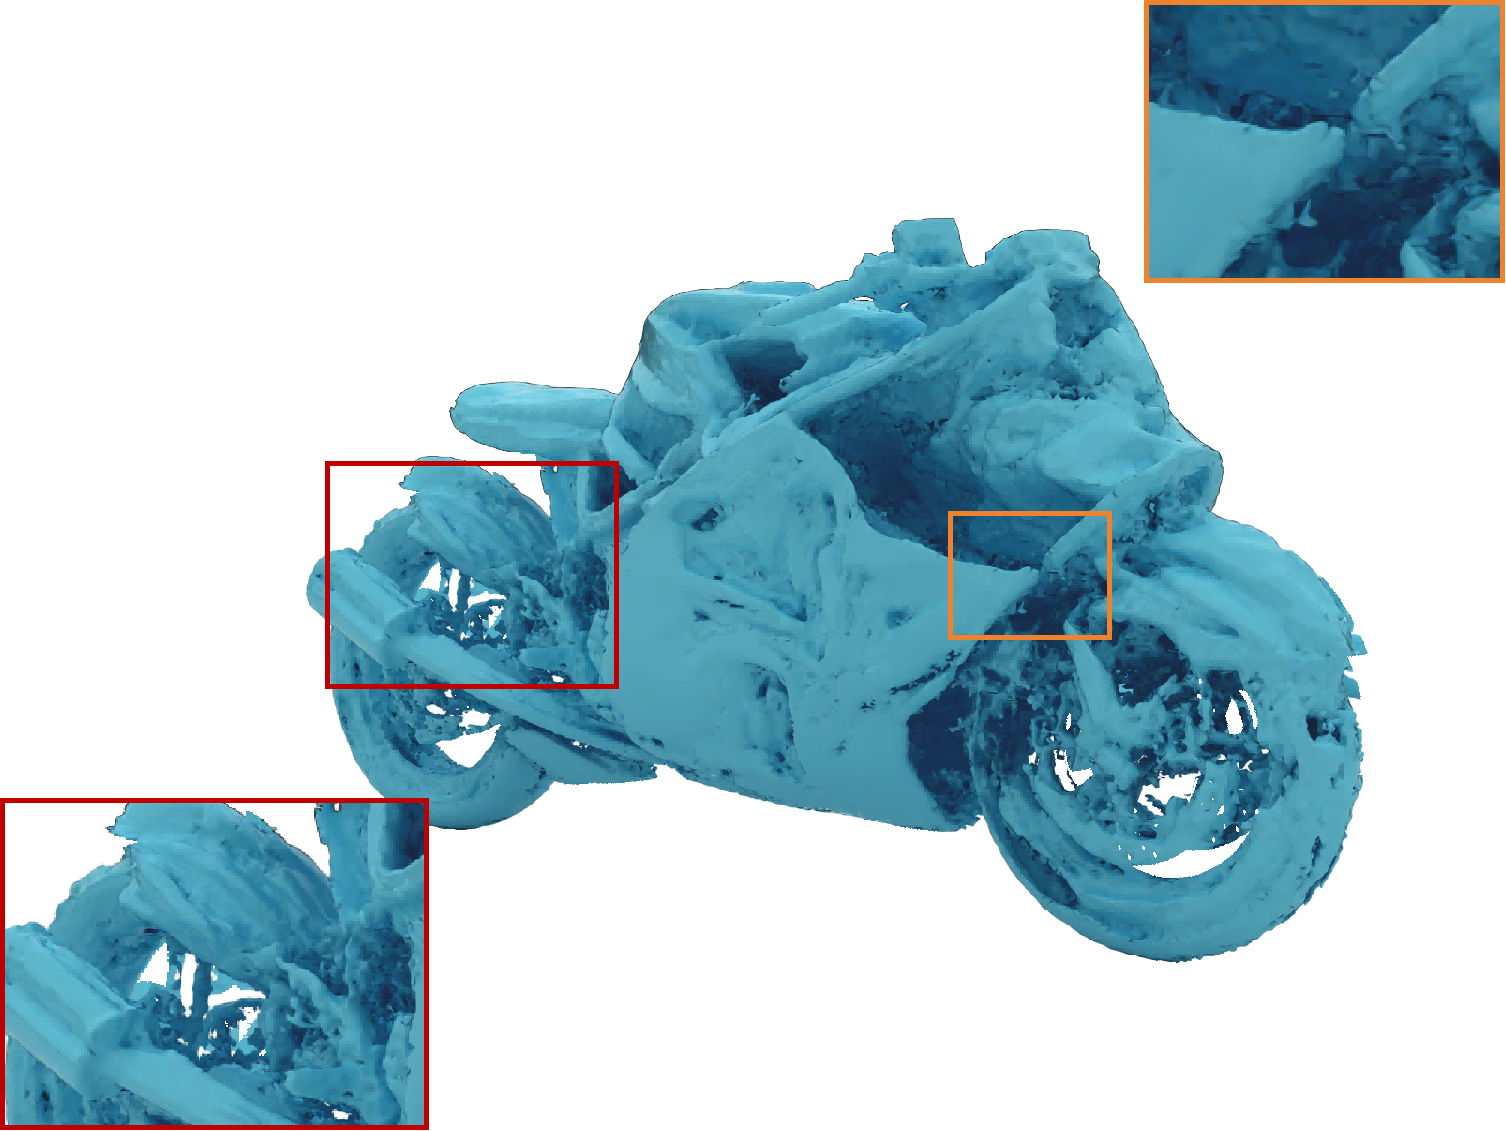} &
        \includegraphics[width=.24\textwidth]{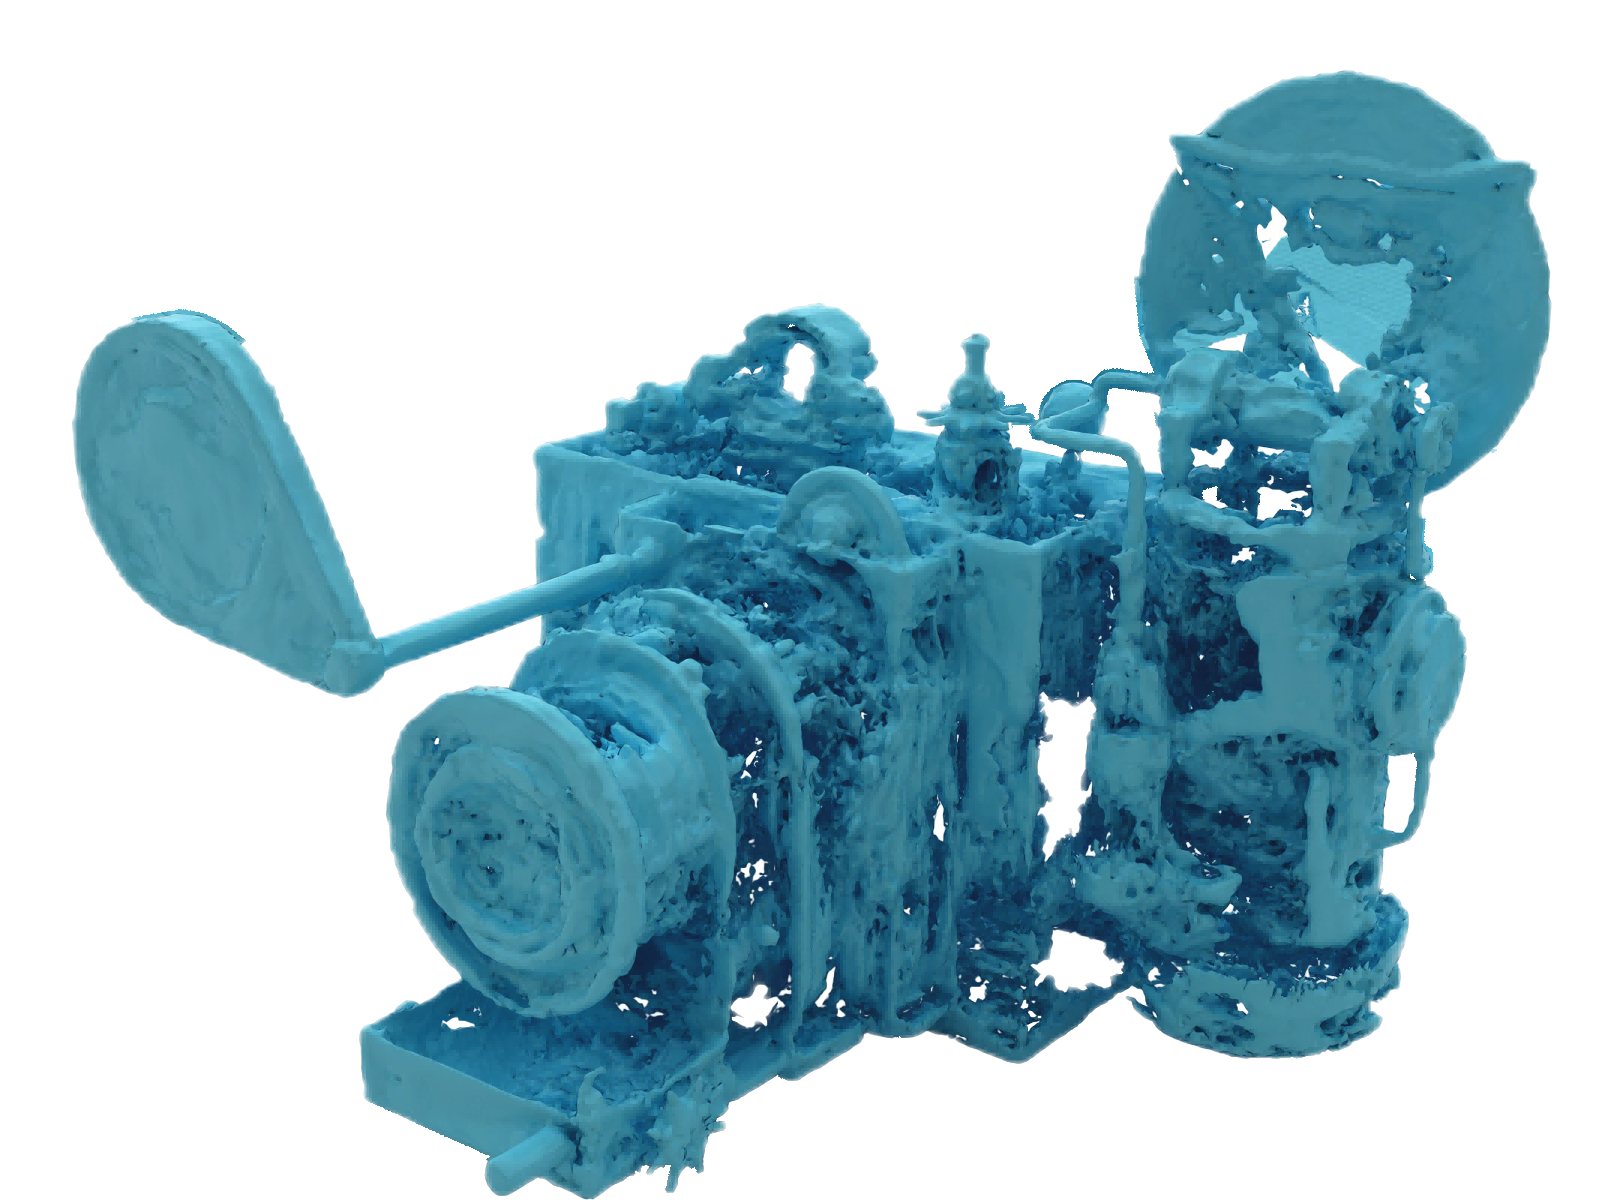} &
        \includegraphics[width=.24\textwidth]{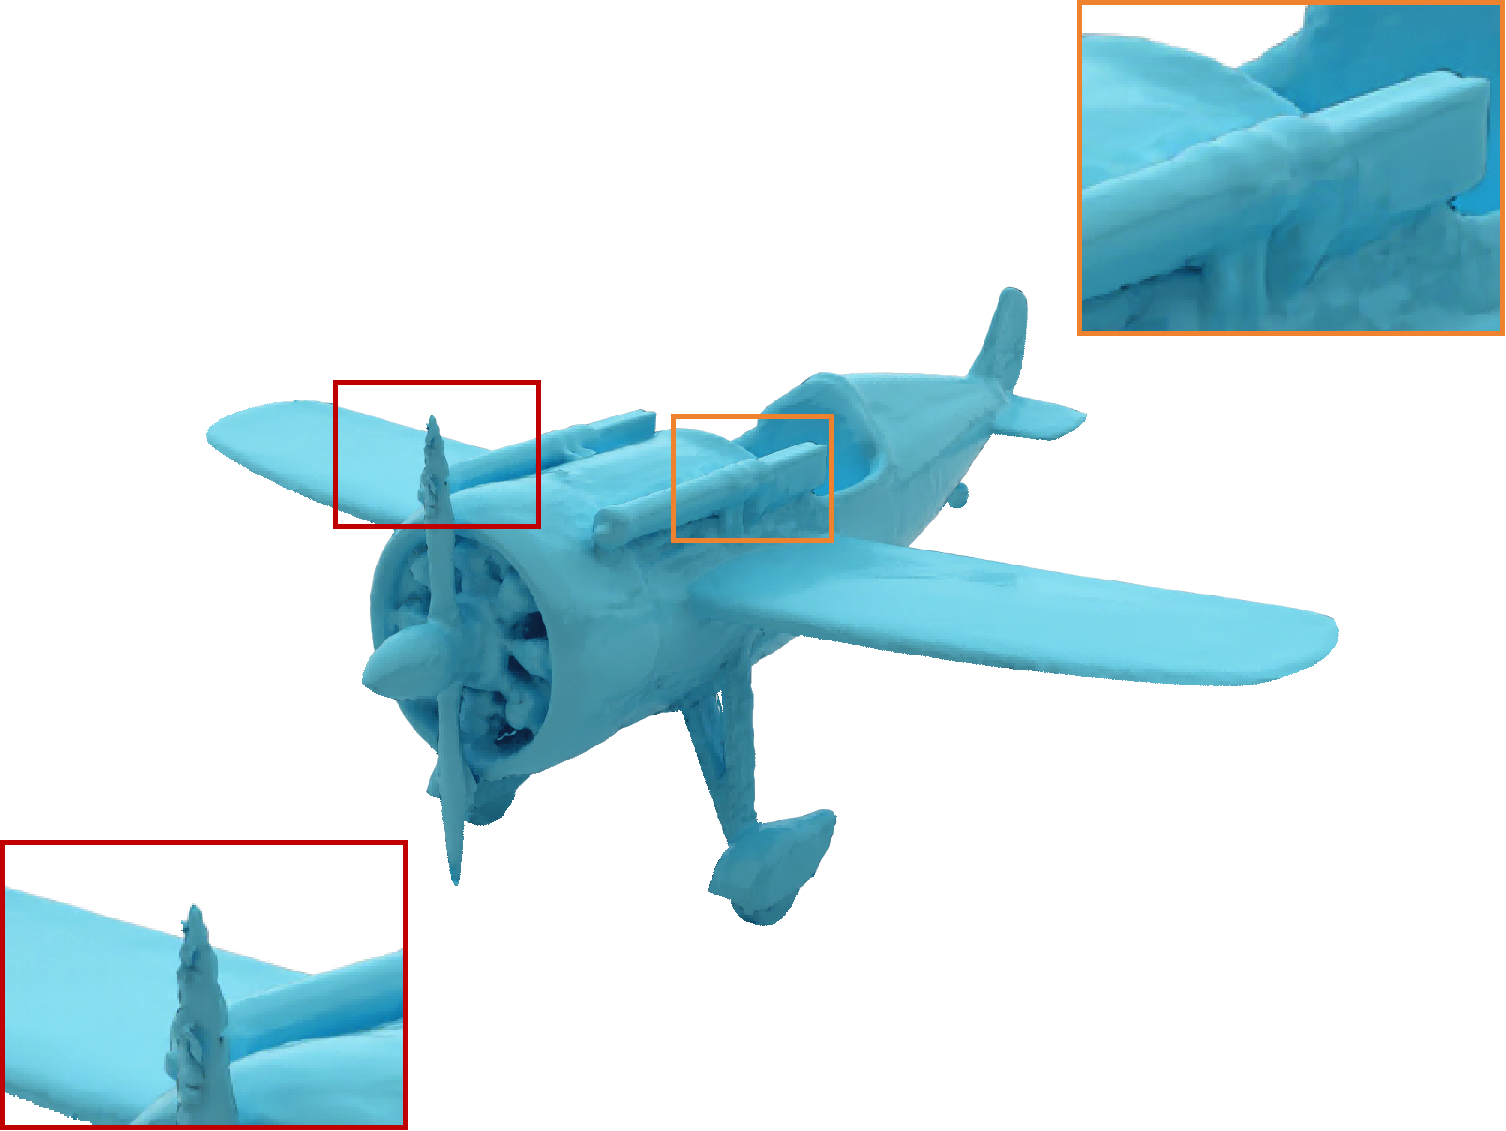} &
        \includegraphics[width=.24\textwidth]{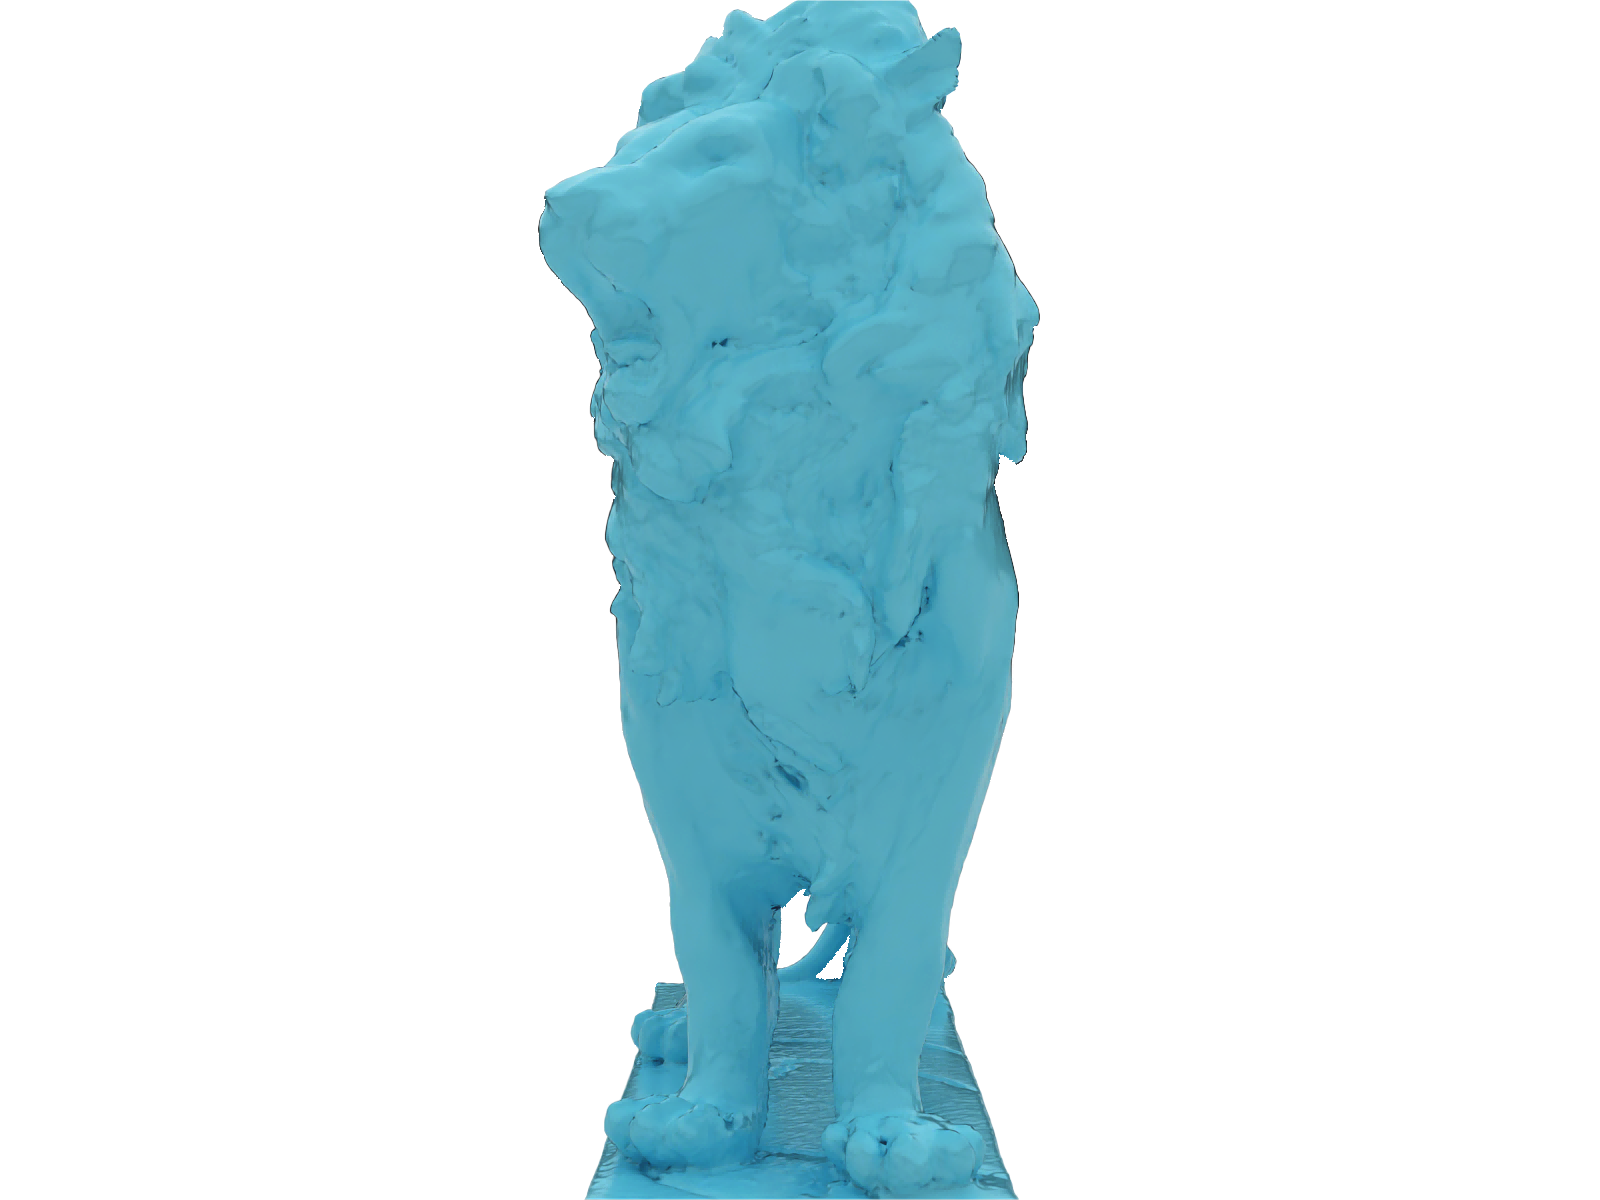} \\

        \rotatebox{90}{\parbox{\imghe}{\centering NeRRF}} &
        \includegraphics[width=.24\textwidth]{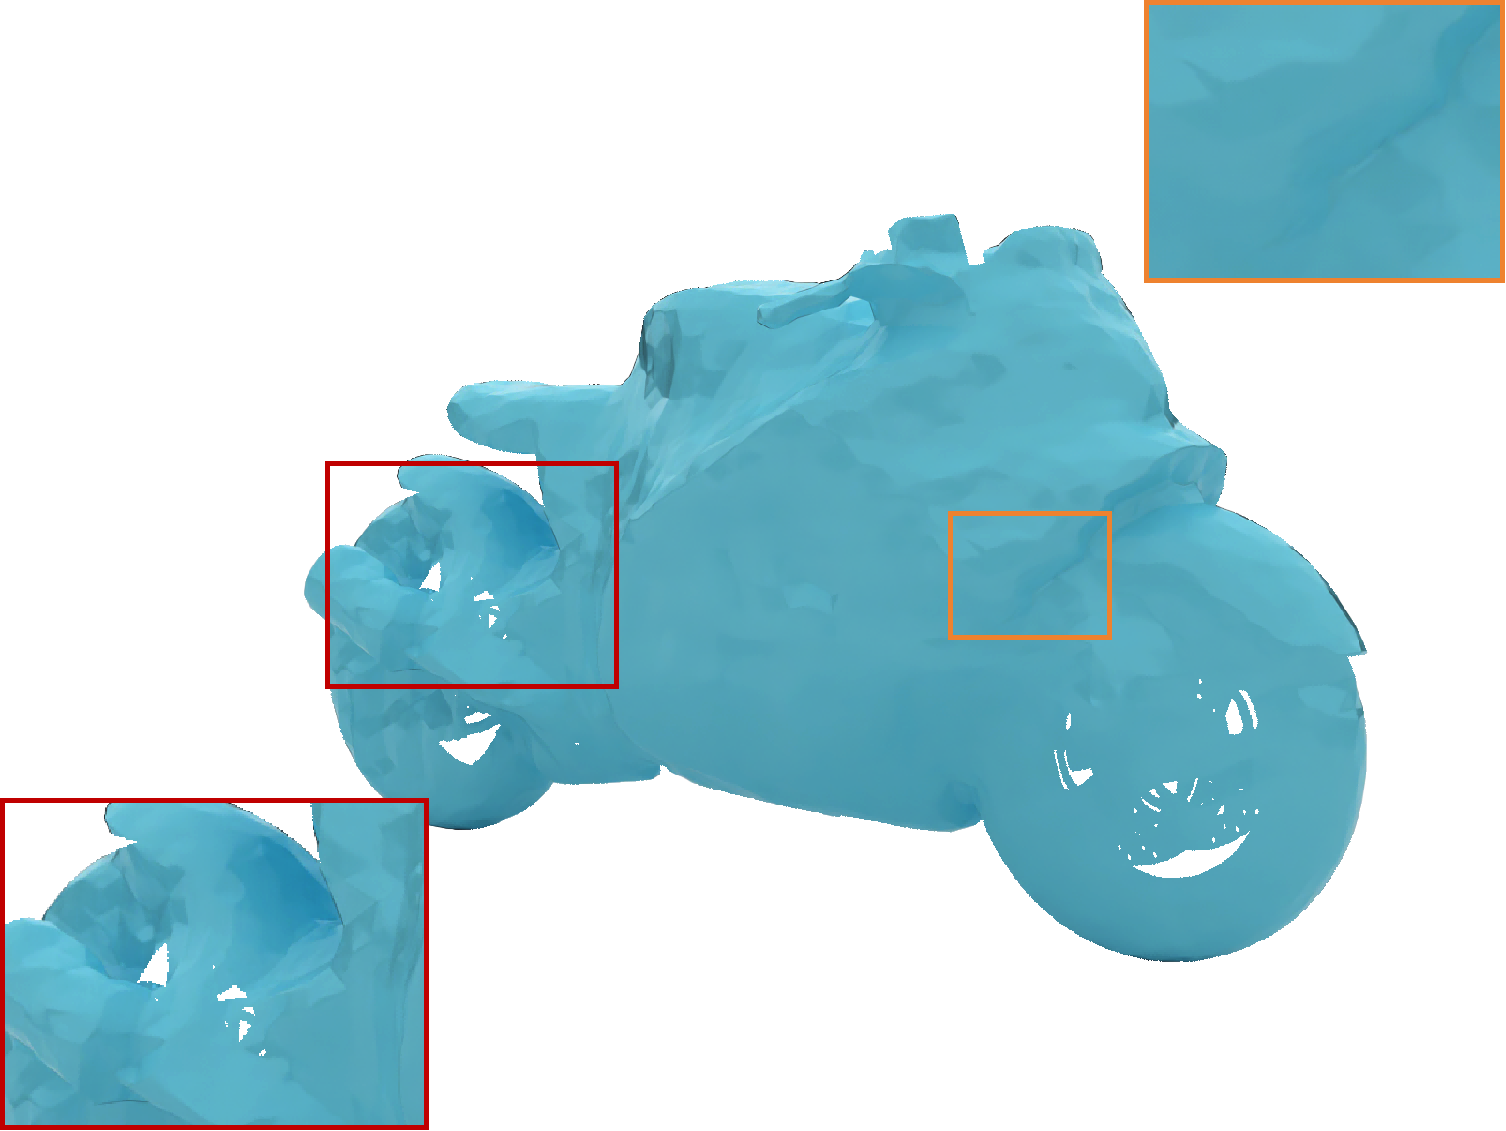} &
        \includegraphics[width=.24\textwidth]{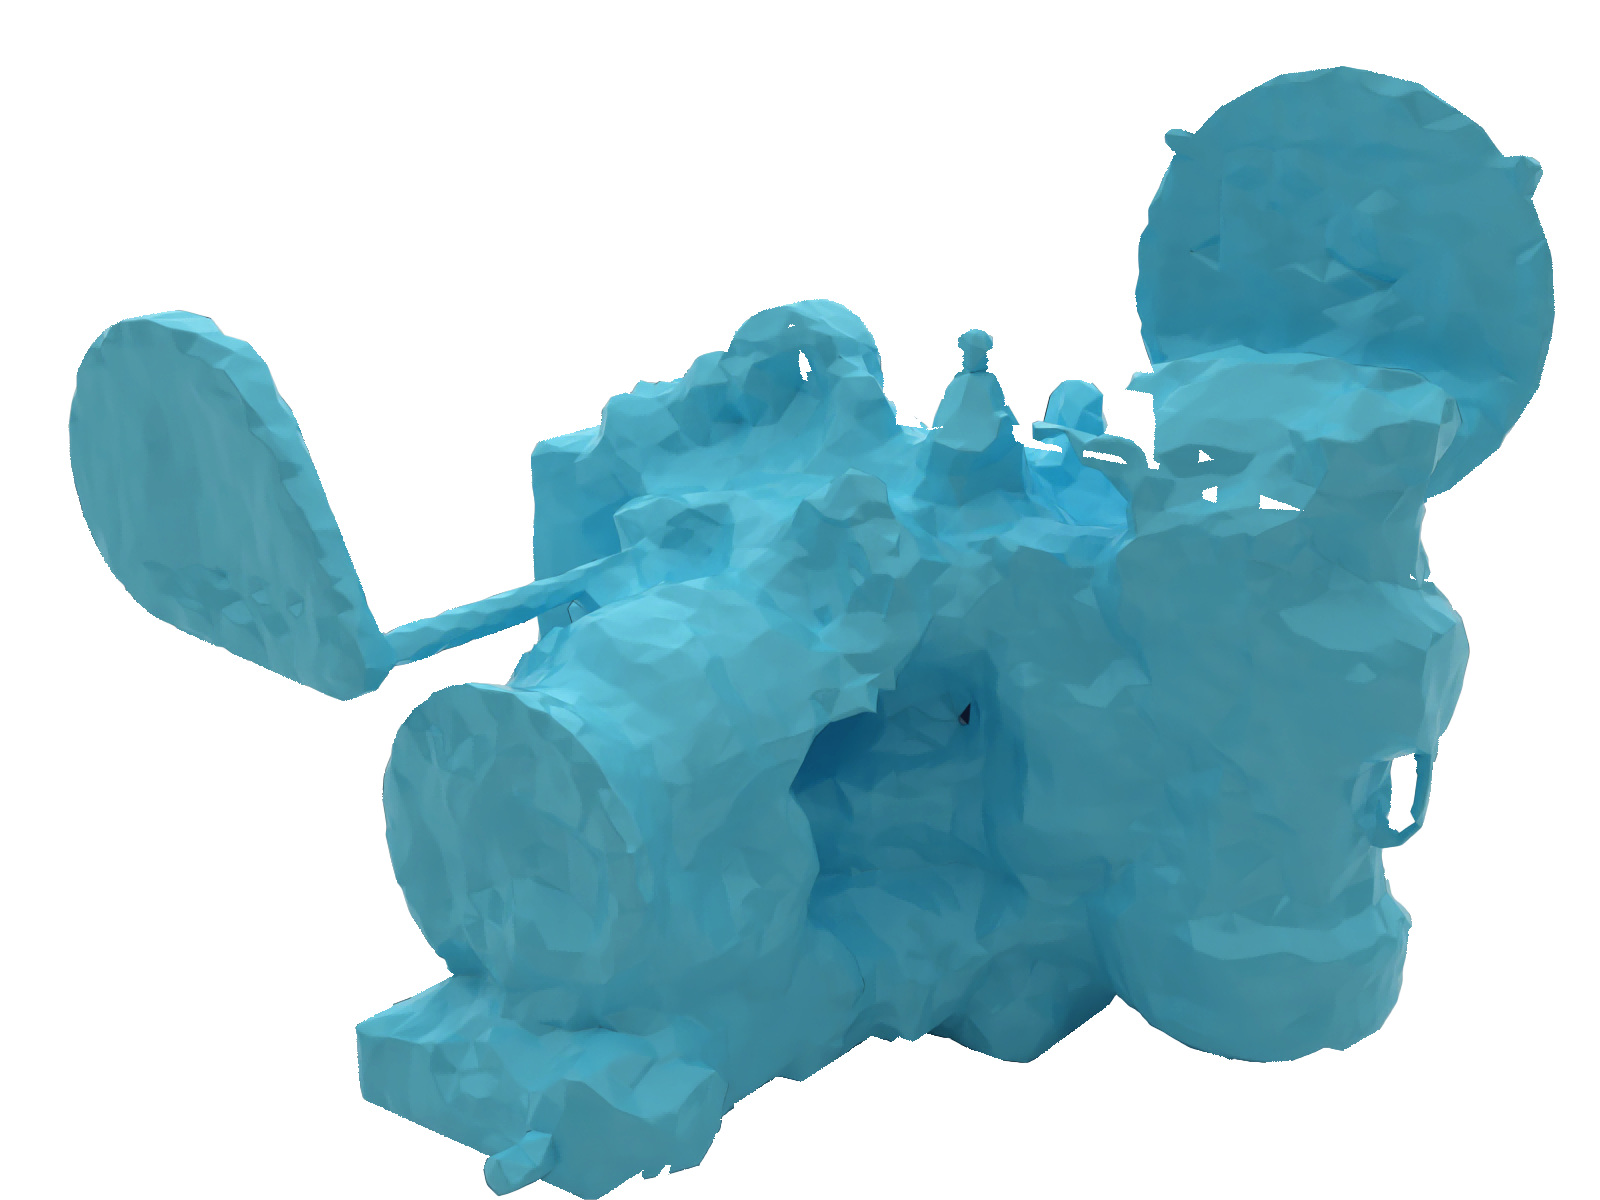} &
        \includegraphics[width=.24\textwidth]{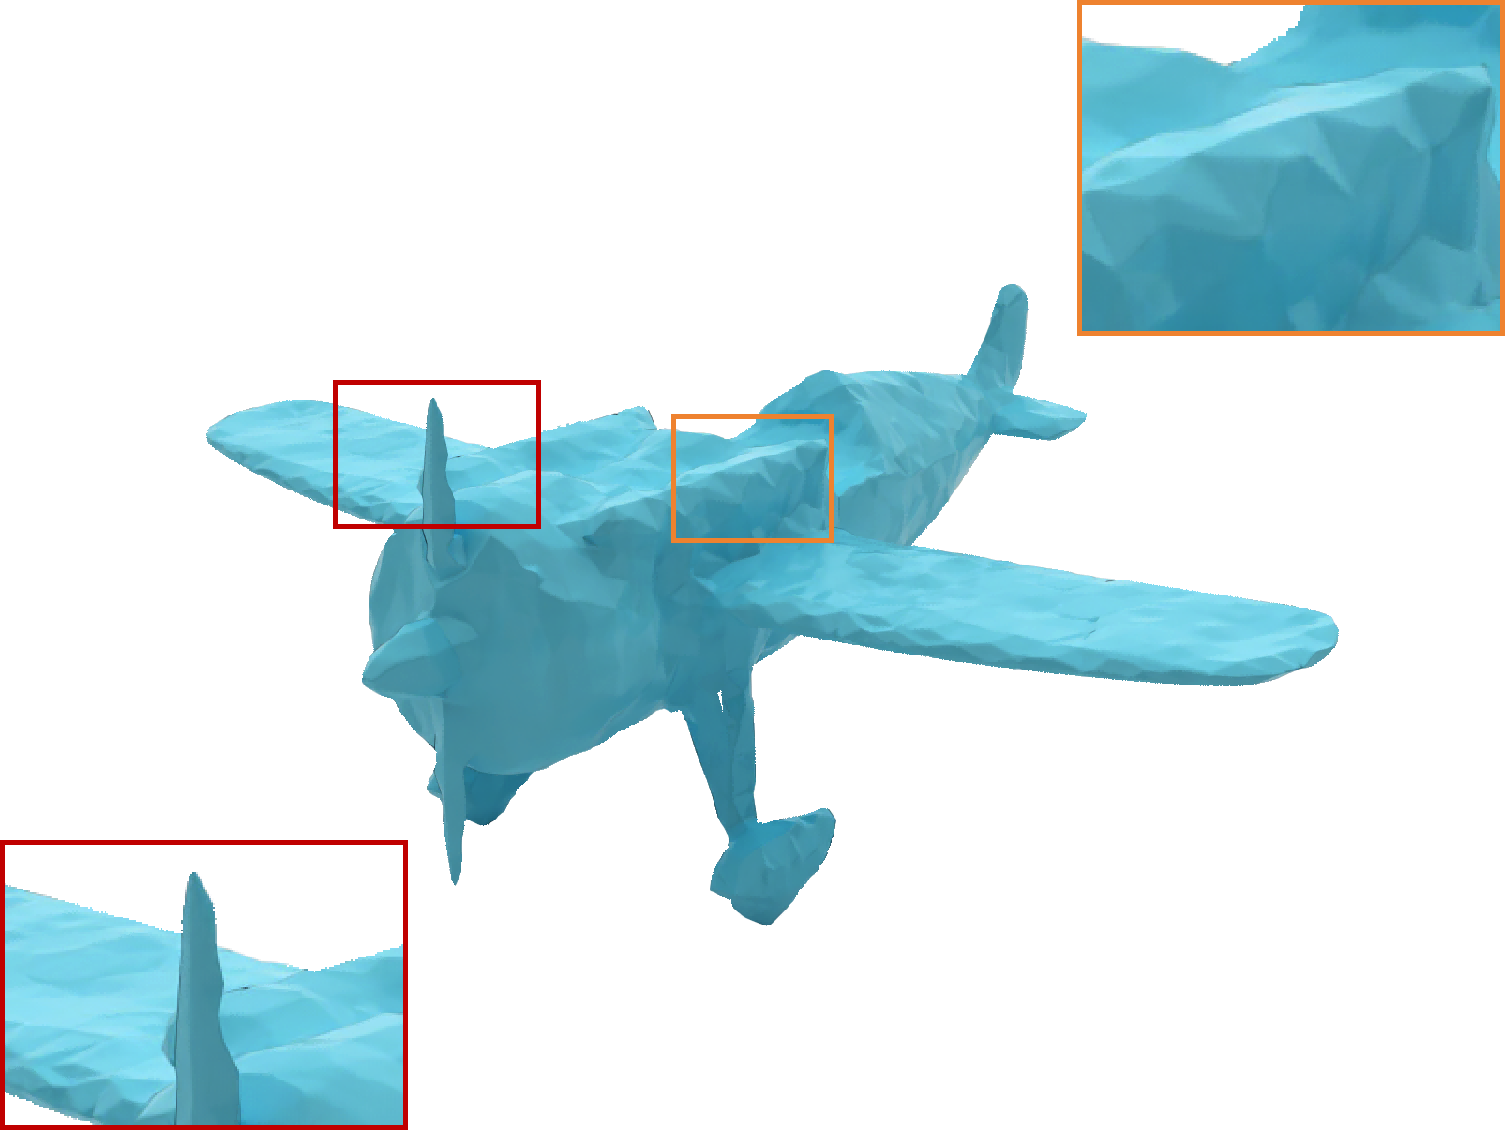} &
        \includegraphics[width=.24\textwidth]{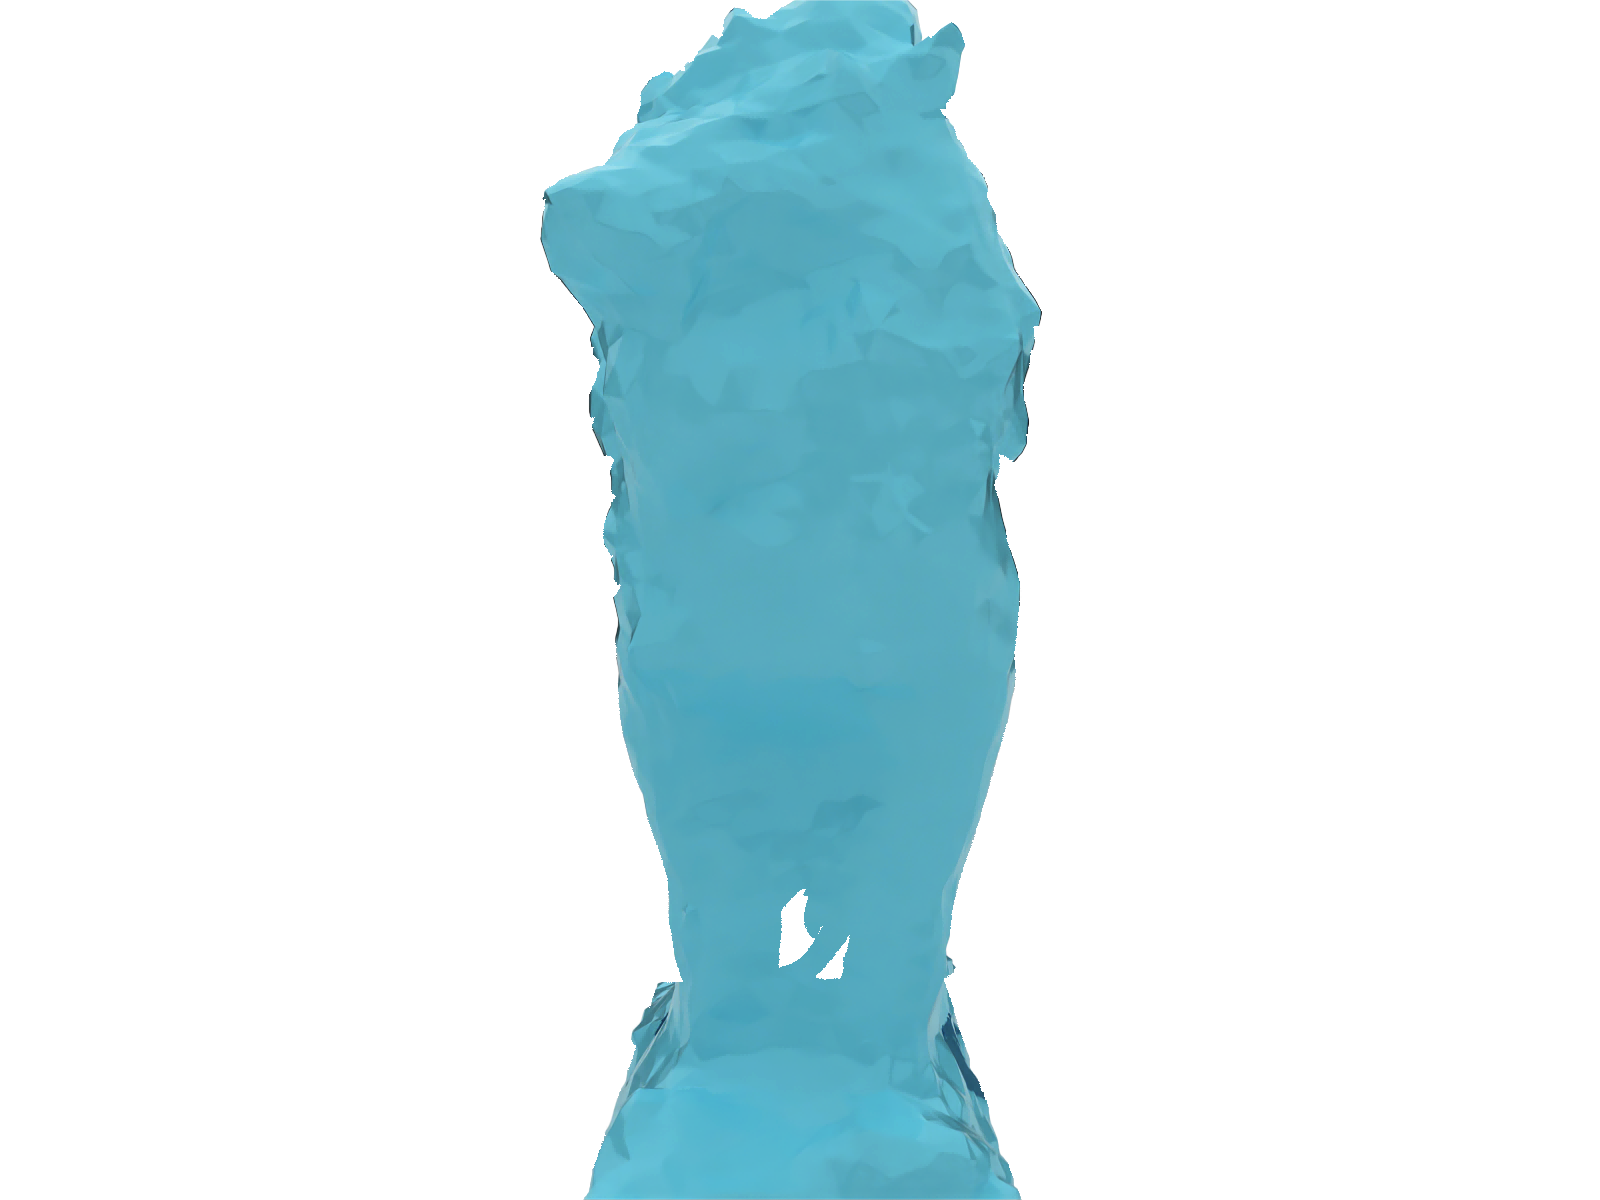} \\

        \rotatebox{90}{\parbox{\imghe}{\centering NeRO}} &
        \includegraphics[width=.24\textwidth]{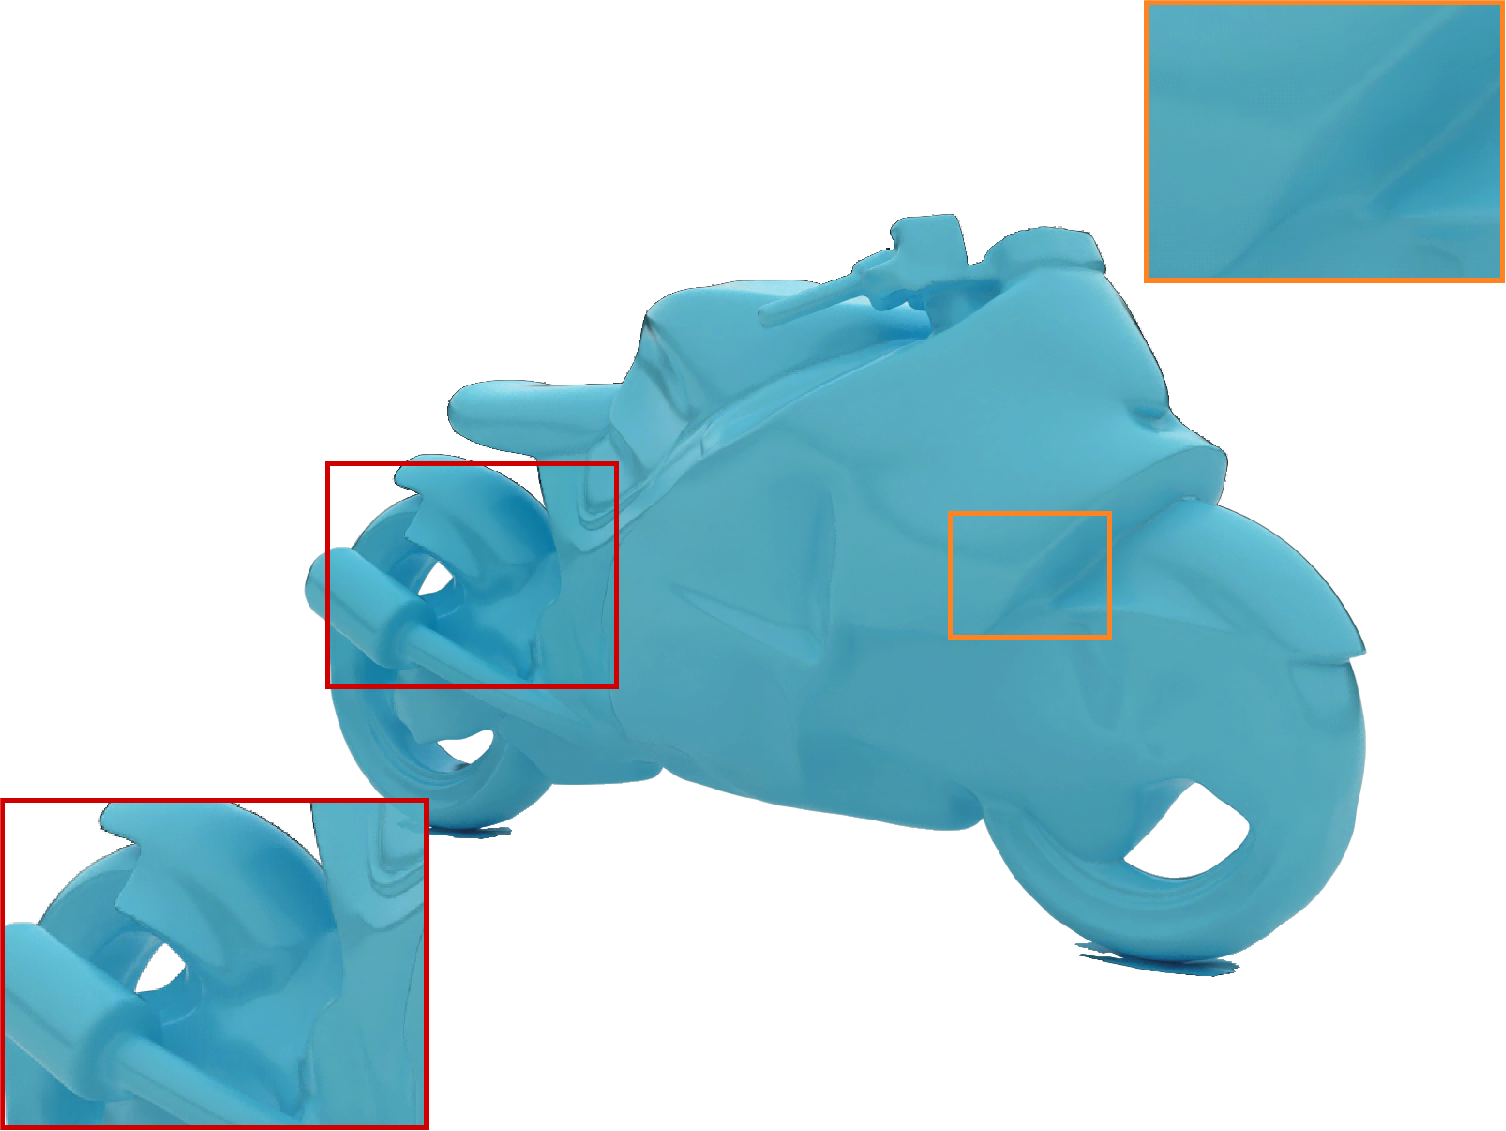} &
        \includegraphics[width=.24\textwidth]{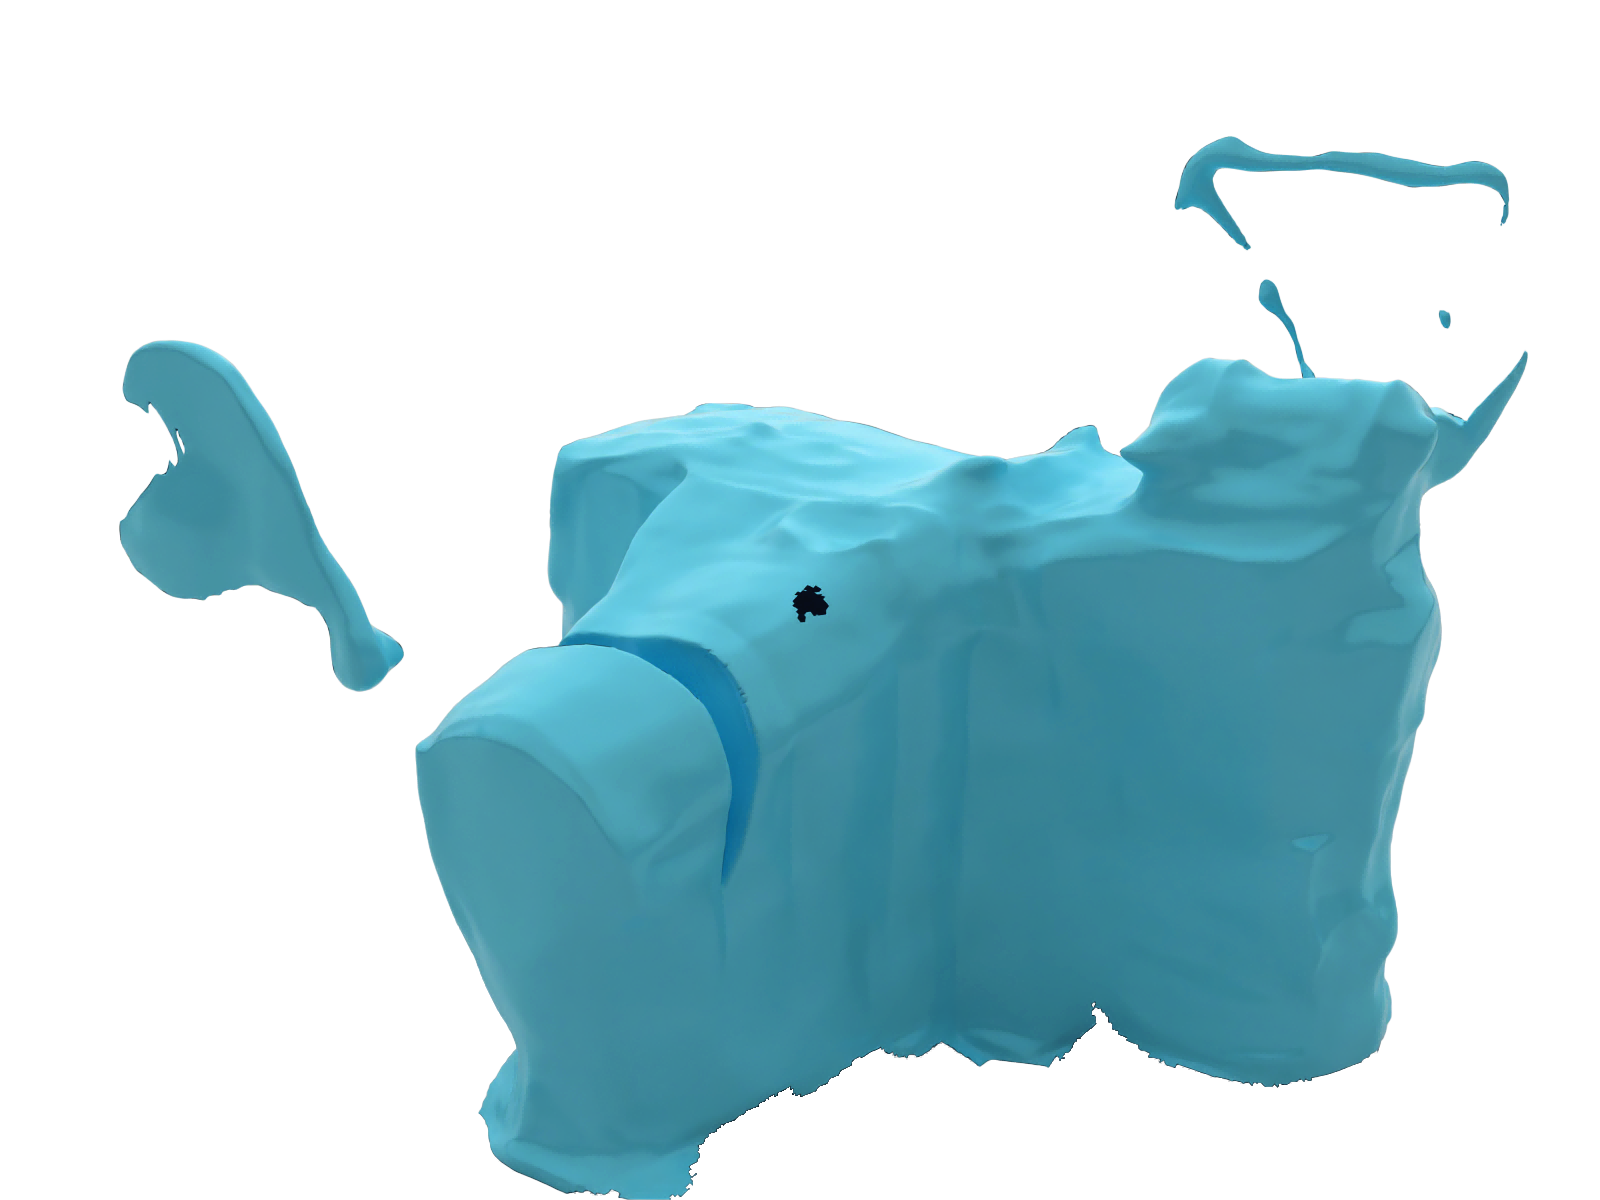} &
        \includegraphics[width=.24\textwidth]{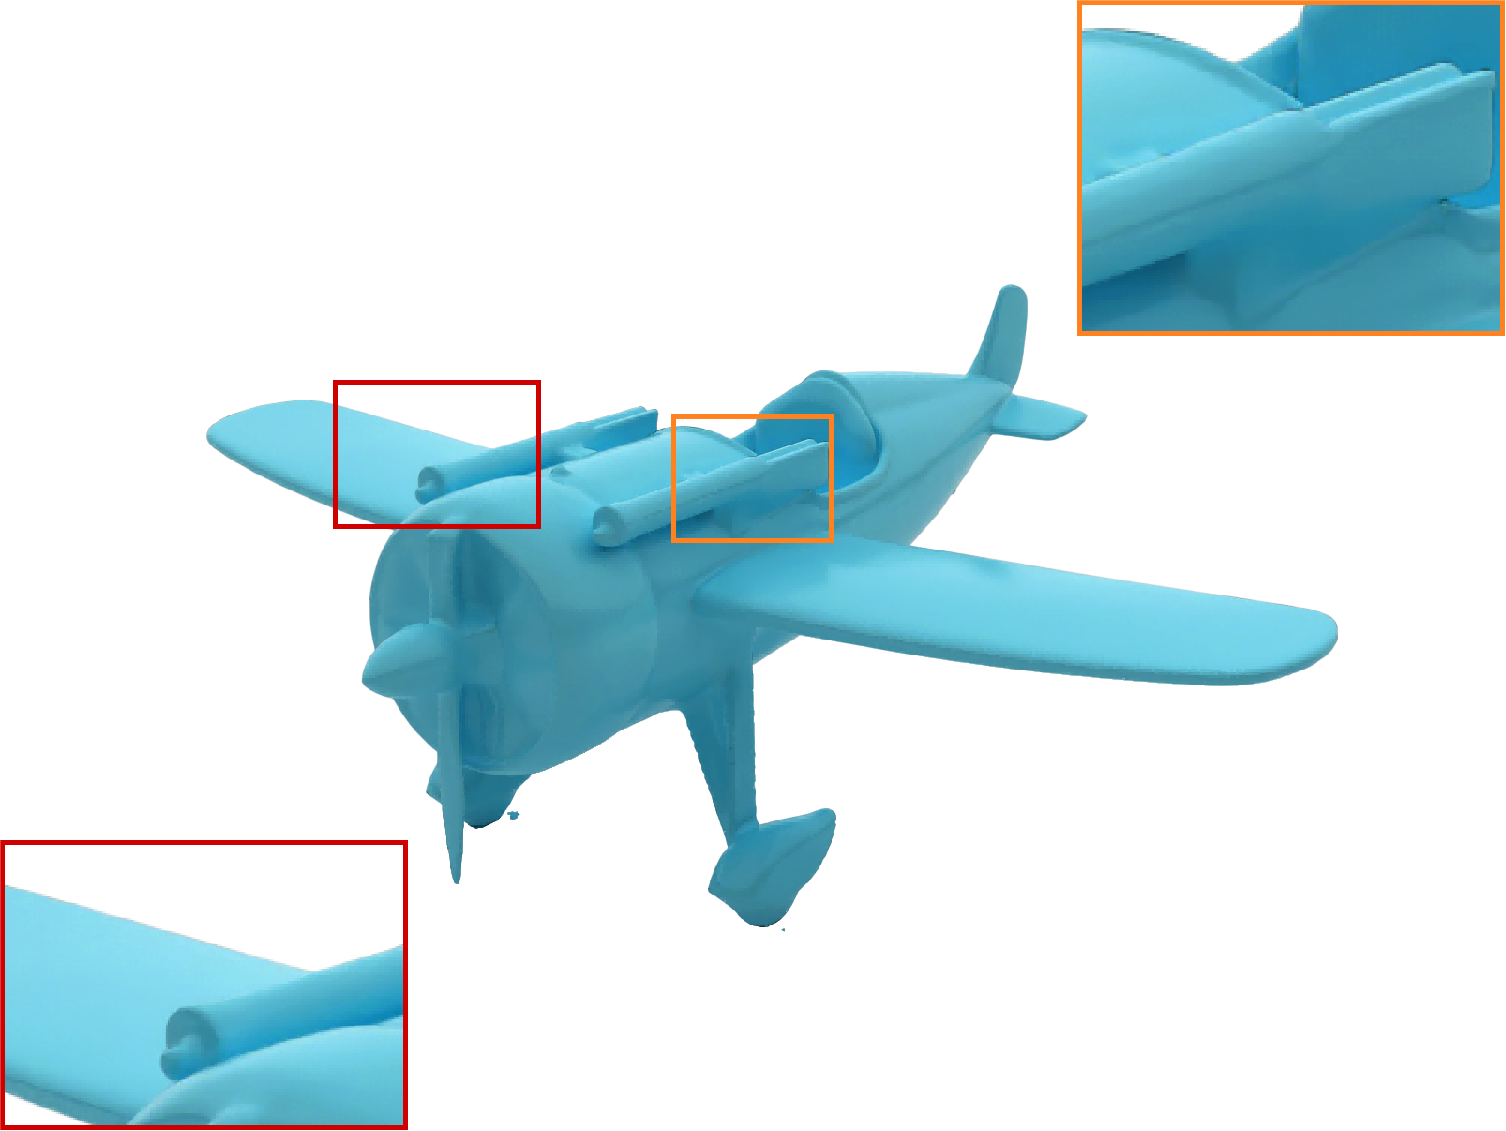} &
        \includegraphics[width=.24\textwidth]{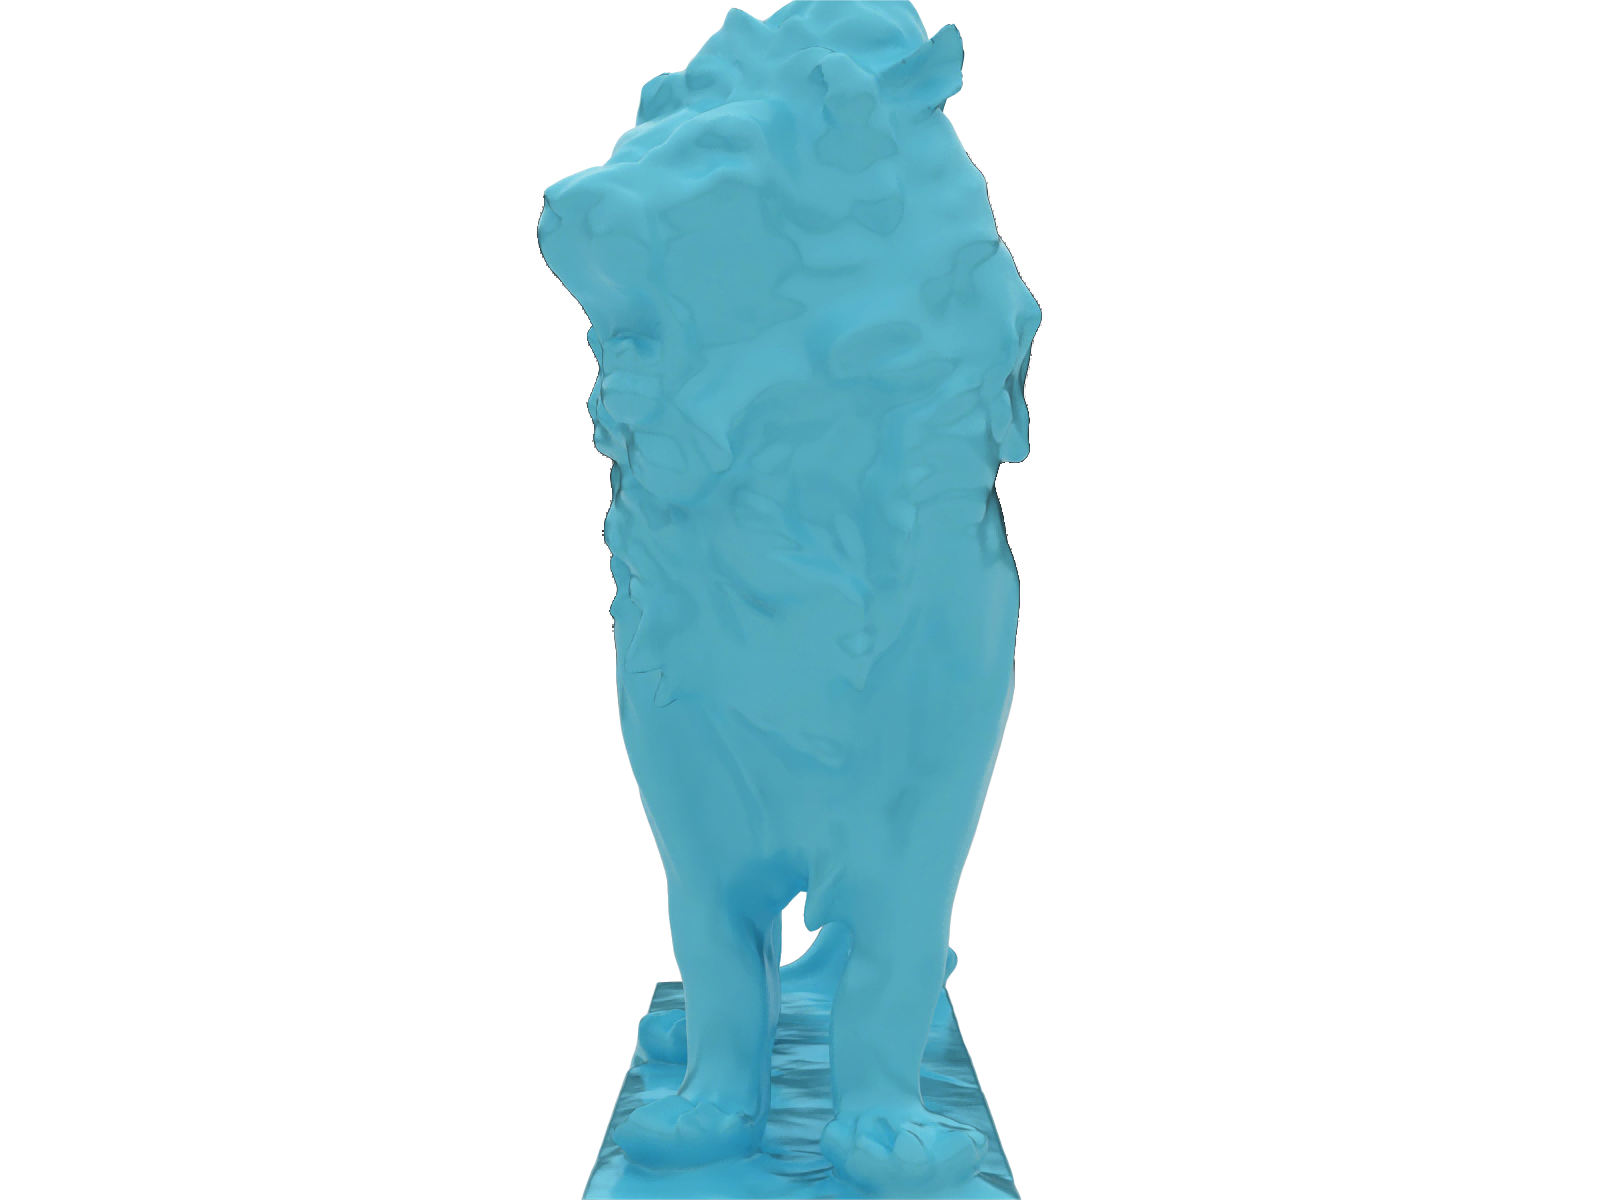} \\

        \rotatebox{90}{\parbox{\imghe}{\centering Instant-NGP}} &
        \includegraphics[width=.24\textwidth]{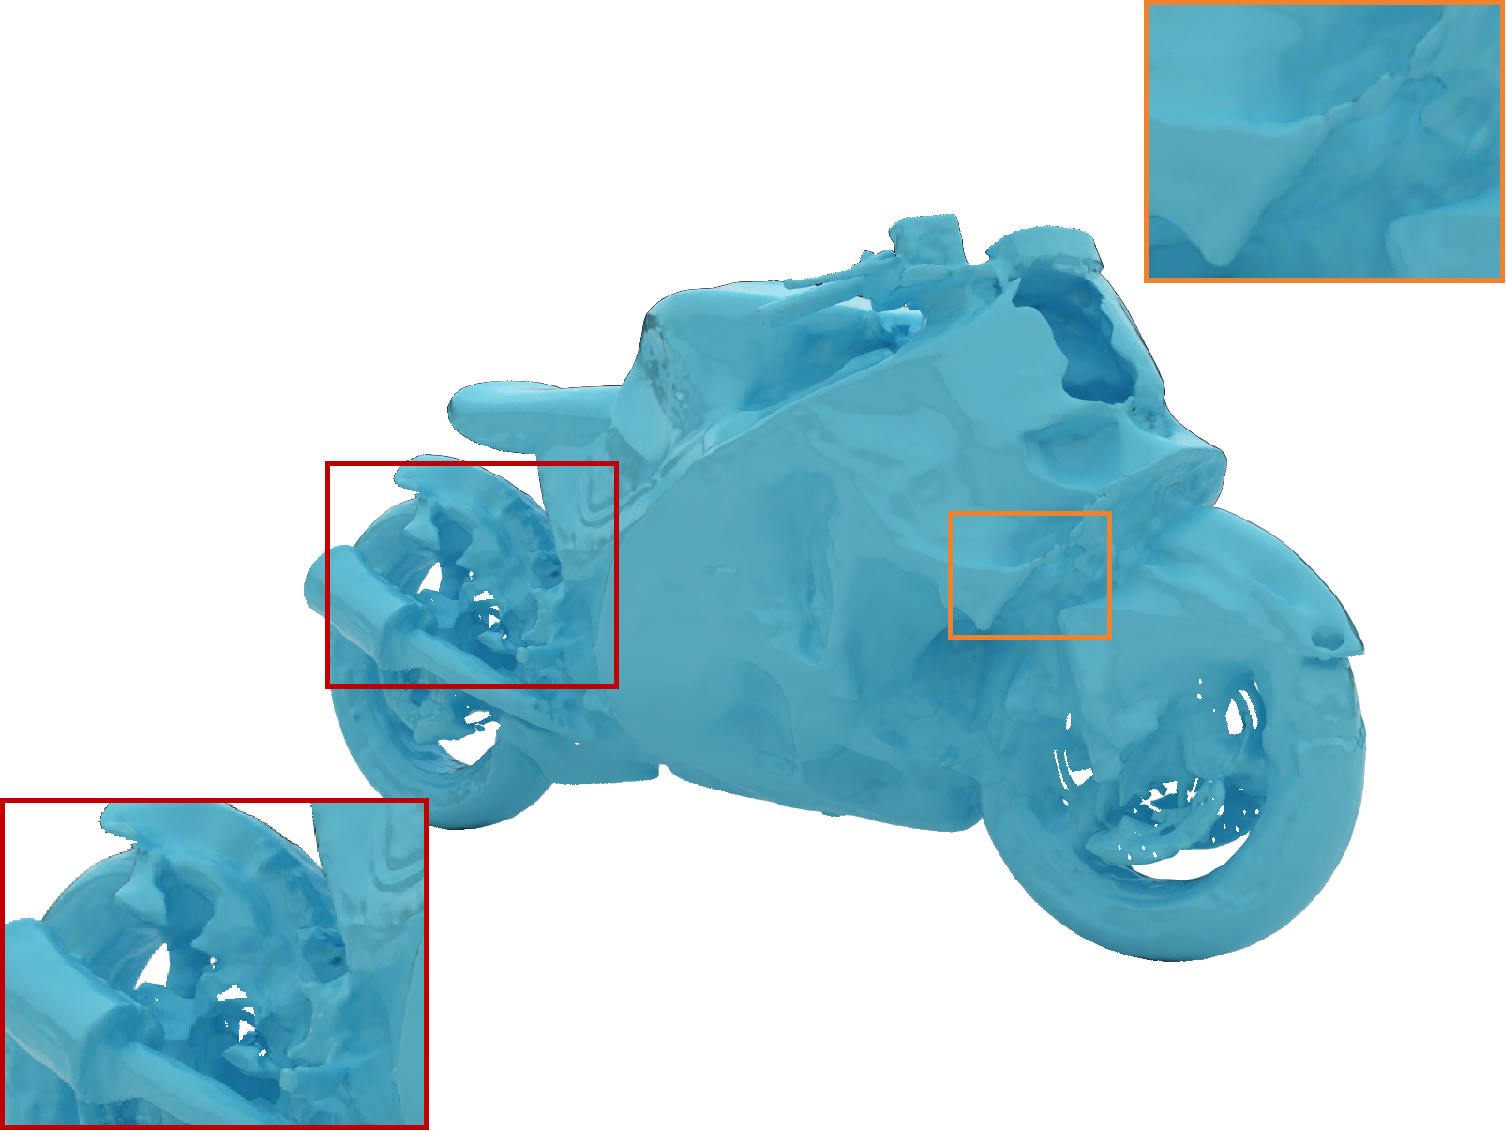} &
        \includegraphics[width=.24\textwidth]{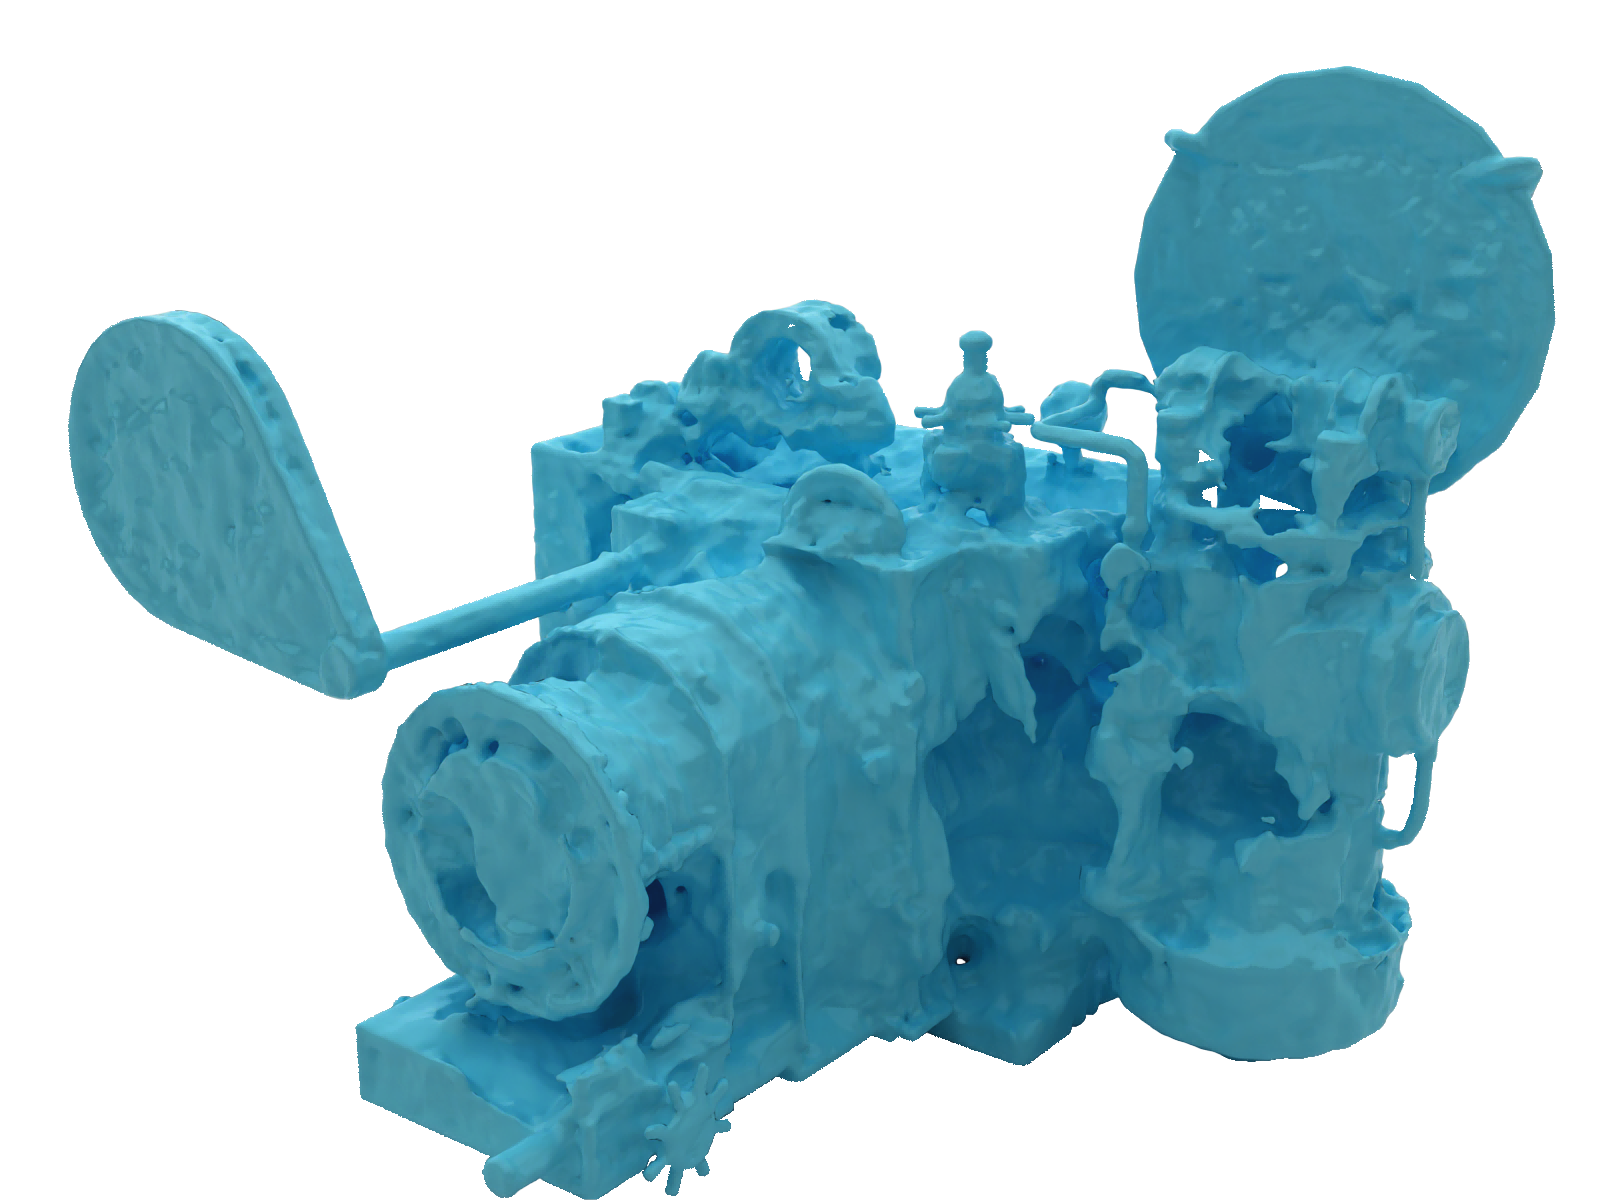} &
        \includegraphics[width=.24\textwidth]{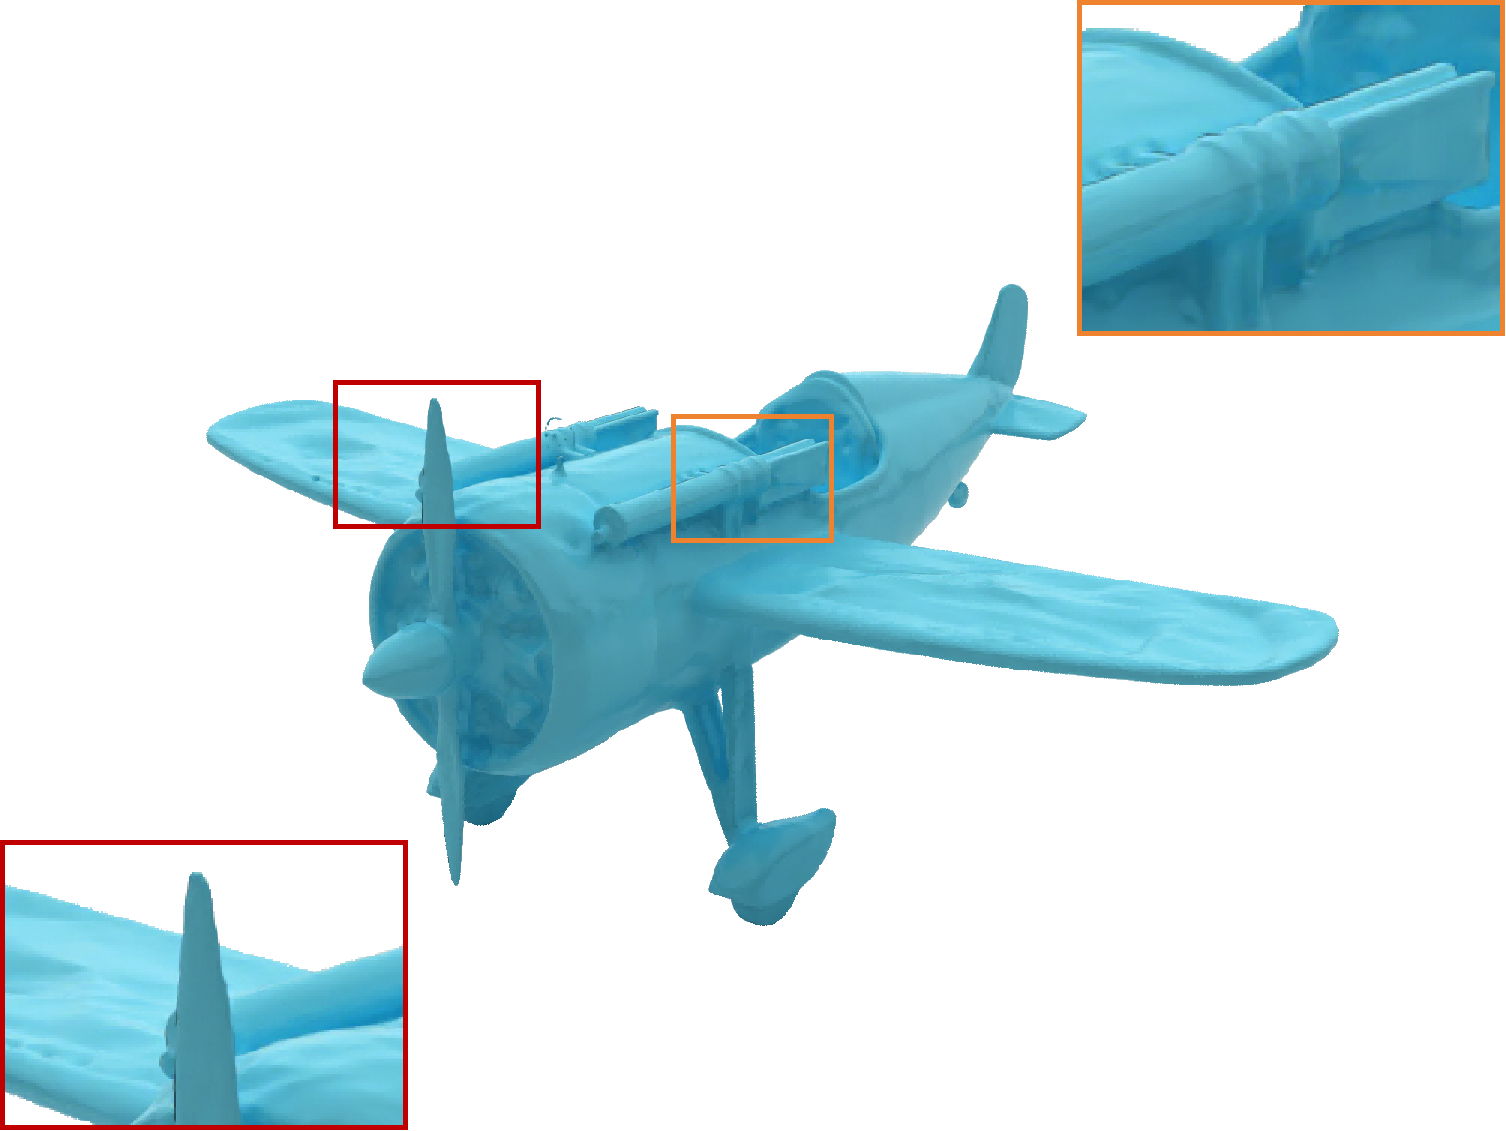} &
        \includegraphics[width=.24\textwidth]{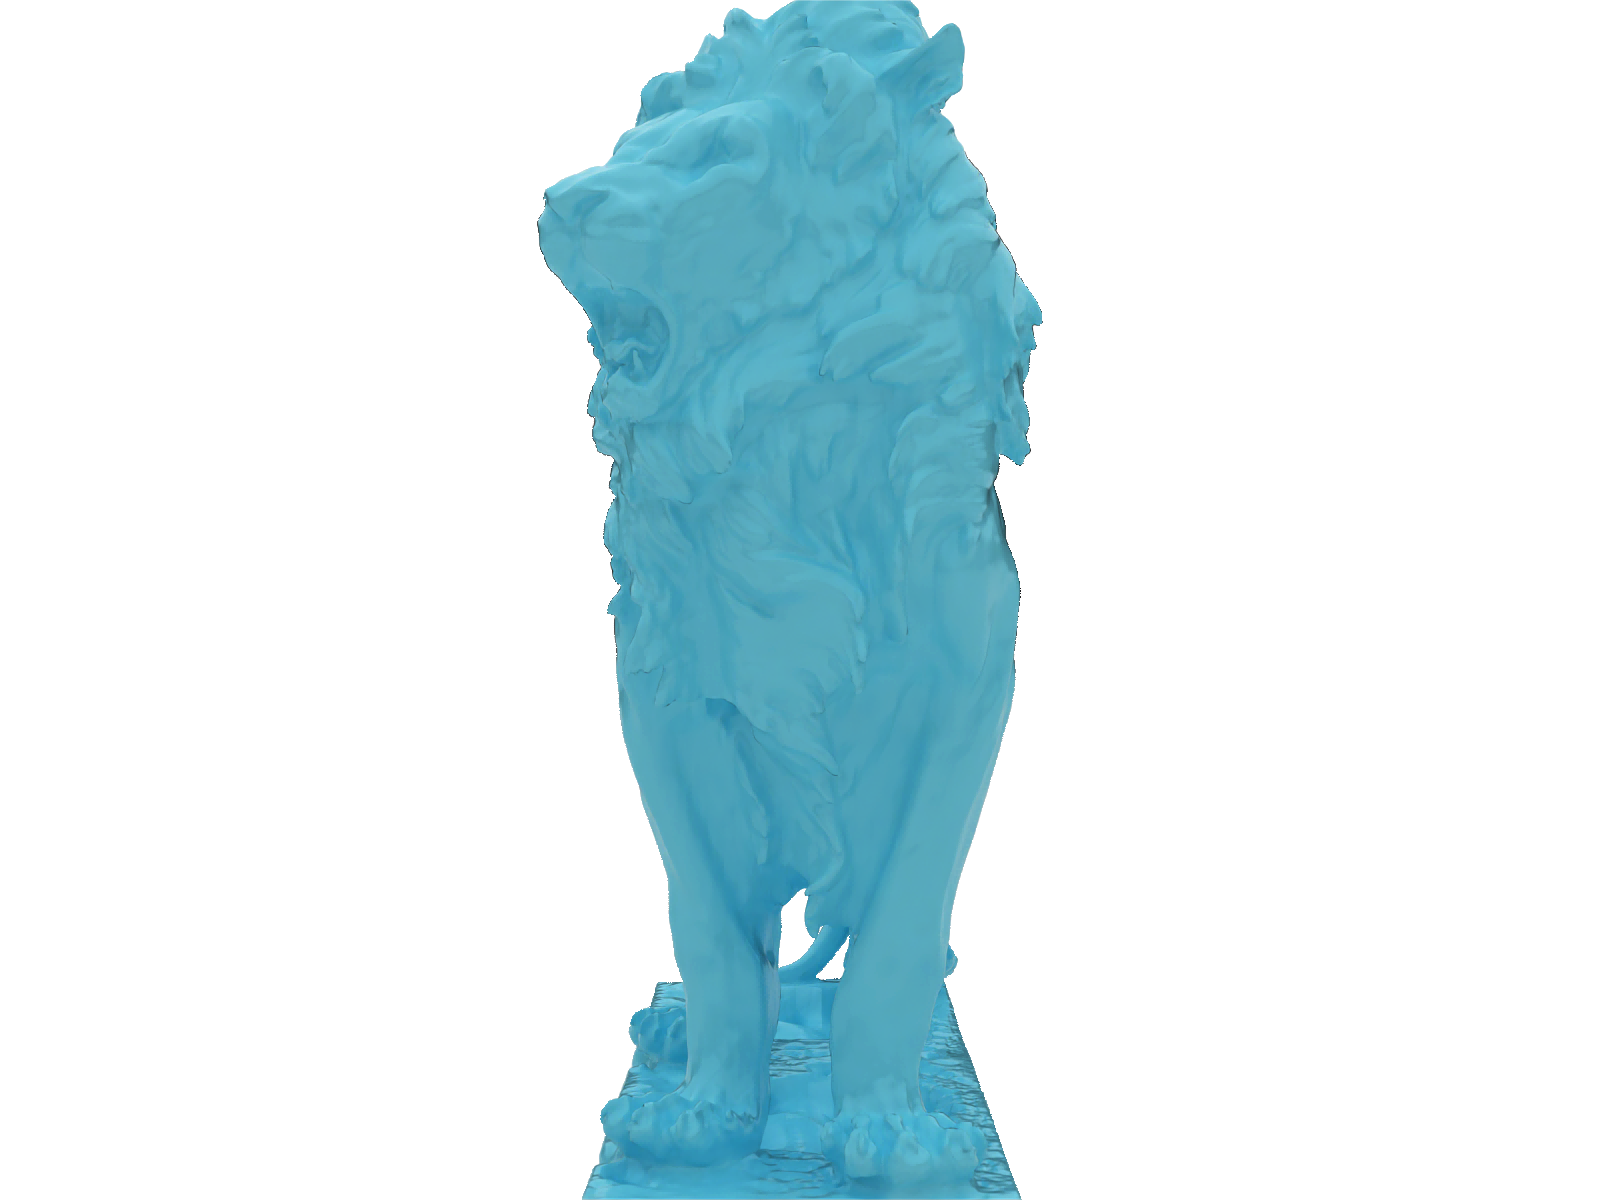} \\

        \rotatebox{90}{\parbox{\imghe}{\centering NeuS2}} &
        \includegraphics[width=.24\textwidth]{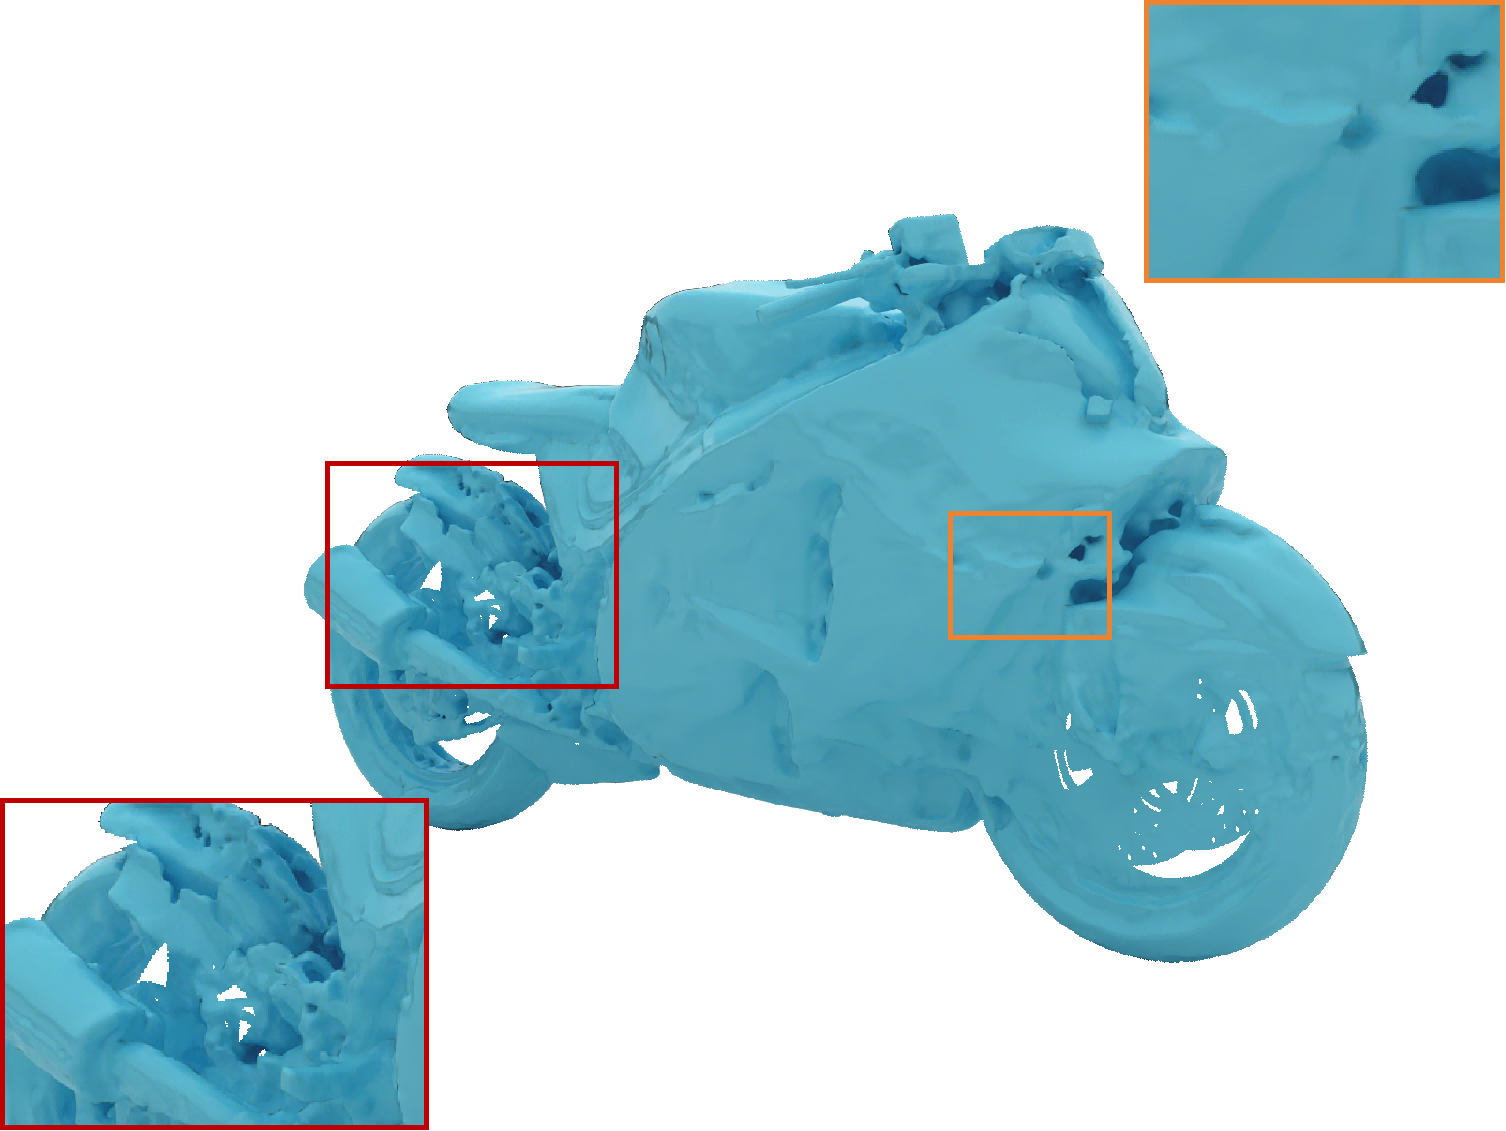} &
        \includegraphics[width=.24\textwidth]{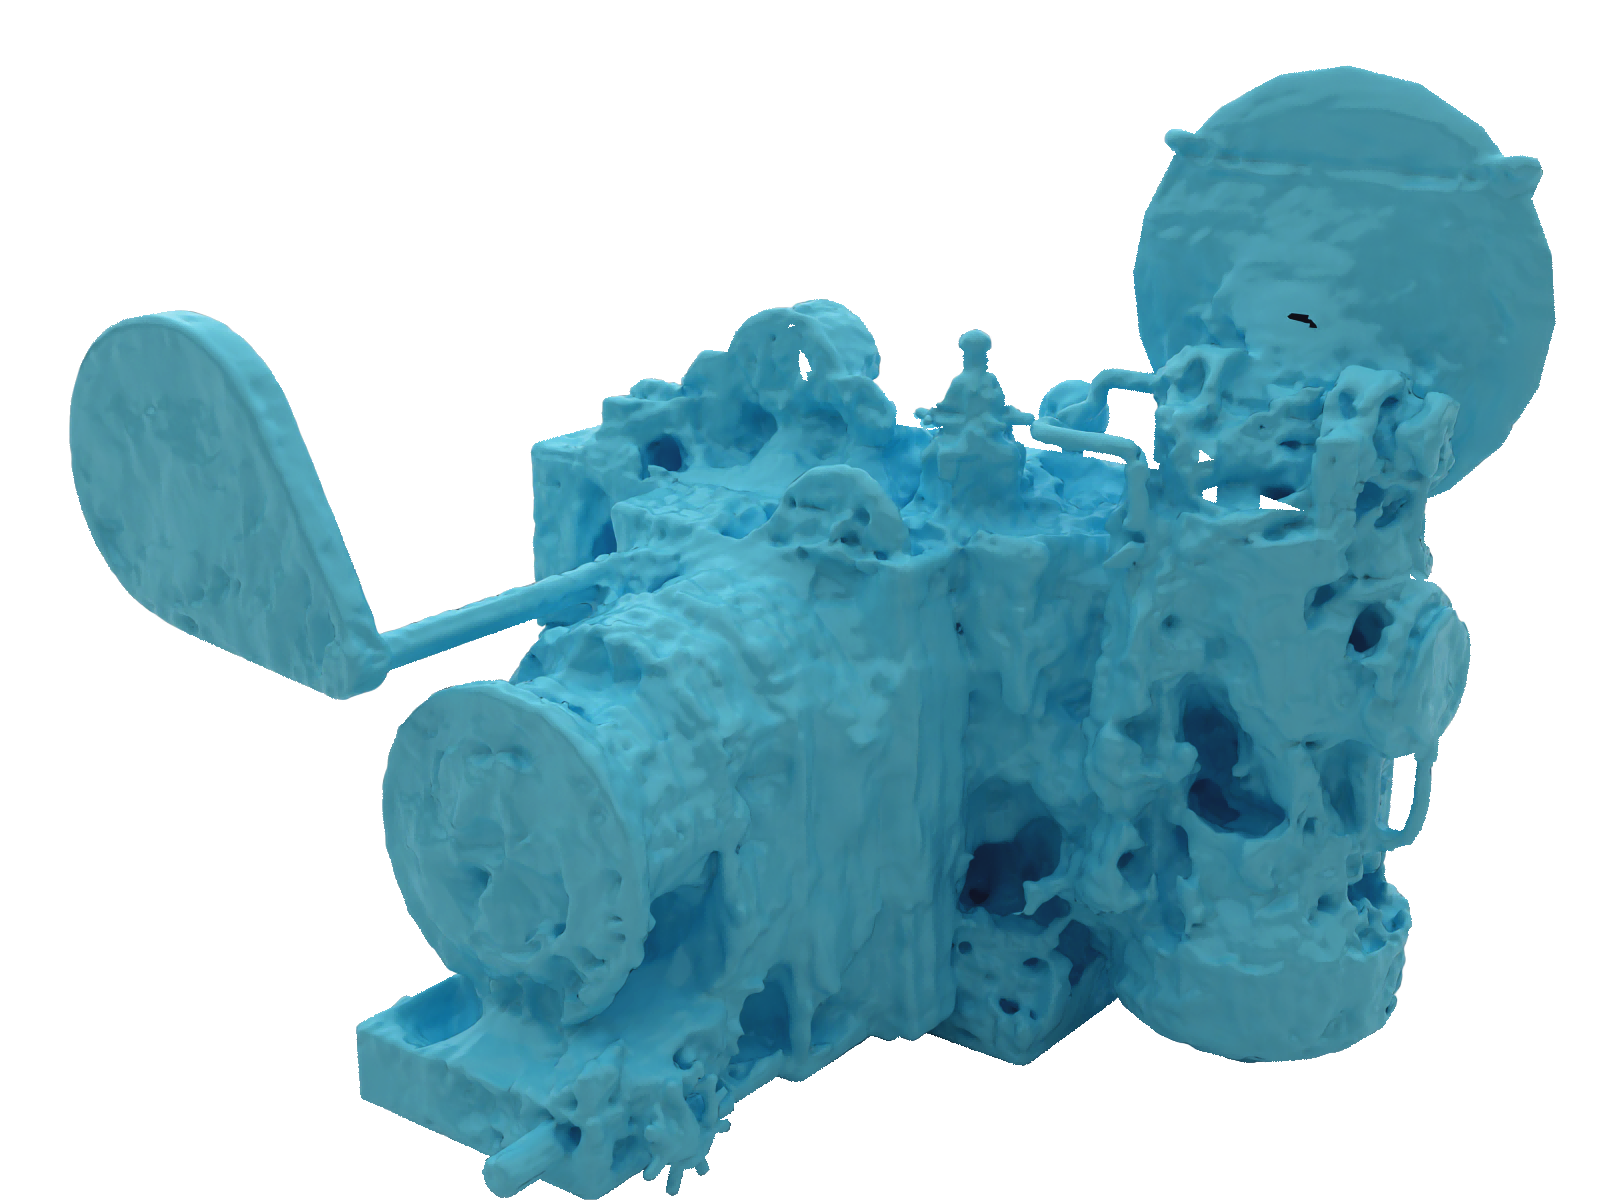} &
        \includegraphics[width=.24\textwidth]{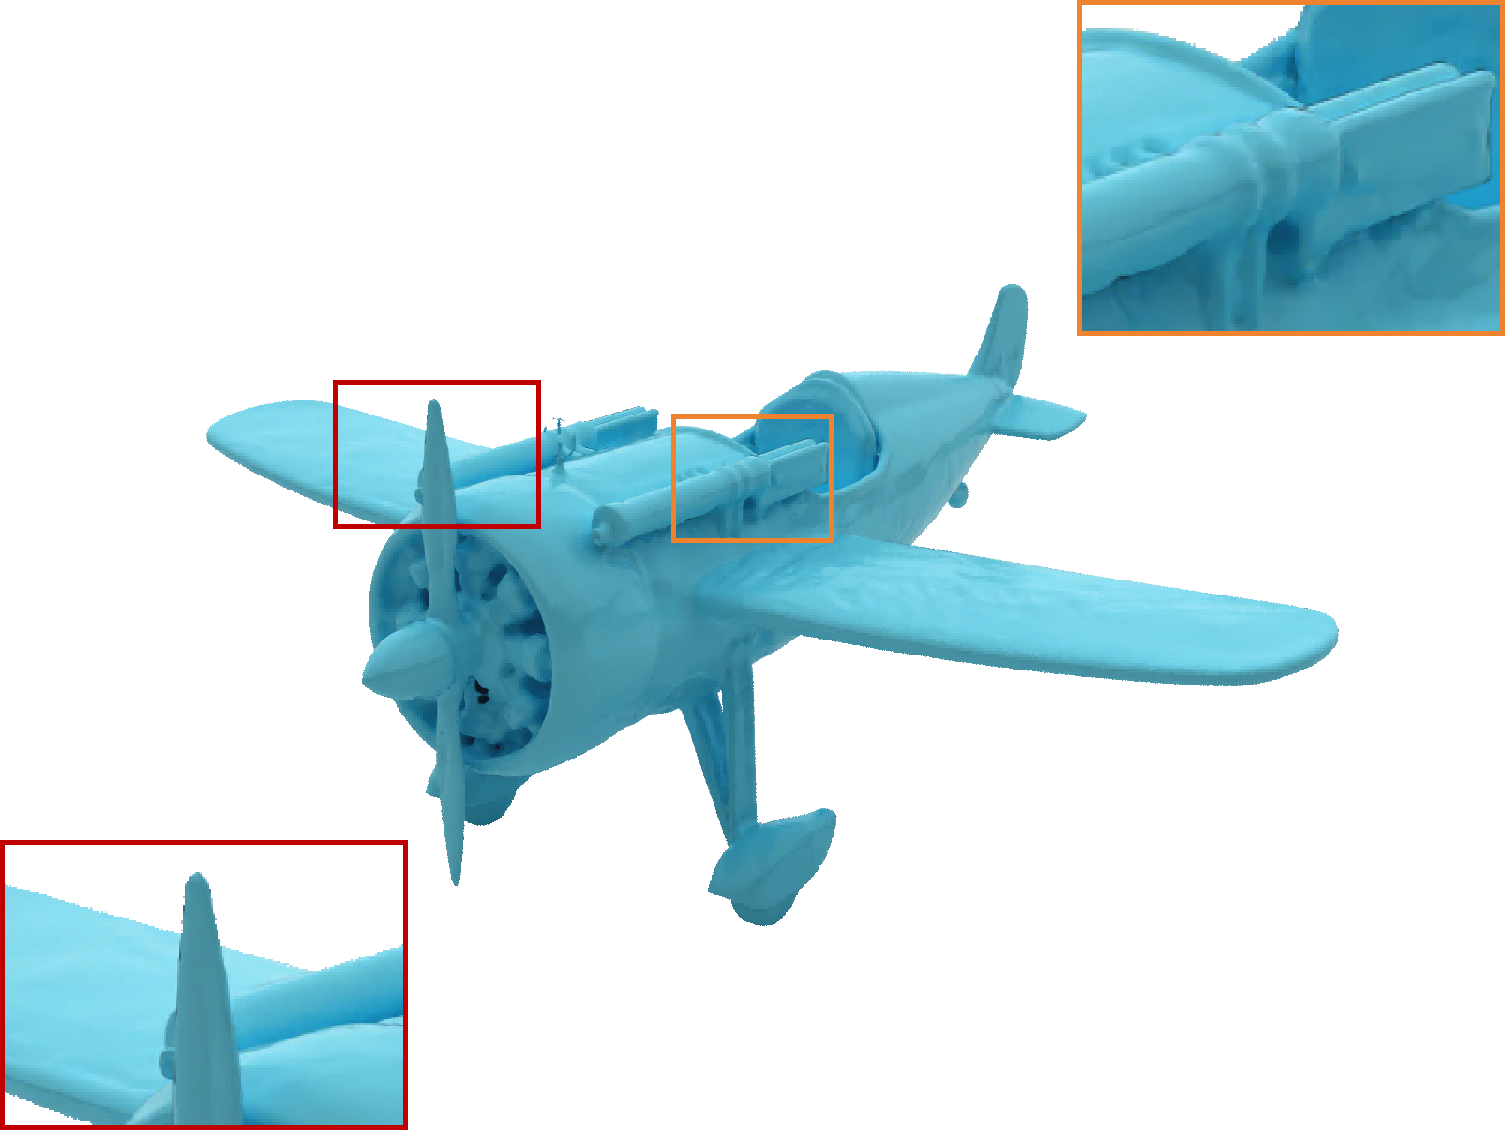} &
        \includegraphics[width=.24\textwidth]{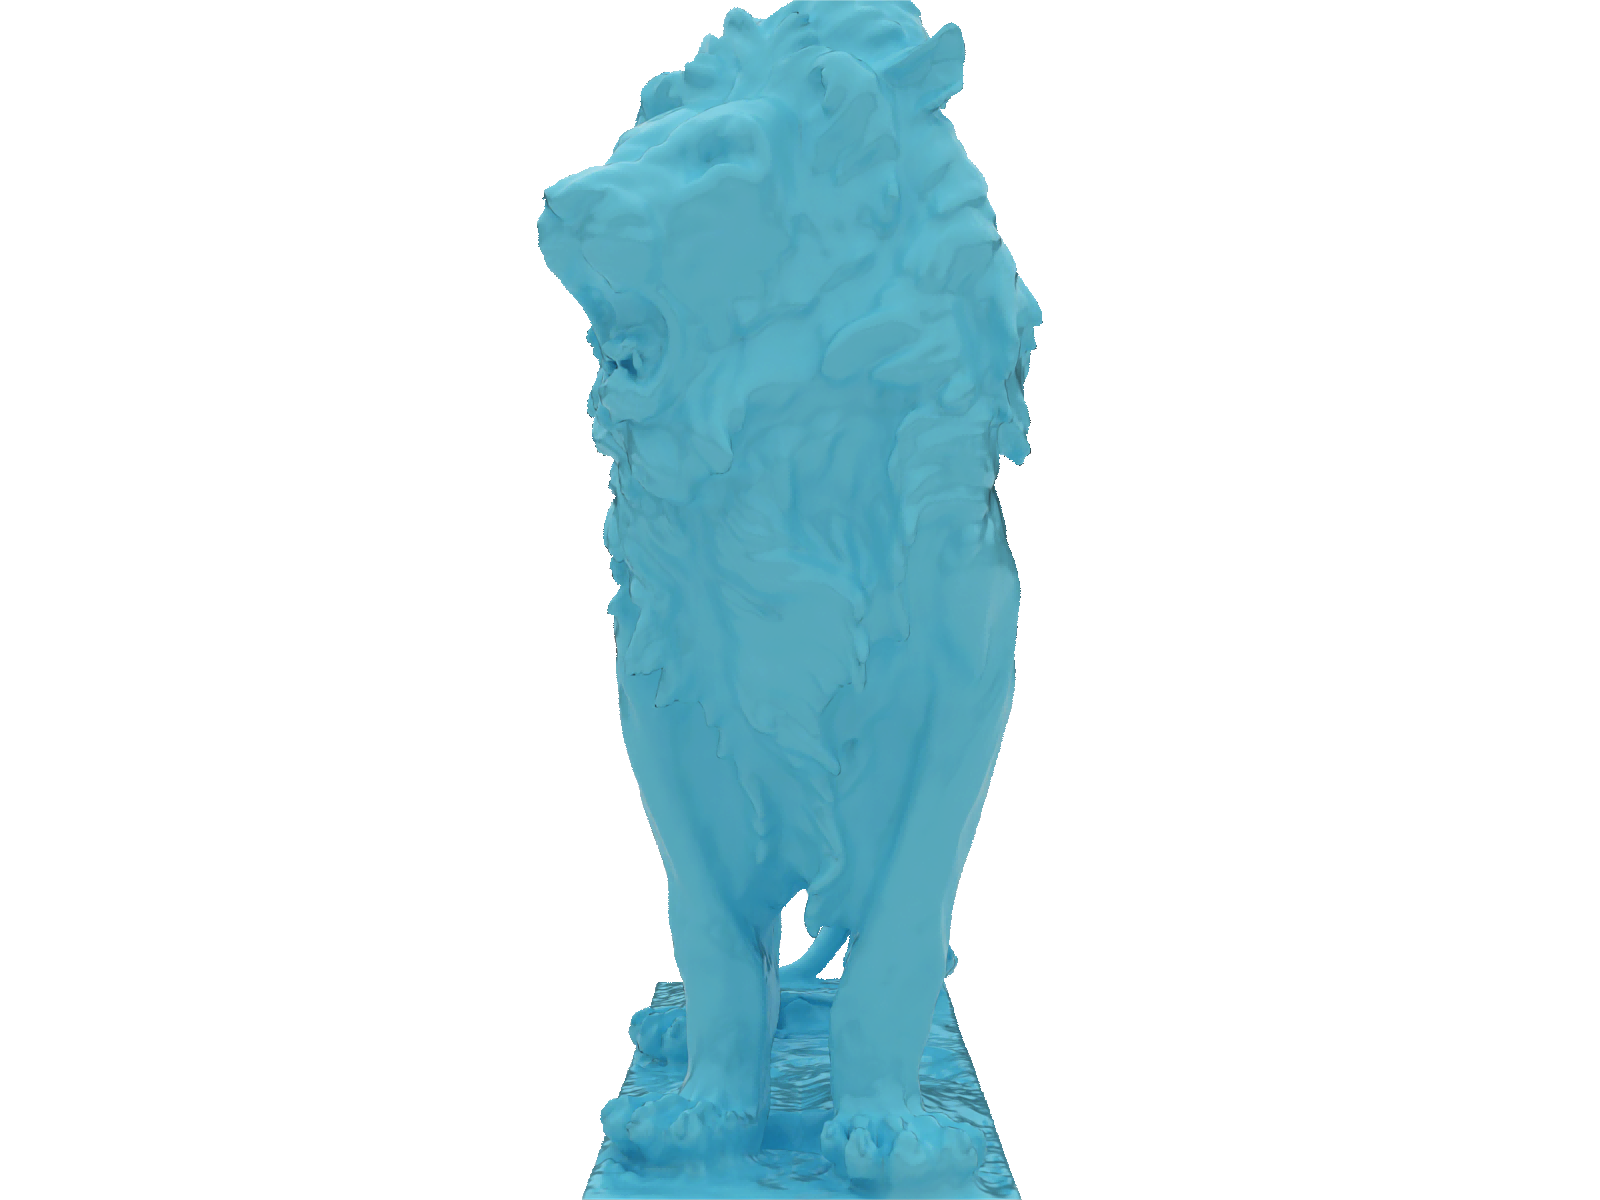} \\
    \end{tabular}
    \caption{\label{fig:neus_appendix-1} \textbf{Additional qualitative 3D reconstruction results on OpenMaterial.}}
    \end{minipage}
\end{figure*}
\begin{figure*}[htb]
    \setlength{\tabcolsep}{1.25pt}
    \setlength{\belowcaptionskip}{-20pt}
    
    \begin{minipage}{\textwidth}
    % Start of centering for all tables
    \begin{tabular}{cc}
    \hspace{1.1cm}
        % Left big image
        \begin{minipage}{.40\textwidth}
            \includegraphics[width=\textwidth]{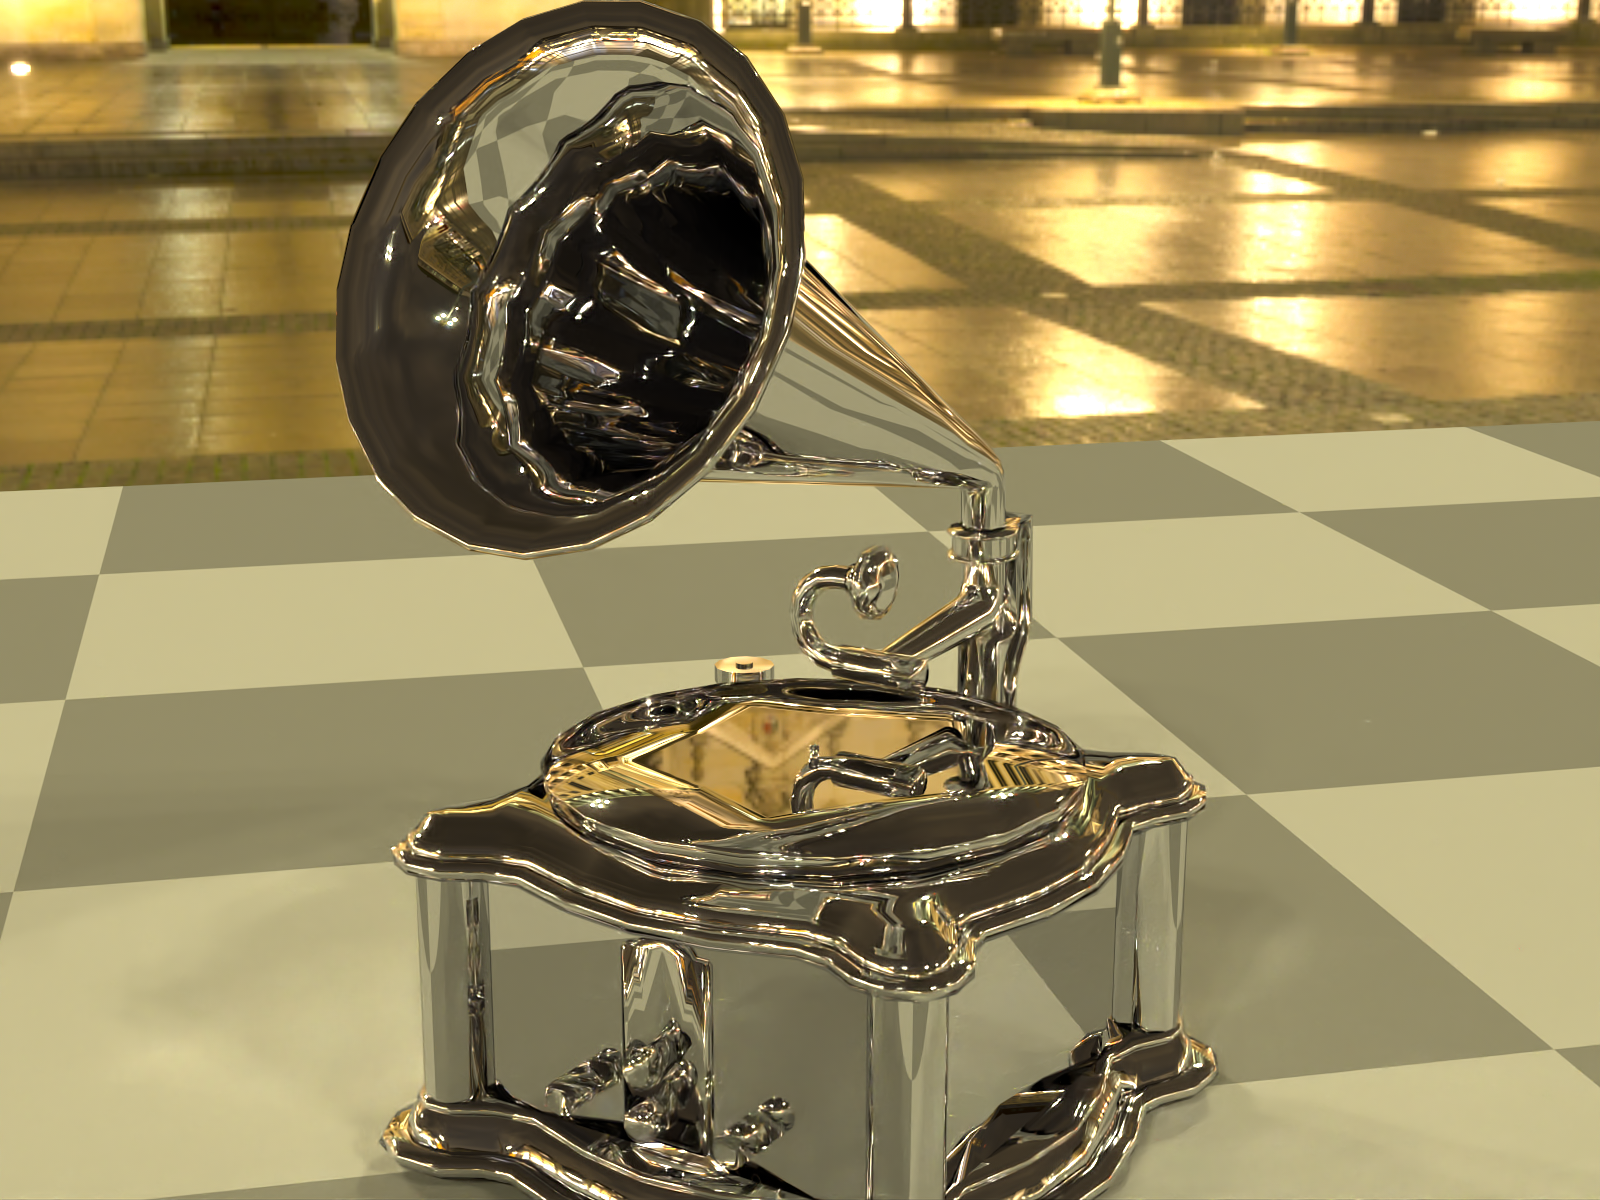}
        \end{minipage} &
        % Right small images in 2x3 grid
        \begin{minipage}{.148\textwidth}
            \begin{tabular}{ccc}
                \includegraphics[width=\textwidth]{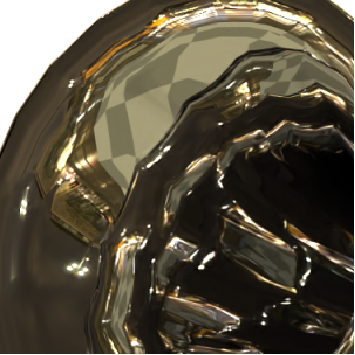} &
                \includegraphics[width=\textwidth]{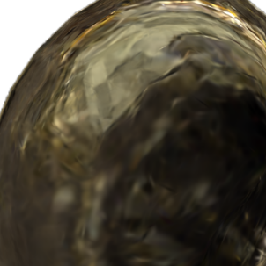} &
                \includegraphics[width=\textwidth]{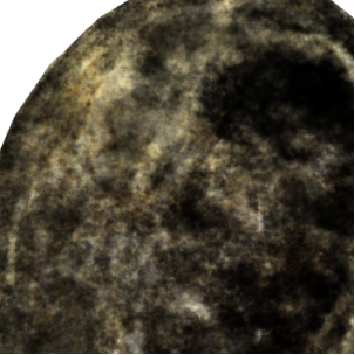} \\
                \includegraphics[width=\textwidth]{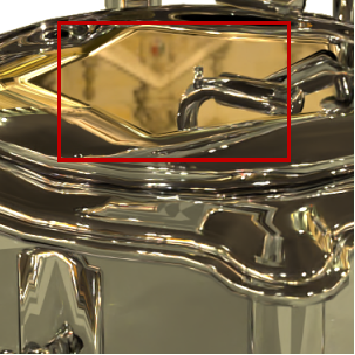} &
                \includegraphics[width=\textwidth]{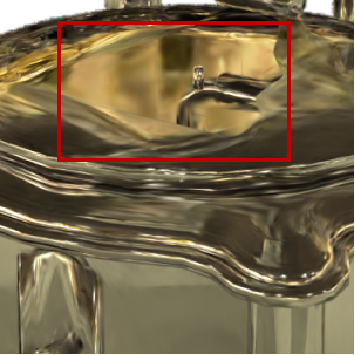} &
                \includegraphics[width=\textwidth]{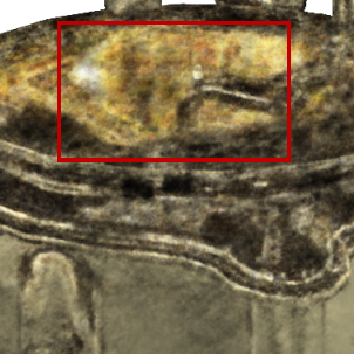} \\
            \end{tabular}
        \end{minipage}
    \end{tabular}

    \begin{tabular}{cc}
    \hspace{1.1cm}
        % Left big image
        \begin{minipage}{.40\textwidth}
            \includegraphics[width=\textwidth]{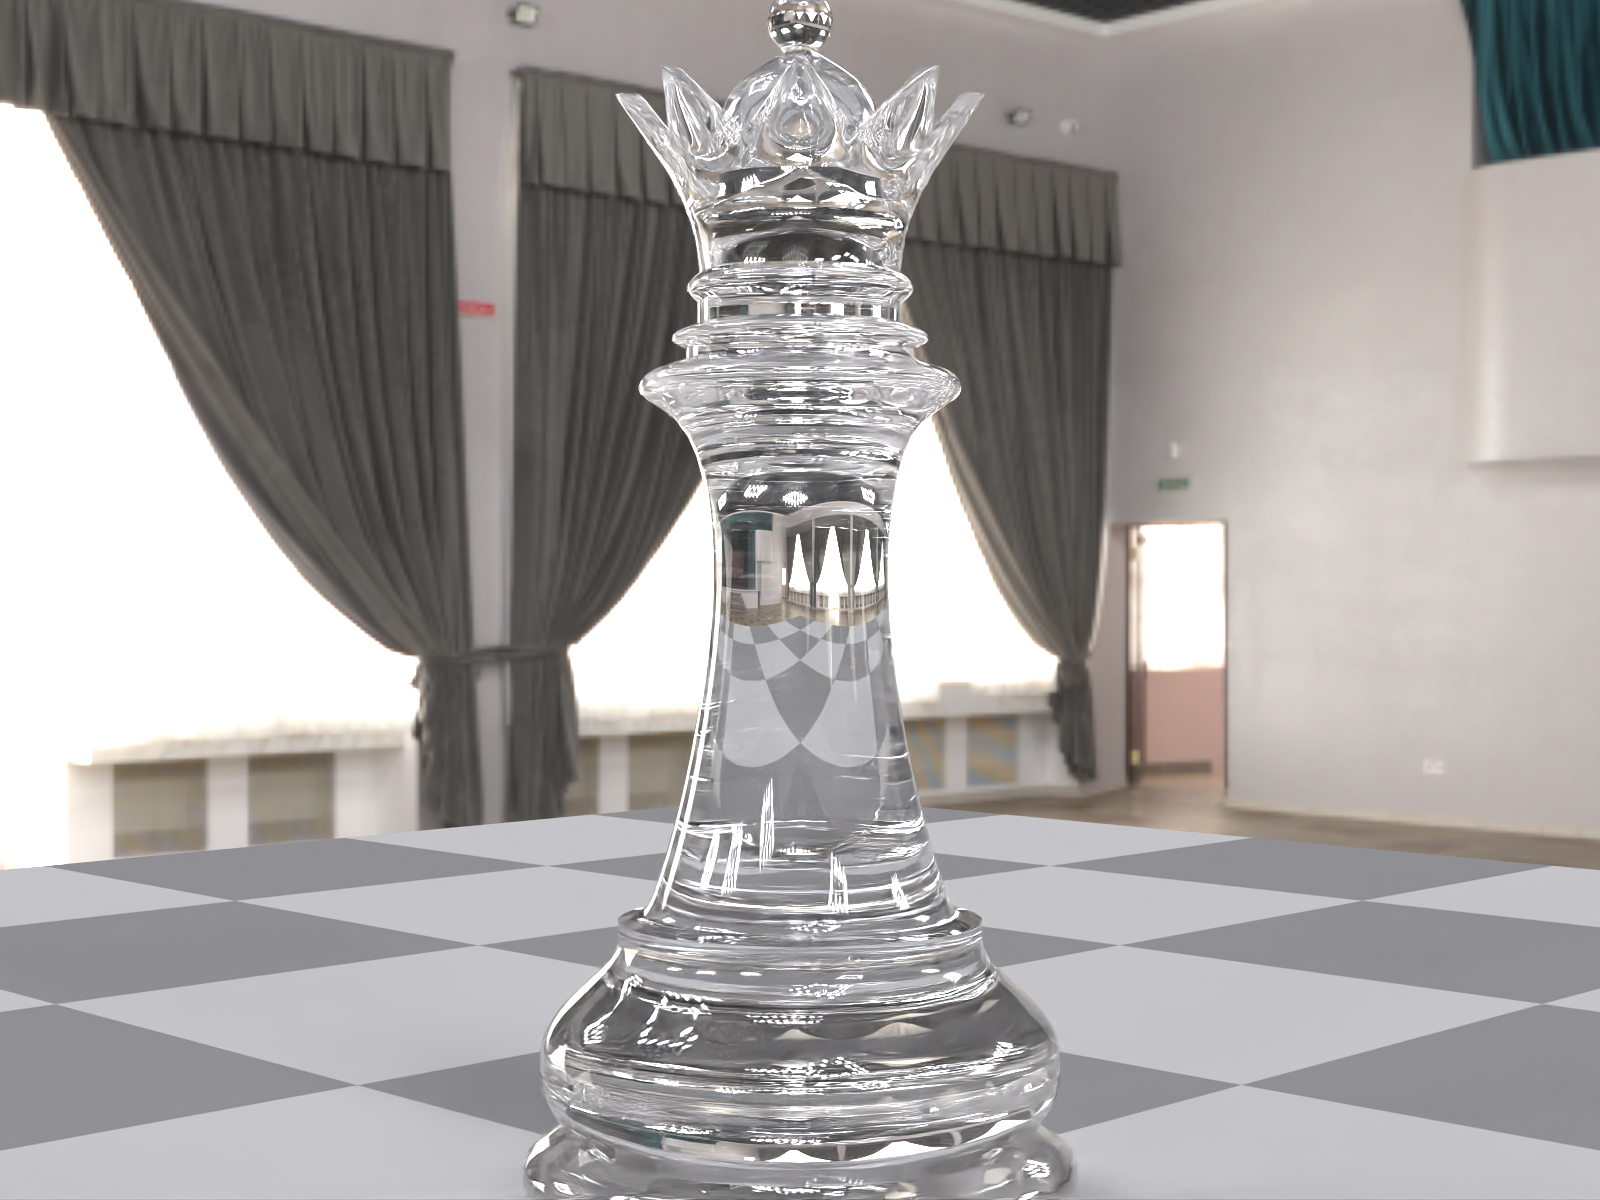}
        \end{minipage} &
        
        % Right small images in 2x3 grid
        \begin{minipage}{.148\textwidth}
            \begin{tabular}{ccc}
                \includegraphics[width=\textwidth]{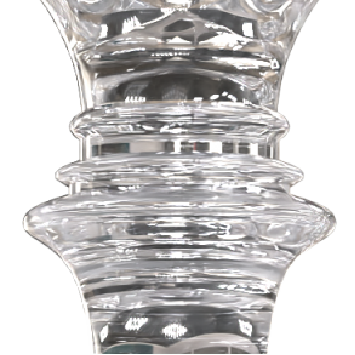} &
                \includegraphics[width=\textwidth]{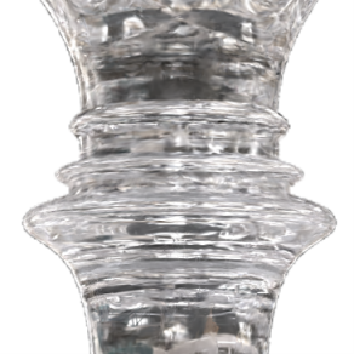} &
                \includegraphics[width=\textwidth]{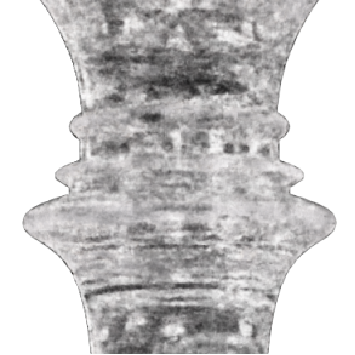} \\
                \includegraphics[width=\textwidth]{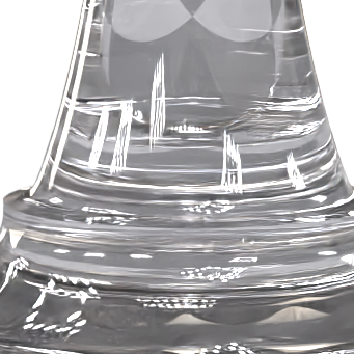} &
                \includegraphics[width=\textwidth]{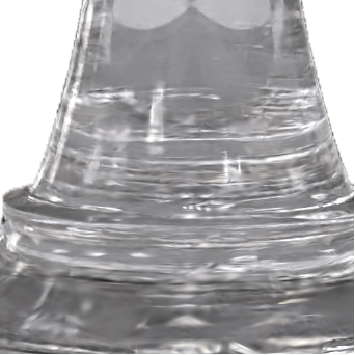} &
                \includegraphics[width=\textwidth]{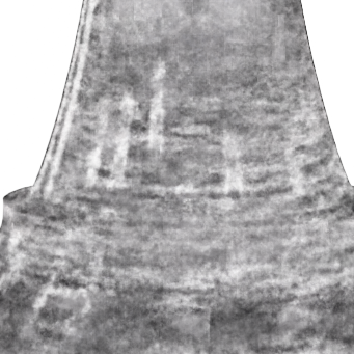} \\
            \end{tabular}
        \end{minipage}
    \end{tabular}

    \begin{tabular}{cc}
    \hspace{1.1cm}
        % Left big image
        \begin{minipage}{.40\textwidth}
            \includegraphics[width=\textwidth]{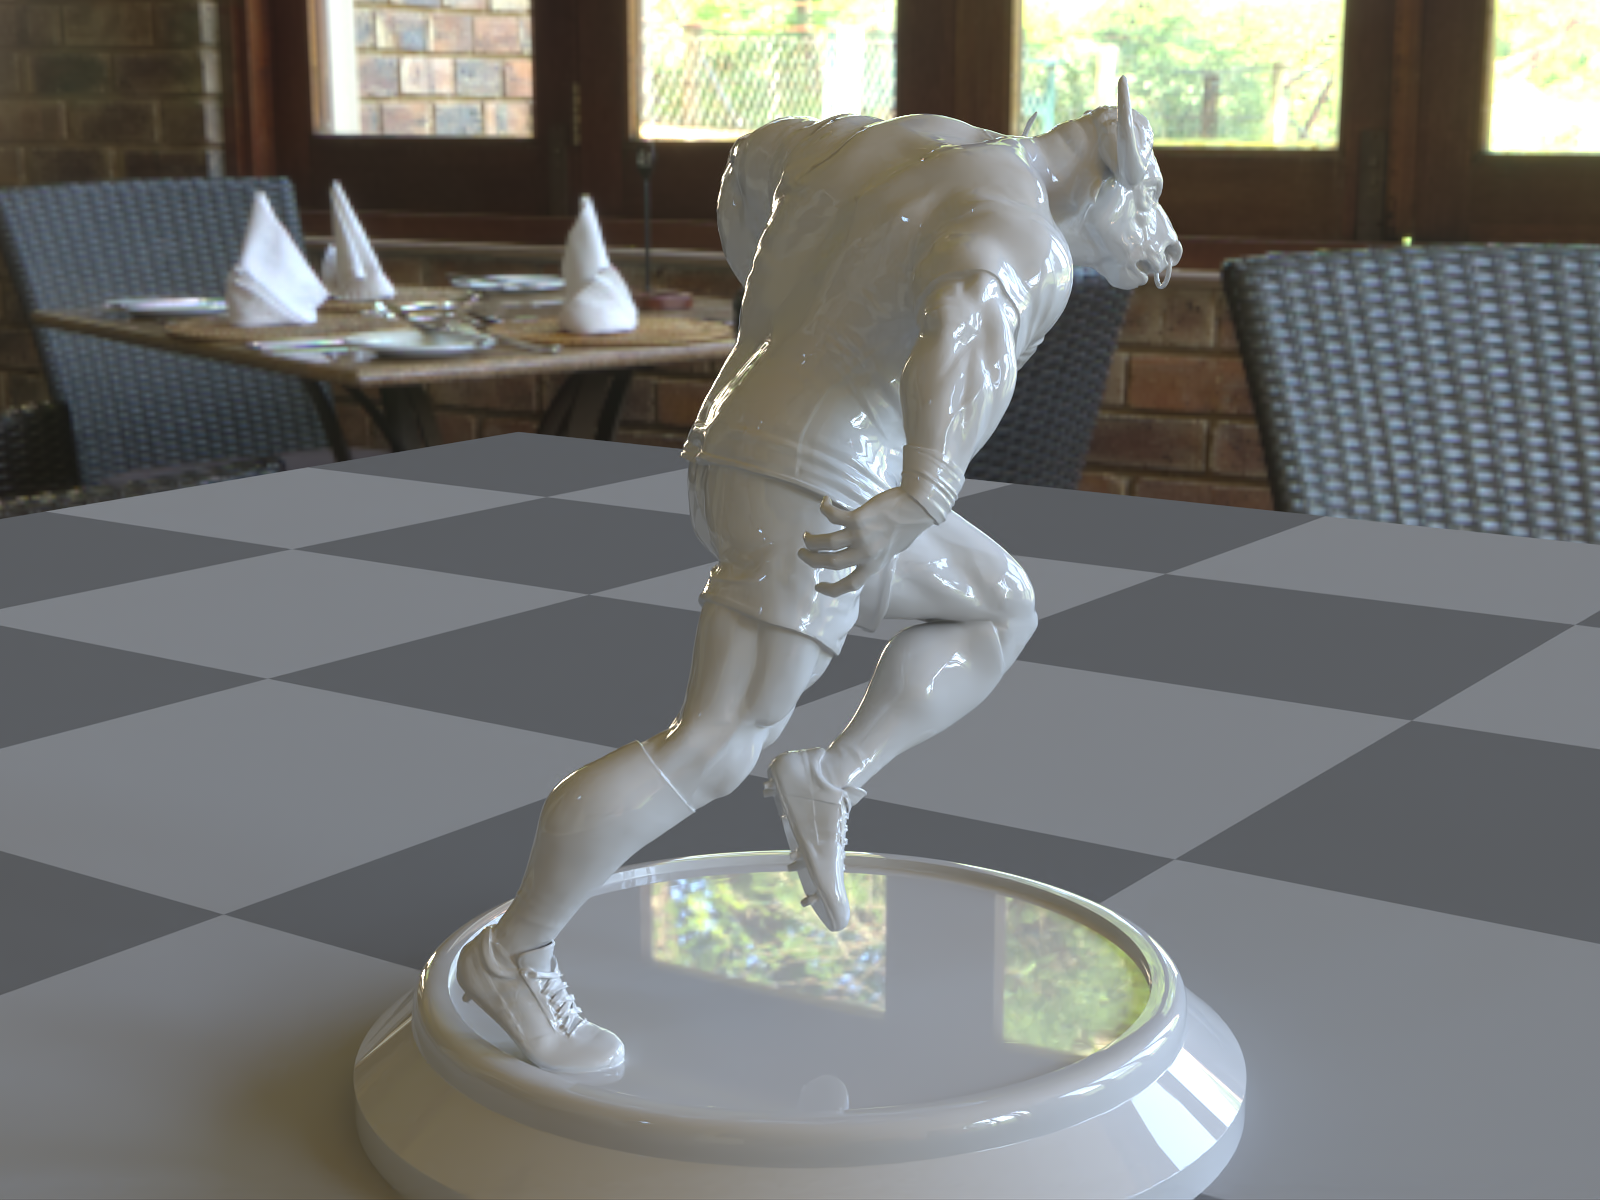}
        \end{minipage} &
        
        % Right small images in 2x3 grid
        \begin{minipage}{.148\textwidth}
            \begin{tabular}{ccc}
                \includegraphics[width=\textwidth]{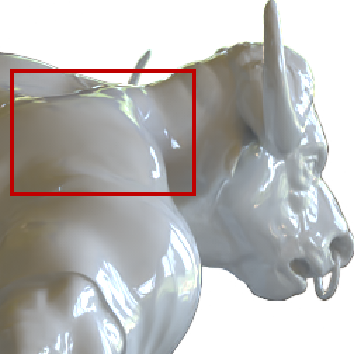} &
                \includegraphics[width=\textwidth]{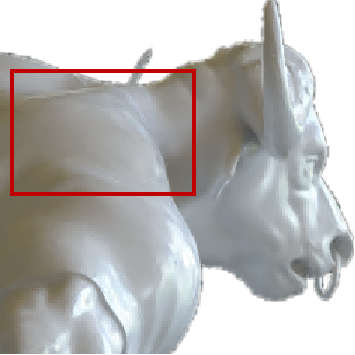} &
                \includegraphics[width=\textwidth]{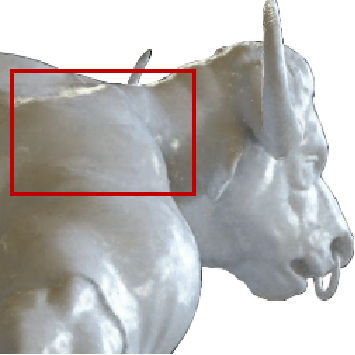} \\
                \includegraphics[width=\textwidth]{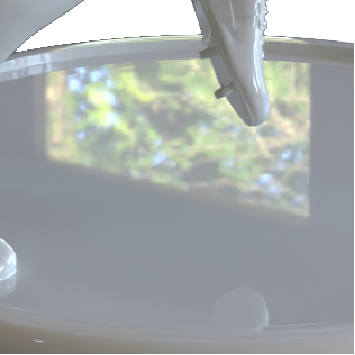} &
                \includegraphics[width=\textwidth]{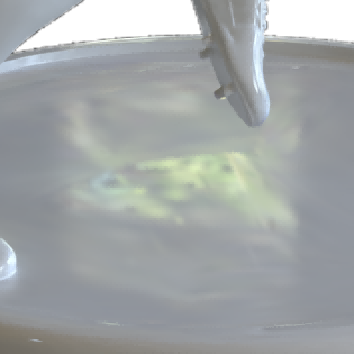} &
                \includegraphics[width=\textwidth]{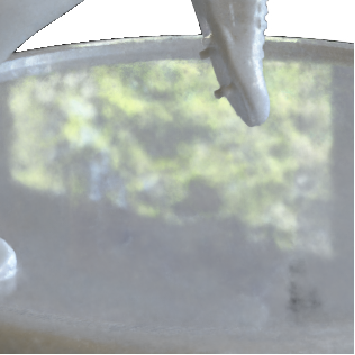} \\
            \end{tabular}
        \end{minipage}
    \end{tabular}

    \begin{tabular}{cc}
    \hspace{1.1cm}
        % Left big image
        \begin{minipage}{.40\textwidth}
            \includegraphics[width=\textwidth]{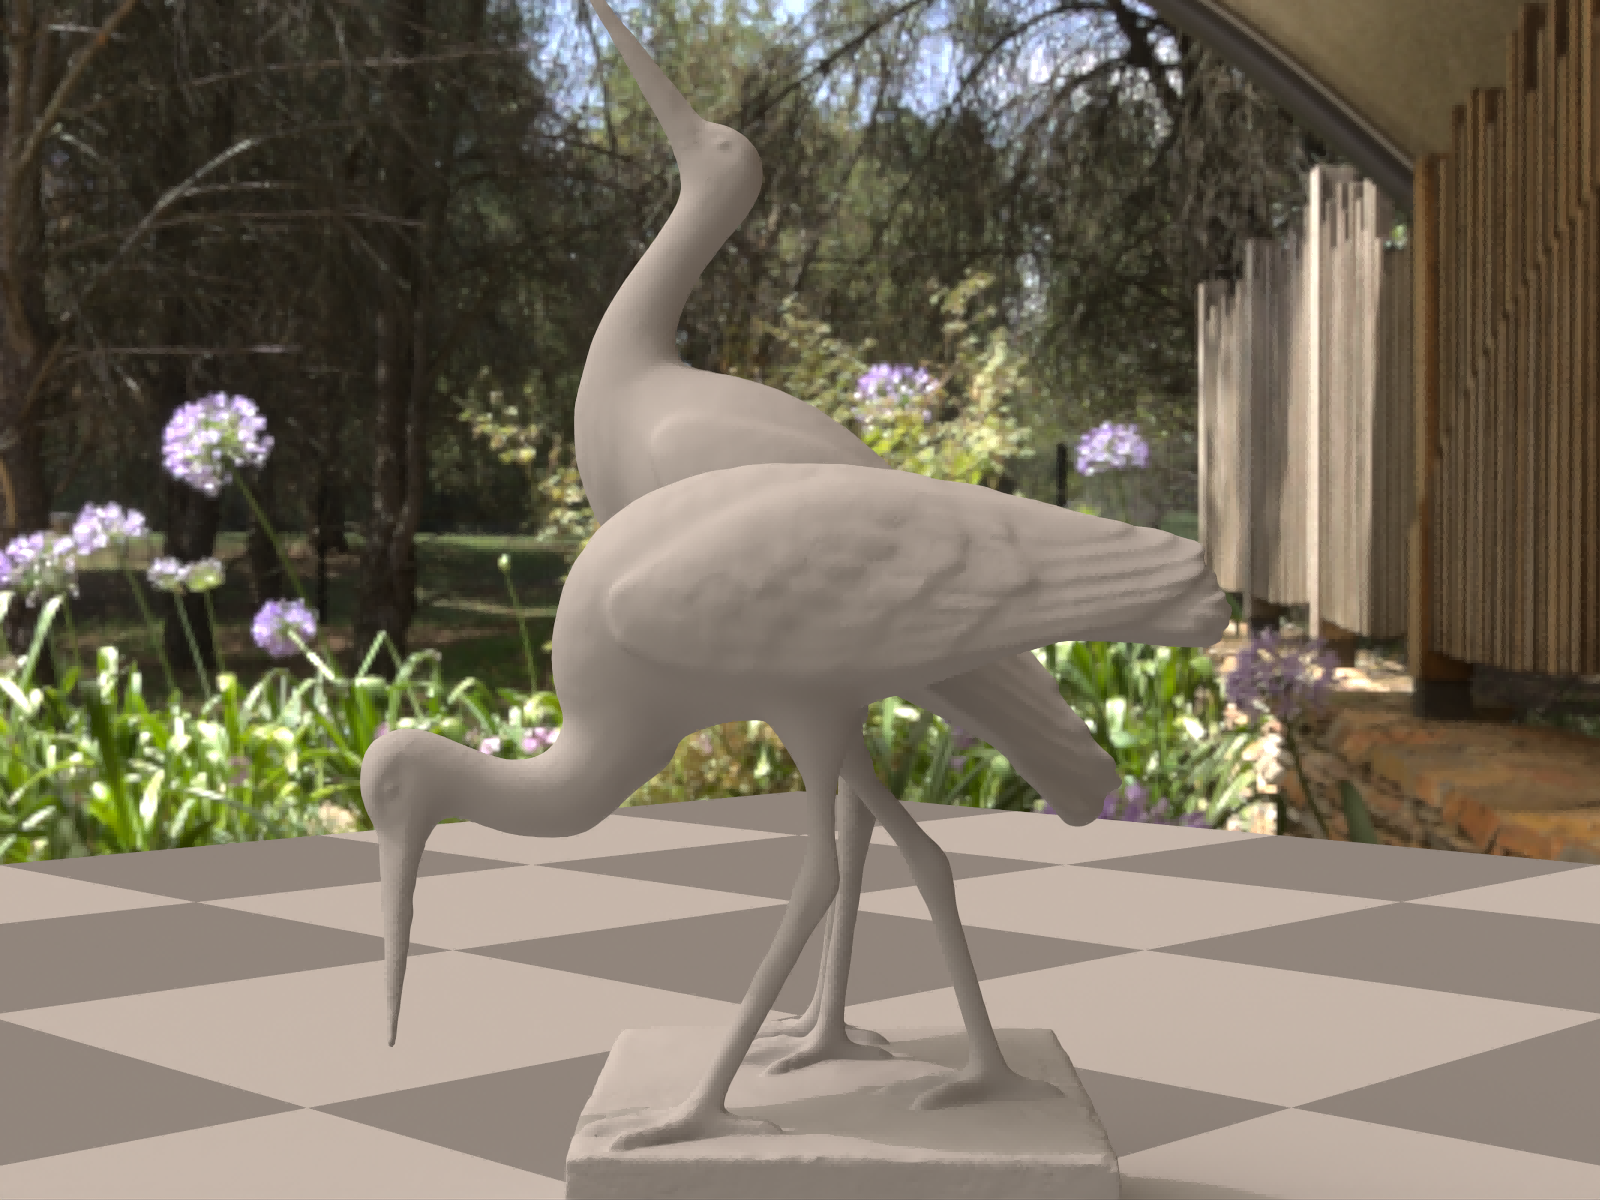}
        \end{minipage} &
        
        % Right small images in 2x3 grid
        \begin{minipage}{.148\textwidth}
            \begin{tabular}{ccc}
                \includegraphics[width=\textwidth]{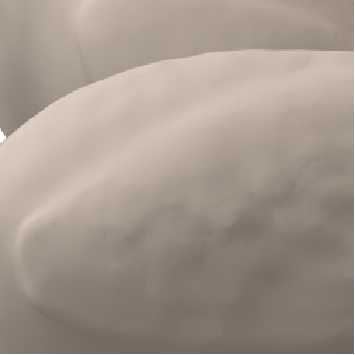} &
                \includegraphics[width=\textwidth]{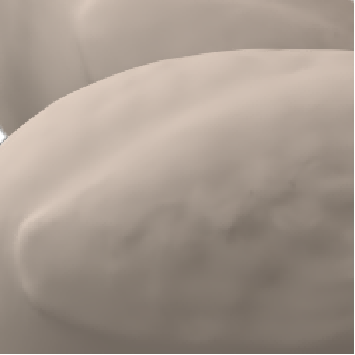} &
                \includegraphics[width=\textwidth]{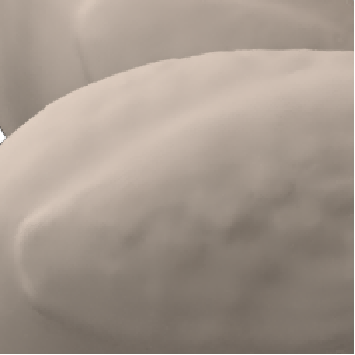} \\
                \includegraphics[width=\textwidth]{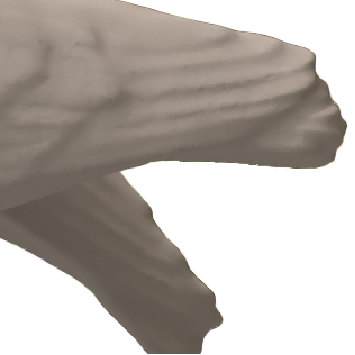} &
                \includegraphics[width=\textwidth]{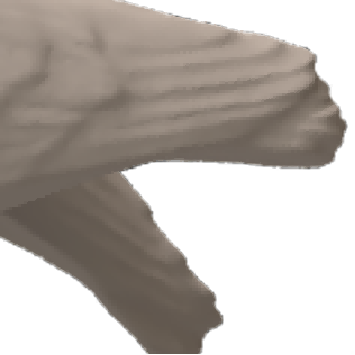} &
                \includegraphics[width=\textwidth]{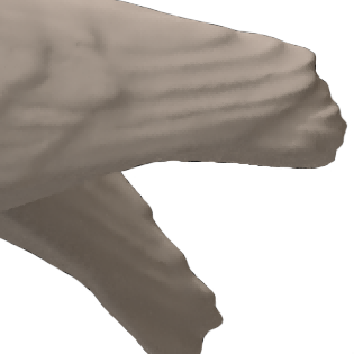} \\
            \end{tabular}
        \end{minipage}
    \end{tabular}
    \end{minipage}
    \caption{\label{fig:nerf_appendix} \textbf{Qualitative result on the novel view synthesis task.} From top to bottom: Conductor, Dielectric, Plastic, Diffuse. From left to right: GT (global), GT (local), PGSR, Instant-NGP.}
\end{figure*}

\FloatBarrier

\section{Dataset Responsibility and Accessibility}

\textbf{Author statement.}
The authors of this submission bear all responsibility in the event of any rights violations or other legal issues. We confirm that the dataset is distributed under the CC BY-NC 4.0 DEED license, allowing free use with proper attribution.

% \textbf{Long-term preservation.}
% To ensure the long-term preservation of the dataset, we have opted to host it on Hugging Face, a choice that underscores our commitment to data longevity and reliability. We follow Hugging Face's standarization to arrange our dataset, which allows users to conveniently download and explore datasets through a python API.
% We enable the dataset version control, which supports users in accessing specific versions of the data, ensuring the reproducibility of experimental results.
\vspace{.3cm}
\noindent\textbf{Hosting, licensing, and maintenance plan.}
The dataset will be hosted on Hugging Face, which guarantees reliable access and data integrity. We have enabled the feedback system on the repository for users to report issues and suggest improvements. The dataset as a whole is licensed under the CC BY-NC 4.0 DEED license, ensuring it can be freely used with proper attribution. However, individual 3D object shapes within the dataset are subject to different licenses. For more detail on each object's specific license, please refer to the Objaverse~\cite{Deitke23} documentation.
